# Supplementary material for: Describing Deferred Acceptance and Strategyproofness to Participants: Experimental Analysis
Source: arXiv:2409.18166 ancillary file (2024-09-26)
Supplement: Supplementary file 2 [file full-screenshot-appendix.pdf]

## D.1.1 Welcome Page (Cornell)

# Welcome

This study takes around **50 minutes** to complete.

In this study you will learn about a game, and play the game.

For completing the study, you will earn **\$17.00**. Your total earnings can increase in two ways:

1. **Earnings from playing**, which can be up to **\$9.90**: You will play a lot of rounds of the game, and each round earns you money depending on your actions and luck, as you will learn shortly. Make sure you play the game thoughtfully!
2. An **Understanding Bonus**, which can be up to **\$4.50**: You will learn about the game in different parts of this study and we will ask you many understanding questions. At the end of the study, each question you answer correctly on the **first attempt** will be counted for your Understanding Bonus.
  - If you answered all questions correctly on the first attempt, you will earn the full Understanding Bonus of \$4.50.
  - If you answered some fraction of the questions correctly on the first attempt, you will earn this fraction of the Understanding Bonus. For example, if you answered 80% of the questions correctly on the first attempt, you will earn 80% times \$4.50 = \$3.60.
  - Unless stated otherwise, you will **not** earn money for questions that you only answered correctly after more than one attempt.

Make sure you pay close attention to the game instructions to earn this money!

**It is crucial for our purposes that you complete the study** once you start it. Making some mistakes in understanding questions along the way is perfectly normal. Our main objective is that you try your best to understand and play the game.

If you feel that you currently lack sufficient time or mental resources for this study, we kindly request that you stop your participation now, and quietly inform the lab staff in the room that you decided to leave. No questions will be asked.

Important notes:

- Remember that your Understanding Bonus will increase the more questions you answer correctly, and your earnings from playing the game depend on your understanding of it.
- Remember that every question you are asked or a game round you play is a completely new opportunity to increase your earnings, regardless of your previous outcomes.

## Consent

Thank you for participating in this study! Your participation is voluntary, and is greatly appreciated. We anticipate that your participation in this study presents no greater risk than everyday internet use. We are committed to protecting your privacy. After validating that your response qualifies for payment, your answers will remain anonymous and will only take part in aggregate statistical analyses. You may withdraw from the study at any time if you feel uncomfortable answering some questions.

It is very important that you complete this study on your own and with adequate effort.

## Additional Information

The main researchers conducting this study are Ori Heffetz, a professor at Cornell University, and Guy Ishai. If you have any questions or concerns regarding your rights as a subject in this study, you may contact the Institutional Review Board (IRB) for Human Participants at 607-255-5138 or access their website at <http://www.irb.cornell.edu>. You may also anonymously report your concerns or complaints through Ethicspoint online at [www.hotline.cornell.edu](http://www.hotline.cornell.edu) or by calling toll free at 1-866-293-3077.

Ethicspoint is an independent organization that serves as a liaison between the University and the person bringing the complaint to ensure anonymity.

Confirmation:

- Yes, I agree to participate in the study  
 No, I do not agree to participate in the study

Please enter your Cornell email address:

Next

## D.1.2 Welcome Page (Prolific)

# Welcome

This study takes around **70 minutes** to complete. Everything you will earn in the study is actual money.

Please **use Google Chrome** and **maximize the browser's window** on your screen to view the study properly.

In this study you will learn about a game, and play the game.

For completing the study, you will earn **£7.00**. Your total earnings can increase in two ways:

1. **Earnings from playing**, which can be up to **£9.90**: You will play a lot of rounds of the game, and each round earns you money depending on your actions and luck, as you will learn shortly. Make sure you play the game thoughtfully!
2. An **Understanding Bonus**, which can be up to **£4.50**: You will learn about the game in different parts of this study and we will ask you many understanding questions. At the end of the study, each question you answer correctly on the **first attempt** will be counted for your Understanding Bonus.
  - If you answered all questions correctly on the first attempt, you will earn the full Understanding Bonus of £4.50.
  - If you answered some fraction of the questions correctly on the first attempt, you will earn this fraction of the Understanding Bonus. For example, if you answered 80% of the questions correctly on the first attempt, you will earn 80% times £4.50 = £3.60.
  - Unless stated otherwise, you will **not** earn money for questions that you only answered correctly after more than one attempt.

Make sure you pay close attention to the game instructions to earn this money!

**It is crucial for our purposes that you complete the study** once you start it. Making some mistakes in understanding questions along the way is perfectly normal. Our main objective is that you try your best to understand and play the game.

If you feel that you currently lack sufficient time or mental resources for this study, we kindly request that you return the submission now.

Important notes:

- Do not worry about rejection. We will **not reject your submission** if you do not answer understanding questions correctly. Instead, your Understanding Bonus will increase the more questions you answer correctly, and your earnings from playing the game depend on your understanding of it.
- Remember that every question you are asked or a game round you play is a completely new opportunity to increase your earnings, regardless of your previous outcomes.

## Consent

Thank you for participating in this study! Your participation is voluntary, and is greatly appreciated. We anticipate that your participation in this study presents no greater risk than everyday internet use. We are committed to protecting your privacy. After validating that your response qualifies for payment, your answers will remain anonymous and will only take part in aggregate statistical analyses. You may withdraw from the study at any time if you feel uncomfortable answering some questions.

It is very important that you complete this study on your own and with adequate effort.

## Additional Information

The main researchers conducting this study are Ori Heffetz, a professor at Cornell University, and Guy Ishai. Please ask any questions you have using the Prolific messaging system. If you have any questions or concerns regarding your rights as a subject in this study, you may contact the Institutional Review Board (IRB) for Human Participants at 607-255-5138 or access their website at <http://www.irb.cornell.edu>. You may also anonymously report your concerns or complaints through Ethicspoint online at [www.hotline.cornell.edu](http://www.hotline.cornell.edu) or by calling toll free at 1-866-293-3077. Ethicspoint is an independent organization that serves as a liaison between the University and the person bringing the complaint to ensure anonymity.

Confirmation:

- Yes, I agree to participate in the study
- No, I do not agree to participate in the study

Please enter your Prolific ID:

Next

## D.2.0 Null Description

### The Basics

*In this study, you and three computerized participants, Ruth, Shirley, and Theresa, are going to play a game for four prizes. Each prize is worth money, but might be worth a different amount of money for each participant.*

*You and the computerized participants will each rank the four prizes in any order you wish. Then, an **allocation process** will use these rankings to allocate the prizes—one prize for each participant.*

*The allocation process attempts to give each participant a prize that they ranked higher rather than a prize that they ranked lower. However, this is not always possible, since the allocation process must take into account the rankings of all participants.*

*You will now learn about the game and allocation process. The text in blue bubbles, such as this text, provides explanations about the game and allocation process. **Make sure you read it carefully.***

*A round of the game has three steps.*

### Step 1: Round Information

*In Step 1, you first see the **prizes** you can get in this round and how much money they are worth to **you**.*

In this round, the **prizes** are:

| Prize       | A   | B  | C   | D   |
|-------------|-----|----|-----|-----|
| Money worth | 67¢ | 7¢ | 95¢ | 45¢ |

In the table above, under each prize A, B, C or D, you can see how much money it would add to **your** earnings.

Each prize might be worth a **different** amount of money for each participant, and each participant can only see the money amounts relevant to **themselves**. However, the prizes that earn **you** a large amount of money are also likely to earn the **other participants** a large amount of money. There is more likely to be **competition** for the high-earning prizes.

The money worth of prizes for you and for the other participants can be different in different rounds of the game, and they were **determined beforehand**. You and the other participants **cannot affect the money worth of prizes**.

Still in Step 1, you see next what we call the **prize priorities**.

All four participants have some **priority** for getting each of the four prizes.

These priorities can affect the allocation of prizes.

The higher your priority is for getting some prize, the more likely you generally are to get that prize at the end of the process.

In this round, the **prize priorities** for you and for the other participants are:

| Prize                  | A       | B       | C       | D       |
|------------------------|---------|---------|---------|---------|
| 1st priority (highest) | Ruth    | Shirley | Theresa | You     |
| 2nd priority           | Shirley | You     | Shirley | Theresa |
| 3rd priority           | You     | Theresa | You     | Ruth    |
| 4th priority (lowest)  | Theresa | Ruth    | Ruth    | Shirley |

Each column shows the priorities of all participants for getting some prize, written from highest to lowest

The prize priorities can be different in different rounds of the game, and they were **determined beforehand**.

You and the other participants **cannot affect the prize priorities**.

## Step 2: Submit Your Ranking

In Step 2, you are asked to **rank the four prizes**.

Please type your ranking of the four prizes in an order of your choice in the box below. For example, if you want to rank Prize A first, Prize B second, Prize C third and Prize D fourth, type "A" followed by "B" followed by "C" followed by "D," and then click "Submit Ranking."

**C-A-B-D**

The computerized participants simultaneously submit their own rankings. They **do not know your own ranking**.

Their rankings are aimed at getting them their high-earning prizes. Your own ranking **cannot affect the computerized participants' rankings**.

## Step 3: Allocation Process

In Step 3, the allocation process allocates the prizes to participants. Then, you get the prize that was allocated to you.

Remember:

The allocation process attempts to give each participant a prize that they ranked higher rather than a prize that they ranked lower. However, this is not always possible, since the allocation process must take into account the rankings of all participants.

Additionally, the prize priorities can affect the allocation of prizes.

The higher your priority is for getting some prize, the more likely you generally are to get that prize at the end of the process.

### **You get Prize B.**

If this were a real round, your total earning would increase by 7¢.

That's it!

Click on the button below to proceed to training rounds.

Proceed to training rounds

## D.2.1 Null Description: Training Round 1

### Training Round 1/2

[Click for a general reminder on this study](#)

*This is a training round.*

*Everything is **the same** as in the real rounds you will play later on, except that you will **not** earn the money worth of the prize you will get. Instead, we will ask you questions which can count for your **Understanding Bonus** at the end of the study.*

*Remember: each question increases your Understanding Bonus only if you answer it correctly on your first attempt. Think about your answers carefully!*

#### Step 1: Round Information

In this round, your **prizes** are:

| Prize       | A   | B  | C   | D   |
|-------------|-----|----|-----|-----|
| Money worth | 79¢ | 9¢ | 45¢ | 94¢ |

[Click for a reminder on what the prizes mean](#)

Please determine whether the following statement is true or false:

If I rank some prize very **low** and get it, I may earn **less** than its money worth, shown in the table above. If I rank some prize very **high** and get it, I may earn **more** than its money worth.  
(Get it right on first try to increase your bonus)

- True  
 False

**Correct!** Your own ranking cannot affect the money worth of prizes shown in your table, which are determined beforehand.

**Good job on the first try!** This will count for your Understanding Bonus.

Please determine whether the following statement is true or false:

Every participant, including me and the computerized participants, has the same earnings table.  
(Get it right on first try to increase your bonus)

- True
- False

Correct! Each prize might be worth a different amount for each participant.  
Good job on the first try! This will count for your Understanding Bonus.

The **prize priorities** for you and for the other participants are:

| Prize                  | A       | B       | C       | D       |
|------------------------|---------|---------|---------|---------|
| 1st priority (highest) | You     | Theresa | Shirley | Ruth    |
| 2nd priority           | Shirley | You     | Ruth    | You     |
| 3rd priority           | Theresa | Shirley | Theresa | Theresa |
| 4th priority (lowest)  | Ruth    | Ruth    | You     | Shirley |

[Click here for a reminder on what the priorities mean](#)

Please determine whether the following statement is true or false:

If I place a prize very **low** in my ranking, then my priority for getting that prize (in the table above) might **decrease**. If I place a prize very **high** in my ranking, then my priority for getting that prize (in the table above) might **increase**.

(Get it right on first try to increase your bonus)

- True
- False

Correct! Your own ranking cannot affect the prize priorities. Instead, they are determined beforehand.  
Good job on the first try! This will count for your Understanding Bonus.

## Step 2: Submit Your Ranking

Click for a reminder on what this ranking means

Please rank the four prizes in an order of your choice.

**A-D-B-C**

## Step 3: Allocation Process

*Remember:*

*The allocation process attempts to give each participant a prize that they ranked higher rather than a prize that they ranked lower. However, this is not always possible, since the allocation process must take into account the rankings of all participants.*

*The prize priorities can affect the allocation of prizes.*

*The higher your priority is at some prize, the more likely you generally are to get that prize at the end of the process.*

### **You get Prize A.**

If this were a real round, your total earning would increase by 79¢.

Since this is a training round, the questions you answer correctly on the first attempt count for your Understanding Bonus.

Please answer the following question:

How many prizes can you get at most at the end of the allocation process? The correct answer is that you **always** get one prize, no more and no less, so you should select the number one.

(Get it right on first try to increase your bonus)

Answer:

**Correct! You always get one prize at the end of the allocation process.  
Good job on the first try! This will count for your Understanding Bonus.**

Please determine whether the following statement is true or false:

I just submitted some ranking and got some prize. It is possible that if I had submitted a different ranking, my ranking would have **affected the other participants' rankings** such that I would have gotten a different prize.

(Get it right on first try to increase your bonus)

- True
- False

Correct! Your own ranking cannot affect the other participants' rankings.  
Good job on the first try! This will count for your Understanding Bonus.

Proceed

## D.2.2 Null: Training Round 2 (Cornell)

# Training Round 2/2

[Click for a general reminder on this study](#)

*This is a training round.*

*Everything is **the same** as in the real rounds you will play later on, except that you will **not** earn the money worth of the prize you will get. Instead, completing this round will count for your **Understanding Bonus** at the end of the study.*

## Step 1: Round Information

In this round, your **prizes** are:

| Prize       | A   | B   | C  | D   |
|-------------|-----|-----|----|-----|
| Money worth | 30¢ | 99¢ | 8¢ | 86¢ |

[Click for a reminder on what the prizes mean](#)

The **prize priorities** for you and for the other participants are:

| Prize                  | A       | B       | C       | D       |
|------------------------|---------|---------|---------|---------|
| 1st priority (highest) | You     | You     | Shirley | Theresa |
| 2nd priority           | Shirley | Theresa | Ruth    | Ruth    |
| 3rd priority           | Theresa | Shirley | Theresa | You     |
| 4th priority (lowest)  | Ruth    | Ruth    | You     | Shirley |

[Click here for a reminder on what the priorities mean](#)

## Step 2: Submit Your Ranking

[Click for a reminder on what this ranking means](#)

Please rank the four prizes in an order of your choice.

**A-D-B-C**

## Step 3: Allocation Process

**You get Prize A.**

If this were a real round, your total earning would increase by 30¢.

Since this is a training round, it will count for your Understanding Bonus like answering one question correctly.

Proceed

---

## Training Round 2/2

[Click for a general reminder on this study](#)

*This is a training round.*

*Everything is **the same** as in the real rounds you will play later on, except that you will **not** earn the money worth of the prize you will get. Instead, completing this round will count for your **Understanding Bonus** at the end of the study.*

### Step 1: Round Information

In this round, your **prizes** are:

| Prize       | A   | B   | C  | D   |
|-------------|-----|-----|----|-----|
| Money worth | 30¢ | 99¢ | 8¢ | 86¢ |

[Click for a reminder on what the prizes mean](#)

The **prize priorities** for you and for the other participants are:

| Prize                  | A       | B       | C       | D       |
|------------------------|---------|---------|---------|---------|
| 1st priority (highest) | You     | You     | Shirley | Theresa |
| 2nd priority           | Shirley | Theresa | Ruth    | Ruth    |
| 3rd priority           | Theresa | Shirley | Theresa | You     |
| 4th priority (lowest)  | Ruth    | Ruth    | You     | Shirley |

[Click here for a reminder on what the priorities mean](#)

### Step 2: Submit Your Ranking

[Click for a reminder on what this ranking means](#)

Please rank the four prizes in an order of your choice.

**A-B-C-D**

### Step 3: Allocation Process

#### **You get Prize A.**

If this were a real round, your total earning would increase by 30p.

Since this is a training round, it will count for your Understanding Bonus like answering one question correctly.

#### **- This is a point of no return -**

*On the next screens you will continue to read long and detailed explanations, which may be more complicated than those you just learned. You will complete many tasks that depend on your understanding of these explanations.*

*If you feel that you currently lack sufficient time or mental resources for additional highly demanding 50-60 minutes, no worries!*

- *We appreciate your participation and effort. You can quit the study now, **without advancing to the next screen**, and enter the completion code **CNF8D943**. If you do so, we will provide you with a **partial payment of £2** for your effort so far. Please send us a chat message in the Zoom session prior to leaving.*
- *This is a one-time offer. If you advance to the next screen and at some point quit the study, we will **not** be able to provide a partial payment.*

*If you are up to the challenge (and we certainly hope you are!), please note:*

***It is crucial for our purposes that you complete the study if you advance beyond this point.*** Making some mistakes in understanding questions along the way will be perfectly normal—please stay with us. Our main objective is that you try your best at understanding and playing the game.

*If you do not wish to exit early for the partial payment of £2, and if you are ready for a difficult additional 50-60 minute study, please press Proceed below.*

**Proceed**

### D.3.1.0 Traditional DA Mechanics Description

## How the Allocation Process Works

*You will now learn the full technical details of the allocation process.*

***These details are important to learn:*** *You may be able to apply your knowledge of them to make better decisions in the upcoming real rounds of this study.*

*Some details may seem confusing at first. This is quite natural! But don't worry, we will show you step-by-step examples. Things will become clearer along the way.*

### Overview of allocation process

*The following image illustrates how your own ranking, the rankings of the other participants and the prize priorities affect the prize you get:*

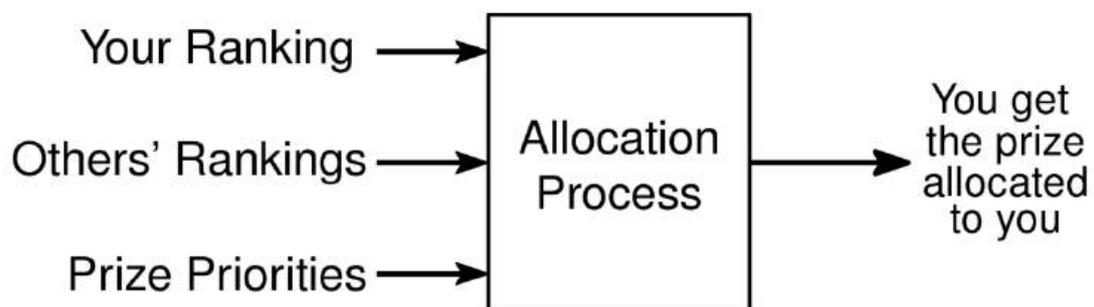

### Details of allocation process

*The allocation process is a multi-step process, as follows (it may look complicated, but don't worry, we will rehearse this in a moment):*

In the first step, each participant is paired to their **highest**-rank prize.

In the next step, possible conflicts are detected and solved.

If two (or more) participants are paired to the same prize, this is a **conflict**.

Each conflict is solved in two steps:

- **Unpair**: only the participant highest in that prize's priorities remains paired to that prize. The others get unpaired.
- **Re-pair**: all unpaired participants can only get re-paired to prizes that they were not paired with before. Each unpaired participant is re-paired to their **highest-rank** prize among the prizes they **were not yet paired with**.

Later steps continue in the same way, by detecting and solving new conflicts.

Like before, if two (or more) participants are paired to the same prize, this is a **conflict**.

The conflict is solved using the same **Unpair** and **Re-pair** steps from above.

A participant can get unpaired from a prize **even if they successfully got paired to that prize in a previous step**.

When there are no more conflicts, the process is over. The result is each participant being paired to a different prize.

Each prize is then allocated to the participant paired to it.

On the next screens you will play training rounds of the game to master your understanding of the allocation process. Click the button below to proceed to these rounds.

Proceed to training rounds

### D.3.1.1 Traditional DA Mechanics: Training Round 1

## How the Allocation Process Works: Training Round 1/3

[Click for a general reminder on this study](#)

[Click for a reminder on the technical details of the allocation process](#)

*This is a training round.*

*Everything is **the same** as in the real rounds you will play later on, except that you will **not** earn the money worth of the prize you will get. Instead, we will ask you questions which can count for your **Understanding Bonus** at the end of the study.*

*Remember: each question increases your Understanding Bonus only if you answer it correctly on your first attempt. Think about your answers carefully!*

### Step 1: Round Information

In this round, the **prizes** are:

| Prize       | A                                           | B | C | D |
|-------------|---------------------------------------------|---|---|---|
| Money worth | - Training round. No earnings from prizes - |   |   |   |

[Click for a reminder on what the prizes mean](#)

The **prize priorities** for you and for the other participants are:

| Prize                  | A       | B       | C       | D       |
|------------------------|---------|---------|---------|---------|
| 1st priority (highest) | Ruth    | Ruth    | Shirley | You     |
| 2nd priority           | Shirley | Shirley | Theresa | Theresa |
| 3rd priority           | Theresa | You     | Ruth    | Shirley |
| 4th priority (lowest)  | You     | Theresa | You     | Ruth    |

Click for a reminder on what the priorities mean

## Step 2: Submit Your Ranking

Click for a reminder on what this ranking means

Please rank the four prizes **in the fixed, specific order C-A-B-D**.

**C-A-B-D**

## Step 3: Allocation Process

You are going to perform the allocation process by yourself, according to what you learned. Since this is the first time, we will help with hints along the way. Click on the button below to start.

Proceed

---

# How the Allocation Process Works: Training Round 1/3

Click for a reminder on the technical details of the allocation process

The training round is not yet over. To complete it, you will perform the allocation process by yourself, instead of the computer performing it.

Remember: each step or question during the process will count for your Understanding Bonus only if you get it correctly on your first attempt. Think about your answers carefully!

Proceed

| Prize Priorities: |  |          |  | Participant Rankings: |  |          |  | reset ↻  |  |          |  |          |  |          |
|-------------------|--|----------|--|-----------------------|--|----------|--|----------|--|----------|--|----------|--|----------|
| <b>A</b>          |  | <b>B</b> |  | <b>C</b>              |  | <b>D</b> |  | <b>R</b> |  | <b>S</b> |  | <b>T</b> |  | <b>Y</b> |
| R                 |  | R        |  | S                     |  | Y        |  | A        |  | A        |  | B        |  | C        |
| S                 |  | S        |  | T                     |  | T        |  | C        |  | C        |  | A        |  | A        |
| T                 |  | Y        |  | R                     |  | S        |  | D        |  | D        |  | D        |  | B        |
| Y                 |  | T        |  | Y                     |  | R        |  | B        |  | B        |  | C        |  | D        |

**Pick participants to pair** → R S T Y

|          |                      |  |                                                                               |
|----------|----------------------|--|-------------------------------------------------------------------------------|
| <b>A</b> | <input type="text"/> |  | <b>R</b> = Ruth<br><b>S</b> = Shirley<br><b>T</b> = Theresa<br><b>Y</b> = You |
| <b>B</b> | <input type="text"/> |  |                                                                               |
| <b>C</b> | <input type="text"/> |  |                                                                               |
| <b>D</b> | <input type="text"/> |  |                                                                               |

Allocation Dashboard

# How the Allocation Process Works: Training Round 1/3

Click for a reminder on the technical details of the allocation process

Let's begin with a question about the **big picture**.

Please determine whether the following statement is true or false:

The allocation process determines the prize I get based on the prize priorities, my own ranking, and the other, computerized participants' rankings.

(Get it right on first try to increase your bonus)

- True
- False

Correct! The allocation process uses all these three components to determine the prize you get. Good job on the first try! This will count for your Understanding Bonus.

Proceed

### Prize Priorities:

| A | B | C | D |
|---|---|---|---|
| R | R | S | Y |
| S | S | T | T |
| T | Y | R | S |
| Y | T | Y | R |

### Participant Rankings:

| R | S | T | Y |
|---|---|---|---|
| A | A | B | C |
| C | C | A | A |
| D | D | D | B |
| B | B | C | D |

reset ↻

**Pick participants to pair →** R S T Y

|          |                      |                                                                               |
|----------|----------------------|-------------------------------------------------------------------------------|
| <b>A</b> | <input type="text"/> | <b>R</b> = Ruth<br><b>S</b> = Shirley<br><b>T</b> = Theresa<br><b>Y</b> = You |
| <b>B</b> | <input type="text"/> |                                                                               |
| <b>C</b> | <input type="text"/> |                                                                               |
| <b>D</b> | <input type="text"/> |                                                                               |

# How the Allocation Process Works: Training Round 1/3

Click for a reminder on the technical details of the allocation process

Now, you will perform all the steps determining the allocation and finally the prize you get.

We will guide you how to use the **Allocation Dashboard** below to find the allocation of prizes to all participants, using the prize priorities and participants' rankings.

Proceed

| Prize Priorities: |  |          |  | Participant Rankings: |  |          |   | reset ↻ |
|-------------------|--|----------|--|-----------------------|--|----------|---|---------|
| <b>A</b>          |  | <b>B</b> |  | <b>C</b>              |  | <b>D</b> |   |         |
| R                 |  | R        |  | S                     |  | Y        | R | A       |
| S                 |  | S        |  | T                     |  | T        | C | C       |
| T                 |  | Y        |  | R                     |  | S        | D | D       |
| Y                 |  | T        |  | Y                     |  | R        | B | B       |

**Pick participants to pair →** R S T Y

|          |                      |  |                                                                               |
|----------|----------------------|--|-------------------------------------------------------------------------------|
| <b>A</b> | <input type="text"/> |  | <b>R</b> = Ruth<br><b>S</b> = Shirley<br><b>T</b> = Theresa<br><b>Y</b> = You |
| <b>B</b> | <input type="text"/> |  |                                                                               |
| <b>C</b> | <input type="text"/> |  |                                                                               |
| <b>D</b> | <input type="text"/> |  |                                                                               |

Allocation Dashboard

# How the Allocation Process Works: Training Round 1/3

Click for a reminder on the technical details of the allocation process

On the upper left part of the dashboard below you see a condensed version of the **Prize Priorities** that you saw before.

Each letter under a prize name indicates one of the four participants. The higher it is placed in the column, the higher the priority of that participant at that prize.

**For example:** ... (click here to expand)

The column under the letter **"A"** indicates the priorities of Prize A. Ruth (**"R"**) has the first (highest) priority for getting that prize, Shirley (**"S"**) has the second priority, Theresa (**"T"**) has the third priority, and you (**"Y"**) have the fourth (lowest) priority.

Proceed

| Prize Priorities:                                                                                                                                                                                                                                                                                                                                | Participant Rankings:               | reset ↻                                                                       |                                                                               |          |                      |          |                      |          |                      |   |   |   |   |   |   |   |   |   |   |   |                                                                                                                                                                                                                                                                                                  |          |          |          |          |   |   |   |   |   |   |   |   |   |   |   |   |   |   |   |   |  |
|--------------------------------------------------------------------------------------------------------------------------------------------------------------------------------------------------------------------------------------------------------------------------------------------------------------------------------------------------|-------------------------------------|-------------------------------------------------------------------------------|-------------------------------------------------------------------------------|----------|----------------------|----------|----------------------|----------|----------------------|---|---|---|---|---|---|---|---|---|---|---|--------------------------------------------------------------------------------------------------------------------------------------------------------------------------------------------------------------------------------------------------------------------------------------------------|----------|----------|----------|----------|---|---|---|---|---|---|---|---|---|---|---|---|---|---|---|---|--|
| <table><tr><td><b>A</b></td><td><b>B</b></td><td><b>C</b></td><td><b>D</b></td></tr><tr><td>R</td><td>R</td><td>S</td><td>Y</td></tr><tr><td>S</td><td>S</td><td>T</td><td>T</td></tr><tr><td>T</td><td>Y</td><td>R</td><td>S</td></tr><tr><td>Y</td><td>T</td><td>Y</td><td>R</td></tr></table>                                                 | <b>A</b>                            | <b>B</b>                                                                      | <b>C</b>                                                                      | <b>D</b> | R                    | R        | S                    | Y        | S                    | S | T | T | T | Y | R | S | Y | T | Y | R | <table><tr><td><b>R</b></td><td><b>S</b></td><td><b>T</b></td><td><b>Y</b></td></tr><tr><td>A</td><td>A</td><td>B</td><td>C</td></tr><tr><td>C</td><td>C</td><td>A</td><td>A</td></tr><tr><td>D</td><td>D</td><td>D</td><td>B</td></tr><tr><td>B</td><td>B</td><td>C</td><td>D</td></tr></table> | <b>R</b> | <b>S</b> | <b>T</b> | <b>Y</b> | A | A | B | C | C | C | A | A | D | D | D | B | B | B | C | D |  |
| <b>A</b>                                                                                                                                                                                                                                                                                                                                         | <b>B</b>                            | <b>C</b>                                                                      | <b>D</b>                                                                      |          |                      |          |                      |          |                      |   |   |   |   |   |   |   |   |   |   |   |                                                                                                                                                                                                                                                                                                  |          |          |          |          |   |   |   |   |   |   |   |   |   |   |   |   |   |   |   |   |  |
| R                                                                                                                                                                                                                                                                                                                                                | R                                   | S                                                                             | Y                                                                             |          |                      |          |                      |          |                      |   |   |   |   |   |   |   |   |   |   |   |                                                                                                                                                                                                                                                                                                  |          |          |          |          |   |   |   |   |   |   |   |   |   |   |   |   |   |   |   |   |  |
| S                                                                                                                                                                                                                                                                                                                                                | S                                   | T                                                                             | T                                                                             |          |                      |          |                      |          |                      |   |   |   |   |   |   |   |   |   |   |   |                                                                                                                                                                                                                                                                                                  |          |          |          |          |   |   |   |   |   |   |   |   |   |   |   |   |   |   |   |   |  |
| T                                                                                                                                                                                                                                                                                                                                                | Y                                   | R                                                                             | S                                                                             |          |                      |          |                      |          |                      |   |   |   |   |   |   |   |   |   |   |   |                                                                                                                                                                                                                                                                                                  |          |          |          |          |   |   |   |   |   |   |   |   |   |   |   |   |   |   |   |   |  |
| Y                                                                                                                                                                                                                                                                                                                                                | T                                   | Y                                                                             | R                                                                             |          |                      |          |                      |          |                      |   |   |   |   |   |   |   |   |   |   |   |                                                                                                                                                                                                                                                                                                  |          |          |          |          |   |   |   |   |   |   |   |   |   |   |   |   |   |   |   |   |  |
| <b>R</b>                                                                                                                                                                                                                                                                                                                                         | <b>S</b>                            | <b>T</b>                                                                      | <b>Y</b>                                                                      |          |                      |          |                      |          |                      |   |   |   |   |   |   |   |   |   |   |   |                                                                                                                                                                                                                                                                                                  |          |          |          |          |   |   |   |   |   |   |   |   |   |   |   |   |   |   |   |   |  |
| A                                                                                                                                                                                                                                                                                                                                                | A                                   | B                                                                             | C                                                                             |          |                      |          |                      |          |                      |   |   |   |   |   |   |   |   |   |   |   |                                                                                                                                                                                                                                                                                                  |          |          |          |          |   |   |   |   |   |   |   |   |   |   |   |   |   |   |   |   |  |
| C                                                                                                                                                                                                                                                                                                                                                | C                                   | A                                                                             | A                                                                             |          |                      |          |                      |          |                      |   |   |   |   |   |   |   |   |   |   |   |                                                                                                                                                                                                                                                                                                  |          |          |          |          |   |   |   |   |   |   |   |   |   |   |   |   |   |   |   |   |  |
| D                                                                                                                                                                                                                                                                                                                                                | D                                   | D                                                                             | B                                                                             |          |                      |          |                      |          |                      |   |   |   |   |   |   |   |   |   |   |   |                                                                                                                                                                                                                                                                                                  |          |          |          |          |   |   |   |   |   |   |   |   |   |   |   |   |   |   |   |   |  |
| B                                                                                                                                                                                                                                                                                                                                                | B                                   | C                                                                             | D                                                                             |          |                      |          |                      |          |                      |   |   |   |   |   |   |   |   |   |   |   |                                                                                                                                                                                                                                                                                                  |          |          |          |          |   |   |   |   |   |   |   |   |   |   |   |   |   |   |   |   |  |
| <b>Pick participants to pair →</b>                                                                                                                                                                                                                                                                                                               | <b>R</b> <b>S</b> <b>T</b> <b>Y</b> |                                                                               |                                                                               |          |                      |          |                      |          |                      |   |   |   |   |   |   |   |   |   |   |   |                                                                                                                                                                                                                                                                                                  |          |          |          |          |   |   |   |   |   |   |   |   |   |   |   |   |   |   |   |   |  |
| <table><tr><td><b>A</b></td><td><input type="text"/></td><td rowspan="4"><b>R</b> = Ruth<br/><b>S</b> = Shirley<br/><b>T</b> = Theresa<br/><b>Y</b> = You</td></tr><tr><td><b>B</b></td><td><input type="text"/></td></tr><tr><td><b>C</b></td><td><input type="text"/></td></tr><tr><td><b>D</b></td><td><input type="text"/></td></tr></table> | <b>A</b>                            | <input type="text"/>                                                          | <b>R</b> = Ruth<br><b>S</b> = Shirley<br><b>T</b> = Theresa<br><b>Y</b> = You | <b>B</b> | <input type="text"/> | <b>C</b> | <input type="text"/> | <b>D</b> | <input type="text"/> |   |   |   |   |   |   |   |   |   |   |   |                                                                                                                                                                                                                                                                                                  |          |          |          |          |   |   |   |   |   |   |   |   |   |   |   |   |   |   |   |   |  |
| <b>A</b>                                                                                                                                                                                                                                                                                                                                         | <input type="text"/>                | <b>R</b> = Ruth<br><b>S</b> = Shirley<br><b>T</b> = Theresa<br><b>Y</b> = You |                                                                               |          |                      |          |                      |          |                      |   |   |   |   |   |   |   |   |   |   |   |                                                                                                                                                                                                                                                                                                  |          |          |          |          |   |   |   |   |   |   |   |   |   |   |   |   |   |   |   |   |  |
| <b>B</b>                                                                                                                                                                                                                                                                                                                                         | <input type="text"/>                |                                                                               |                                                                               |          |                      |          |                      |          |                      |   |   |   |   |   |   |   |   |   |   |   |                                                                                                                                                                                                                                                                                                  |          |          |          |          |   |   |   |   |   |   |   |   |   |   |   |   |   |   |   |   |  |
| <b>C</b>                                                                                                                                                                                                                                                                                                                                         | <input type="text"/>                |                                                                               |                                                                               |          |                      |          |                      |          |                      |   |   |   |   |   |   |   |   |   |   |   |                                                                                                                                                                                                                                                                                                  |          |          |          |          |   |   |   |   |   |   |   |   |   |   |   |   |   |   |   |   |  |
| <b>D</b>                                                                                                                                                                                                                                                                                                                                         | <input type="text"/>                |                                                                               |                                                                               |          |                      |          |                      |          |                      |   |   |   |   |   |   |   |   |   |   |   |                                                                                                                                                                                                                                                                                                  |          |          |          |          |   |   |   |   |   |   |   |   |   |   |   |   |   |   |   |   |  |

# How the Allocation Process Works: Training Round 1/3

Click for a reminder on the technical details of the allocation process

On the upper right part of the dashboard below you see a condensed version of the **Participant Rankings**.

Each letter under a participant's initial indicates one of the four prizes. The higher it is placed in the column, the higher that prize was ranked by that participant.

**For example:** ... (click here to expand)

The column under the letter **"R"** indicates the ranking submitted by the computerized participant Ruth. She ranked Prize A (**"A"**) first (highest), Prize C (**"C"**) second, Prize D (**"D"**) third, and Prize B (**"B"**) fourth (lowest).

Notice that the ranking under **"Y"** (you) is exactly the ranking that you submitted in the previous screen!

Notice: In real rounds of the game you do not see other participants' rankings, but now, since you are in charge of the allocation process, you are able to see them.

Proceed

| Prize Priorities: |          |          |          | Participant Rankings: |          |          |          | reset ↻ |
|-------------------|----------|----------|----------|-----------------------|----------|----------|----------|---------|
| <b>A</b>          | <b>B</b> | <b>C</b> | <b>D</b> | <b>R</b>              | <b>S</b> | <b>T</b> | <b>Y</b> |         |
| R                 | R        | S        | Y        | A                     | A        | B        | C        |         |
| S                 | S        | T        | T        | C                     | C        | A        | A        |         |
| T                 | Y        | R        | S        | D                     | D        | D        | B        |         |
| Y                 | T        | Y        | R        | B                     | B        | C        | D        |         |

**Pick participants to pair** → R S T Y

|          |                      |                                                                               |
|----------|----------------------|-------------------------------------------------------------------------------|
| <b>A</b> | <input type="text"/> | <b>R</b> = Ruth<br><b>S</b> = Shirley<br><b>T</b> = Theresa<br><b>Y</b> = You |
| <b>B</b> | <input type="text"/> |                                                                               |
| <b>C</b> | <input type="text"/> |                                                                               |
| <b>D</b> | <input type="text"/> |                                                                               |

# How the Allocation Process Works: Training Round 1/3

[Click for a reminder on the technical details of the allocation process](#)

The middle and lower parts of the dashboard enable you to pair participants to prizes, as will be explained next.

Proceed

| Prize Priorities: |  |          |  | Participant Rankings: |  |          |  | reset ↻  |  |          |  |          |  |          |
|-------------------|--|----------|--|-----------------------|--|----------|--|----------|--|----------|--|----------|--|----------|
| <b>A</b>          |  | <b>B</b> |  | <b>C</b>              |  | <b>D</b> |  | <b>R</b> |  | <b>S</b> |  | <b>T</b> |  | <b>Y</b> |
| R                 |  | R        |  | S                     |  | Y        |  | A        |  | A        |  | B        |  | C        |
| S                 |  | S        |  | T                     |  | T        |  | C        |  | C        |  | A        |  | A        |
| T                 |  | Y        |  | R                     |  | S        |  | D        |  | D        |  | D        |  | B        |
| Y                 |  | T        |  | Y                     |  | R        |  | B        |  | B        |  | C        |  | D        |

**Pick participants to pair** → R S T Y

|          |                      |  |                    |
|----------|----------------------|--|--------------------|
| <b>A</b> | <input type="text"/> |  | <b>R</b> = Ruth    |
| <b>B</b> | <input type="text"/> |  | <b>S</b> = Shirley |
| <b>C</b> | <input type="text"/> |  | <b>T</b> = Theresa |
| <b>D</b> | <input type="text"/> |  | <b>Y</b> = You     |

Allocation Dashboard

# How the Allocation Process Works: Training Round 1/3

Click for a reminder on the technical details of the allocation process

First, pair Ruth to her **highest-rank** prize. To do this:

1. Start from the "Pick participants to pair" row, and click on **Ruth ("R")**.
2. Then, in the list of four prizes at the bottom left part of the dashboard, click on "+" next to the prize that is **highest in Ruth's ranking**.

Hint: the prize that is highest in Ruth's ranking is indicated by the letter just under "R" in the Participant Rankings table.

After pairing, "A" and "R" will be colored purple in the two tables, to indicate that they are paired.

Only pair **Ruth ("R")!** You will pair the other participants in the next step.

Click Submit when done.  
(Get it right on first try to increase your bonus)

Correct!  
Good job on the first try! This will count for your Understanding Bonus.

Proceed

| Prize Priorities: |   |   |   | Participant Rankings: |   |   |   | reset ↻ |
|-------------------|---|---|---|-----------------------|---|---|---|---------|
| A                 | B | C | D | R                     | S | T | Y |         |
| R                 | R | S | Y | A                     | A | B | C |         |
| S                 | S | T | T | C                     | C | A | A |         |
| T                 | Y | R | S | D                     | D | D | B |         |
| Y                 | T | Y | R | B                     | B | C | D |         |

Pick participants to pair → S T Y

|   |                |
|---|----------------|
| A | <span>R</span> |
| B |                |
| C |                |
| D |                |

R = Ruth  
S = Shirley  
T = Theresa  
Y = You

# How the Allocation Process Works: Training Round 1/3

Click for a reminder on the technical details of the allocation process

Now do the same for the three other participants. One by one, pair each of them to their highest-rank prize.

Click Submit after completing all three.

(Get it right on first try to increase your bonus)

Correct!

Good job on the first try! This will count for your Understanding Bonus.

Proceed

| Prize Priorities:                                                                                                                                                                                                                                                                                  | Participant Rankings:            | reset ↻                                                                       |   |   |   |   |   |   |   |   |   |   |   |   |   |   |   |   |   |   |                                                                                                                                                                                                                                                                                                    |   |   |   |   |   |   |   |   |   |   |   |   |   |   |   |   |   |   |   |   |  |
|----------------------------------------------------------------------------------------------------------------------------------------------------------------------------------------------------------------------------------------------------------------------------------------------------|----------------------------------|-------------------------------------------------------------------------------|---|---|---|---|---|---|---|---|---|---|---|---|---|---|---|---|---|---|----------------------------------------------------------------------------------------------------------------------------------------------------------------------------------------------------------------------------------------------------------------------------------------------------|---|---|---|---|---|---|---|---|---|---|---|---|---|---|---|---|---|---|---|---|--|
| <table><thead><tr><th>A</th><th>B</th><th>C</th><th>D</th></tr></thead><tbody><tr><td>R</td><td>R</td><td>S</td><td>Y</td></tr><tr><td>S</td><td>S</td><td>T</td><td>T</td></tr><tr><td>T</td><td>Y</td><td>R</td><td>S</td></tr><tr><td>Y</td><td>T</td><td>Y</td><td>R</td></tr></tbody></table> | A                                | B                                                                             | C | D | R | R | S | Y | S | S | T | T | T | Y | R | S | Y | T | Y | R | <table><thead><tr><th>R</th><th>S</th><th>T</th><th>Y</th></tr></thead><tbody><tr><td>A</td><td>A</td><td>B</td><td>C</td></tr><tr><td>C</td><td>C</td><td>A</td><td>A</td></tr><tr><td>D</td><td>D</td><td>D</td><td>B</td></tr><tr><td>B</td><td>B</td><td>C</td><td>D</td></tr></tbody></table> | R | S | T | Y | A | A | B | C | C | C | A | A | D | D | D | B | B | B | C | D |  |
| A                                                                                                                                                                                                                                                                                                  | B                                | C                                                                             | D |   |   |   |   |   |   |   |   |   |   |   |   |   |   |   |   |   |                                                                                                                                                                                                                                                                                                    |   |   |   |   |   |   |   |   |   |   |   |   |   |   |   |   |   |   |   |   |  |
| R                                                                                                                                                                                                                                                                                                  | R                                | S                                                                             | Y |   |   |   |   |   |   |   |   |   |   |   |   |   |   |   |   |   |                                                                                                                                                                                                                                                                                                    |   |   |   |   |   |   |   |   |   |   |   |   |   |   |   |   |   |   |   |   |  |
| S                                                                                                                                                                                                                                                                                                  | S                                | T                                                                             | T |   |   |   |   |   |   |   |   |   |   |   |   |   |   |   |   |   |                                                                                                                                                                                                                                                                                                    |   |   |   |   |   |   |   |   |   |   |   |   |   |   |   |   |   |   |   |   |  |
| T                                                                                                                                                                                                                                                                                                  | Y                                | R                                                                             | S |   |   |   |   |   |   |   |   |   |   |   |   |   |   |   |   |   |                                                                                                                                                                                                                                                                                                    |   |   |   |   |   |   |   |   |   |   |   |   |   |   |   |   |   |   |   |   |  |
| Y                                                                                                                                                                                                                                                                                                  | T                                | Y                                                                             | R |   |   |   |   |   |   |   |   |   |   |   |   |   |   |   |   |   |                                                                                                                                                                                                                                                                                                    |   |   |   |   |   |   |   |   |   |   |   |   |   |   |   |   |   |   |   |   |  |
| R                                                                                                                                                                                                                                                                                                  | S                                | T                                                                             | Y |   |   |   |   |   |   |   |   |   |   |   |   |   |   |   |   |   |                                                                                                                                                                                                                                                                                                    |   |   |   |   |   |   |   |   |   |   |   |   |   |   |   |   |   |   |   |   |  |
| A                                                                                                                                                                                                                                                                                                  | A                                | B                                                                             | C |   |   |   |   |   |   |   |   |   |   |   |   |   |   |   |   |   |                                                                                                                                                                                                                                                                                                    |   |   |   |   |   |   |   |   |   |   |   |   |   |   |   |   |   |   |   |   |  |
| C                                                                                                                                                                                                                                                                                                  | C                                | A                                                                             | A |   |   |   |   |   |   |   |   |   |   |   |   |   |   |   |   |   |                                                                                                                                                                                                                                                                                                    |   |   |   |   |   |   |   |   |   |   |   |   |   |   |   |   |   |   |   |   |  |
| D                                                                                                                                                                                                                                                                                                  | D                                | D                                                                             | B |   |   |   |   |   |   |   |   |   |   |   |   |   |   |   |   |   |                                                                                                                                                                                                                                                                                                    |   |   |   |   |   |   |   |   |   |   |   |   |   |   |   |   |   |   |   |   |  |
| B                                                                                                                                                                                                                                                                                                  | B                                | C                                                                             | D |   |   |   |   |   |   |   |   |   |   |   |   |   |   |   |   |   |                                                                                                                                                                                                                                                                                                    |   |   |   |   |   |   |   |   |   |   |   |   |   |   |   |   |   |   |   |   |  |
| <b>Pick participants to pair →</b>                                                                                                                                                                                                                                                                 |                                  |                                                                               |   |   |   |   |   |   |   |   |   |   |   |   |   |   |   |   |   |   |                                                                                                                                                                                                                                                                                                    |   |   |   |   |   |   |   |   |   |   |   |   |   |   |   |   |   |   |   |   |  |
| A                                                                                                                                                                                                                                                                                                  | <input type="text" value="R S"/> | <b>R</b> = Ruth<br><b>S</b> = Shirley<br><b>T</b> = Theresa<br><b>Y</b> = You |   |   |   |   |   |   |   |   |   |   |   |   |   |   |   |   |   |   |                                                                                                                                                                                                                                                                                                    |   |   |   |   |   |   |   |   |   |   |   |   |   |   |   |   |   |   |   |   |  |
| B                                                                                                                                                                                                                                                                                                  | <input type="text" value="T"/>   |                                                                               |   |   |   |   |   |   |   |   |   |   |   |   |   |   |   |   |   |   |                                                                                                                                                                                                                                                                                                    |   |   |   |   |   |   |   |   |   |   |   |   |   |   |   |   |   |   |   |   |  |
| C                                                                                                                                                                                                                                                                                                  | <input type="text" value="Y"/>   |                                                                               |   |   |   |   |   |   |   |   |   |   |   |   |   |   |   |   |   |   |                                                                                                                                                                                                                                                                                                    |   |   |   |   |   |   |   |   |   |   |   |   |   |   |   |   |   |   |   |   |  |
| D                                                                                                                                                                                                                                                                                                  | <input type="text"/>             |                                                                               |   |   |   |   |   |   |   |   |   |   |   |   |   |   |   |   |   |   |                                                                                                                                                                                                                                                                                                    |   |   |   |   |   |   |   |   |   |   |   |   |   |   |   |   |   |   |   |   |  |

# How the Allocation Process Works: Training Round 1/3

Click for a reminder on the technical details of the allocation process

Each participant is now paired to a prize.

However, there are **conflicts**: two (or more) participants are paired to the same prize.

Notice: **Ruth** and **Shirley** are both paired to **Prize A**. This is a conflict.

To solve a conflict, the first step is **Unpair**.

According to this step, only one participant should remain paired to Prize A. **Which participant should remain paired to Prize A?**

Please select one of the answers below and then click Submit.

(Get it right on first try to increase your bonus)

- It is determined at random.
- The participant who got paired to Prize A first.
- The participant for whom Prize A is ranked higher.
- The participant highest in Prize A's priorities.

Correct! When there is a conflict at some prize, only the participant highest in that prize's priorities remain paired to that prize. The others should get unpaired.

Good job on the first try! This will count for your Understanding Bonus.

Proceed

| Prize Priorities:                                                                                                                                                                                                                                                    | Participant Rankings:            | reset ↻                                           |   |   |   |   |   |   |   |   |   |   |   |   |   |   |   |   |   |   |                                                                                                                                                                                                                                                                      |   |   |   |   |   |   |   |   |   |   |   |   |   |   |   |   |   |   |   |   |  |
|----------------------------------------------------------------------------------------------------------------------------------------------------------------------------------------------------------------------------------------------------------------------|----------------------------------|---------------------------------------------------|---|---|---|---|---|---|---|---|---|---|---|---|---|---|---|---|---|---|----------------------------------------------------------------------------------------------------------------------------------------------------------------------------------------------------------------------------------------------------------------------|---|---|---|---|---|---|---|---|---|---|---|---|---|---|---|---|---|---|---|---|--|
| <table><tr><td>A</td><td>B</td><td>C</td><td>D</td></tr><tr><td>R</td><td>R</td><td>S</td><td>Y</td></tr><tr><td>S</td><td>S</td><td>T</td><td>T</td></tr><tr><td>T</td><td>Y</td><td>R</td><td>S</td></tr><tr><td>Y</td><td>T</td><td>Y</td><td>R</td></tr></table> | A                                | B                                                 | C | D | R | R | S | Y | S | S | T | T | T | Y | R | S | Y | T | Y | R | <table><tr><td>R</td><td>S</td><td>T</td><td>Y</td></tr><tr><td>A</td><td>A</td><td>B</td><td>C</td></tr><tr><td>C</td><td>C</td><td>A</td><td>A</td></tr><tr><td>D</td><td>D</td><td>D</td><td>B</td></tr><tr><td>B</td><td>B</td><td>C</td><td>D</td></tr></table> | R | S | T | Y | A | A | B | C | C | C | A | A | D | D | D | B | B | B | C | D |  |
| A                                                                                                                                                                                                                                                                    | B                                | C                                                 | D |   |   |   |   |   |   |   |   |   |   |   |   |   |   |   |   |   |                                                                                                                                                                                                                                                                      |   |   |   |   |   |   |   |   |   |   |   |   |   |   |   |   |   |   |   |   |  |
| R                                                                                                                                                                                                                                                                    | R                                | S                                                 | Y |   |   |   |   |   |   |   |   |   |   |   |   |   |   |   |   |   |                                                                                                                                                                                                                                                                      |   |   |   |   |   |   |   |   |   |   |   |   |   |   |   |   |   |   |   |   |  |
| S                                                                                                                                                                                                                                                                    | S                                | T                                                 | T |   |   |   |   |   |   |   |   |   |   |   |   |   |   |   |   |   |                                                                                                                                                                                                                                                                      |   |   |   |   |   |   |   |   |   |   |   |   |   |   |   |   |   |   |   |   |  |
| T                                                                                                                                                                                                                                                                    | Y                                | R                                                 | S |   |   |   |   |   |   |   |   |   |   |   |   |   |   |   |   |   |                                                                                                                                                                                                                                                                      |   |   |   |   |   |   |   |   |   |   |   |   |   |   |   |   |   |   |   |   |  |
| Y                                                                                                                                                                                                                                                                    | T                                | Y                                                 | R |   |   |   |   |   |   |   |   |   |   |   |   |   |   |   |   |   |                                                                                                                                                                                                                                                                      |   |   |   |   |   |   |   |   |   |   |   |   |   |   |   |   |   |   |   |   |  |
| R                                                                                                                                                                                                                                                                    | S                                | T                                                 | Y |   |   |   |   |   |   |   |   |   |   |   |   |   |   |   |   |   |                                                                                                                                                                                                                                                                      |   |   |   |   |   |   |   |   |   |   |   |   |   |   |   |   |   |   |   |   |  |
| A                                                                                                                                                                                                                                                                    | A                                | B                                                 | C |   |   |   |   |   |   |   |   |   |   |   |   |   |   |   |   |   |                                                                                                                                                                                                                                                                      |   |   |   |   |   |   |   |   |   |   |   |   |   |   |   |   |   |   |   |   |  |
| C                                                                                                                                                                                                                                                                    | C                                | A                                                 | A |   |   |   |   |   |   |   |   |   |   |   |   |   |   |   |   |   |                                                                                                                                                                                                                                                                      |   |   |   |   |   |   |   |   |   |   |   |   |   |   |   |   |   |   |   |   |  |
| D                                                                                                                                                                                                                                                                    | D                                | D                                                 | B |   |   |   |   |   |   |   |   |   |   |   |   |   |   |   |   |   |                                                                                                                                                                                                                                                                      |   |   |   |   |   |   |   |   |   |   |   |   |   |   |   |   |   |   |   |   |  |
| B                                                                                                                                                                                                                                                                    | B                                | C                                                 | D |   |   |   |   |   |   |   |   |   |   |   |   |   |   |   |   |   |                                                                                                                                                                                                                                                                      |   |   |   |   |   |   |   |   |   |   |   |   |   |   |   |   |   |   |   |   |  |
| <b>Pick participants to pair →</b>                                                                                                                                                                                                                                   |                                  |                                                   |   |   |   |   |   |   |   |   |   |   |   |   |   |   |   |   |   |   |                                                                                                                                                                                                                                                                      |   |   |   |   |   |   |   |   |   |   |   |   |   |   |   |   |   |   |   |   |  |
| A                                                                                                                                                                                                                                                                    | <input type="text" value="R S"/> | R = Ruth<br>S = Shirley<br>T = Theresa<br>Y = You |   |   |   |   |   |   |   |   |   |   |   |   |   |   |   |   |   |   |                                                                                                                                                                                                                                                                      |   |   |   |   |   |   |   |   |   |   |   |   |   |   |   |   |   |   |   |   |  |
| B                                                                                                                                                                                                                                                                    | <input type="text" value="T"/>   |                                                   |   |   |   |   |   |   |   |   |   |   |   |   |   |   |   |   |   |   |                                                                                                                                                                                                                                                                      |   |   |   |   |   |   |   |   |   |   |   |   |   |   |   |   |   |   |   |   |  |
| C                                                                                                                                                                                                                                                                    | <input type="text" value="Y"/>   |                                                   |   |   |   |   |   |   |   |   |   |   |   |   |   |   |   |   |   |   |                                                                                                                                                                                                                                                                      |   |   |   |   |   |   |   |   |   |   |   |   |   |   |   |   |   |   |   |   |  |
| D                                                                                                                                                                                                                                                                    | <input type="text"/>             |                                                   |   |   |   |   |   |   |   |   |   |   |   |   |   |   |   |   |   |   |                                                                                                                                                                                                                                                                      |   |   |   |   |   |   |   |   |   |   |   |   |   |   |   |   |   |   |   |   |  |

# How the Allocation Process Works: Training Round 1/3

Click for a reminder on the technical details of the allocation process

The second step in solving conflicts is **Re-pair**.

After a participant gets unpaired, what new prize do they get paired to?

Please select one of the answers below and then click Submit.

(Get it right on first try to increase your bonus)

- A random prize that is currently unpaired to any participant.
- Their highest-rank prize among the prizes they were not yet paired with.
- Their highest-rank prize.

Correct! Each unpaired participant is re-paired to their highest-rank prize among the prizes they were **not yet paired with**.

Good job on the first try! This will count for your Understanding Bonus.

Proceed

### Prize Priorities:

| A | B | C | D |
|---|---|---|---|
| R | R | S | Y |
| S | S | T | T |
| T | Y | R | S |
| Y | T | Y | R |

### Participant Rankings:

| R | S | T | Y |
|---|---|---|---|
| A | A | B | C |
| C | C | A | A |
| D | D | D | B |
| B | B | C | D |

reset ↻

### Pick participants to pair →

|   |                                  |                                                   |
|---|----------------------------------|---------------------------------------------------|
| A | <input type="text" value="R S"/> | R = Ruth<br>S = Shirley<br>T = Theresa<br>Y = You |
| B | <input type="text" value="T"/>   |                                                   |
| C | <input type="text" value="Y"/>   |                                                   |
| D | <input type="text"/>             |                                                   |

# How the Allocation Process Works: Training Round 1/3

Click for a reminder on the technical details of the allocation process

Now, let's solve the conflict.

According to the Prize Priorities, **Ruth's** priority for getting **Prize A** is higher than **Shirley's**. Hence, **Shirley** should get unpaired from **Prize A**, and then get re-paired to her second highest-rank prize.

Perform this using the two steps:

1. **Unpair**: at the lower part of the dashboard, next to Prize A ("A"), click on **Shirley ("S")**.
2. **Re-pair**: at the same lower part of the dashboard, click on "+" next to Shirley's ("S") **second highest-rank prize**.

Hint: You can easily find which prize it is, using the Participant Rankings table: this is the prize right below the one that is currently colored purple under Shirley's name ("S")

Click Submit when done.  
(Get it right on first try to increase your bonus)

Correct!  
Good job on the first try! This will count for your Understanding Bonus.

Proceed

| Prize Priorities: |   |   |   | Participant Rankings: |   |   |   | reset ↻ |
|-------------------|---|---|---|-----------------------|---|---|---|---------|
| A                 | B | C | D | R                     | S | T | Y |         |
| R                 | R | S | Y | A                     | A | B | C |         |
| S                 | S | T | T | C                     | C | A | A |         |
| T                 | Y | R | S | D                     | D | D | B |         |
| Y                 | T | Y | R | B                     | B | C | D |         |

**Pick participants to pair →**

|   |                                  |                                                   |
|---|----------------------------------|---------------------------------------------------|
| A | <input type="text" value="R"/>   | R = Ruth<br>S = Shirley<br>T = Theresa<br>Y = You |
| B | <input type="text" value="T"/>   |                                                   |
| C | <input type="text" value="Y S"/> |                                                   |
| D | <input type="text"/>             |                                                   |

# How the Allocation Process Works: Training Round 1/3

Click for a reminder on the technical details of the allocation process

Is the process determining the allocation of prizes to participants over?  
(Get it right on first try to increase your bonus)

- No, there are new conflicts: two (or more) participants are paired to the same prize.
- No, some participants are paired to prizes that are not in their highest rank.
- Yes, it is fine that two (or more) participants are paired to the same prize because they all get different amounts of money anyway.
- Yes, there are no more conflicts.

Correct! The process is only over when there are no more conflicts.  
Good job on the first try! This will count for your Understanding Bonus.

Proceed

### Prize Priorities:

| A | B | C | D |
|---|---|---|---|
| R | R | S | Y |
| S | S | T | T |
| T | Y | R | S |
| Y | T | Y | R |

### Participant Rankings:

| R | S | T | Y |
|---|---|---|---|
| A | A | B | C |
| C | C | A | A |
| D | D | D | B |
| B | B | C | D |

reset ↻

---

**Pick participants to pair →**

|   |                                  |                                                   |
|---|----------------------------------|---------------------------------------------------|
| A | <input type="text" value="R"/>   | R = Ruth<br>S = Shirley<br>T = Theresa<br>Y = You |
| B | <input type="text" value="T"/>   |                                                   |
| C | <input type="text" value="Y S"/> |                                                   |
| D | <input type="text"/>             |                                                   |

# How the Allocation Process Works: Training Round 1/3

Click for a reminder on the technical details of the allocation process

Find the next conflict and solve it like before. First, find all prizes that are paired to two (or more) participants. Then, perform the two steps:

- **Unpair:** for each such prize, keep only the participant with the highest priority for getting that prize paired to it.  
**Unpair** the other participants from that prize.
- **Re-pair:** re-pair these participants to their highest-rank prize among the prizes they were **not yet paired with**.

Hint: You can easily find which prize you should re-pair the unpaired participant to, using the Participant Rankings table: this is the prize right below the one that is currently colored purple under the unpaired participant's name.

**Only solve the conflict you see first on this screen!** If new conflicts emerge after solving the current one, wait. You will solve them one-by-one on the next screens.

Click Submit when done.

(Get it right on first try to increase your bonus)

Correct!

Good job on the first try! This will count for your Understanding Bonus.

Proceed

| Prize Priorities: |   |   |   | Participant Rankings: |   |   |   | reset ↻ |
|-------------------|---|---|---|-----------------------|---|---|---|---------|
| A                 | B | C | D | R                     | S | T | Y |         |
| R                 | R | S | Y | A                     | A | B | C |         |
| S                 | S | T | T | C                     | C | A | A |         |
| T                 | Y | R | S | D                     | D | D | B |         |
| Y                 | T | Y | R | B                     | B | C | D |         |

**Pick participants to pair →**

|   |                                  |                                                   |
|---|----------------------------------|---------------------------------------------------|
| A | <input type="text" value="R Y"/> | R = Ruth<br>S = Shirley<br>T = Theresa<br>Y = You |
| B | <input type="text" value="T"/>   |                                                   |
| C | <input type="text" value="S"/>   |                                                   |
| D | <input type="text"/>             |                                                   |

# How the Allocation Process Works: Training Round 1/3

Click for a reminder on the technical details of the allocation process

Is the process determining the allocation of prizes to participants over?  
(Get it right on first try to increase your bonus)

- No
- Yes

Correct! The process is only over when there are no more conflicts.  
Good job on the first try! This will count for your Understanding Bonus.

Proceed

### Prize Priorities:

| A | B | C | D |
|---|---|---|---|
| R | R | S | Y |
| S | S | T | T |
| T | Y | R | S |
| Y | T | Y | R |

### Participant Rankings:

| R | S | T | Y |
|---|---|---|---|
| A | A | B | C |
| C | C | A | A |
| D | D | D | B |
| B | B | C | D |

reset ↻

---

**Pick participants to pair →**

|   |                                  |                                                                               |
|---|----------------------------------|-------------------------------------------------------------------------------|
| A | <input type="text" value="R Y"/> | <b>R</b> = Ruth<br><b>S</b> = Shirley<br><b>T</b> = Theresa<br><b>Y</b> = You |
| B | <input type="text" value="T"/>   |                                                                               |
| C | <input type="text" value="S"/>   |                                                                               |
| D | <input type="text"/>             |                                                                               |

# How the Allocation Process Works: Training Round 1/3

Click for a reminder on the technical details of the allocation process

Find all conflicts and solve them like before. First, find all prizes that are paired to two (or more) participants. Then, perform the two steps:

- **Unpair:** for each such prize, keep only the participant with the highest priority for getting that prize paired to it.  
**Unpair** the other participants from that prize.
- **Re-pair:** re-pair these participants to their highest-rank prize among the prizes they were **not yet paired with**.

Hint: You can easily find which prize you should re-pair the unpaired participant to, using the Participant Rankings table: this is the prize right below the one that is currently colored purple under the unpaired participant's name.

**Only solve the conflict you see first on this screen!** If new conflicts emerge after solving the current one, wait. You will solve them one-by-one on the next screens.

Click Submit when done.

(Get it right on first try to increase your bonus)

Correct!

Good job on the first try! This will count for your Understanding Bonus.

Proceed

| Prize Priorities: |   |   |   | Participant Rankings: |   |   |   | reset ↻ |
|-------------------|---|---|---|-----------------------|---|---|---|---------|
| A                 | B | C | D | R                     | S | T | Y |         |
| R                 | R | S | Y | A                     | A | B | C |         |
| S                 | S | T | T | C                     | C | A | A |         |
| T                 | Y | R | S | D                     | D | D | B |         |
| Y                 | T | Y | R | B                     | B | C | D |         |

**Pick participants to pair →**

|   |                                  |                                                   |
|---|----------------------------------|---------------------------------------------------|
| A | <input type="text" value="R"/>   | R = Ruth<br>S = Shirley<br>T = Theresa<br>Y = You |
| B | <input type="text" value="T Y"/> |                                                   |
| C | <input type="text" value="S"/>   |                                                   |
| D | <input type="text"/>             |                                                   |

# How the Allocation Process Works: Training Round 1/3

Click for a reminder on the technical details of the allocation process

Is the process determining the allocation of prizes to participants over?  
(Get it right on first try to increase your bonus)

- No
- Yes

Correct! The process is only over when there are no more conflicts.  
Good job on the first try! This will count for your Understanding Bonus.

Proceed

### Prize Priorities:

| A | B | C | D |
|---|---|---|---|
| R | R | S | Y |
| S | S | T | T |
| T | Y | R | S |
| Y | T | Y | R |

### Participant Rankings:

| R | S | T | Y |
|---|---|---|---|
| A | A | B | C |
| C | C | A | A |
| D | D | D | B |
| B | B | C | D |

reset ↻

### Pick participants to pair →

|   |     |                                                   |
|---|-----|---------------------------------------------------|
| A | R   | R = Ruth<br>S = Shirley<br>T = Theresa<br>Y = You |
| B | T Y |                                                   |
| C | S   |                                                   |
| D |     |                                                   |

Allocation Dashboard

# How the Allocation Process Works: Training Round 1/3

Click for a reminder on the technical details of the allocation process

Find all conflicts and solve them like before. First, find all prizes that are paired to two (or more) participants. Then, perform the two steps:

- **Unpair:** for each such prize, keep only the participant with the highest priority for getting that prize paired to it.  
**Unpair** the other participants from that prize.
- **Re-pair:** re-pair these participants to their highest-rank prize among the prizes they were **not yet paired with**.

Hint: You can easily find which prize you should re-pair the unpaired participant to, using the Participant Rankings table: this is the prize right below the one that is currently colored purple under the unpaired participant's name.

**Only solve the conflict you see first on this screen!** If new conflicts emerge after solving the current one, wait. You will solve them one-by-one on the next screens.

Click Submit when done.

(Get it right on first try to increase your bonus)

Correct!

Good job on the first try! This will count for your Understanding Bonus.

Proceed

### Prize Priorities:

| A | B | C | D |
|---|---|---|---|
| R | R | S | Y |
| S | S | T | T |
| T | Y | R | S |
| Y | T | Y | R |

### Participant Rankings:

| R | S | T | Y |
|---|---|---|---|
| A | A | B | C |
| C | C | A | A |
| D | D | D | B |
| B | B | C | D |

reset ↻

---

**Pick participants to pair →**

|   |                                  |             |
|---|----------------------------------|-------------|
| A | <input type="text" value="R T"/> | R = Ruth    |
| B | <input type="text" value="Y"/>   | S = Shirley |
| C | <input type="text" value="S"/>   | T = Theresa |
| D | <input type="text"/>             | Y = You     |

# How the Allocation Process Works: Training Round 1/3

Click for a reminder on the technical details of the allocation process

Is the process determining the allocation of prizes to participants over?  
(Get it right on first try to increase your bonus)

- No
- Yes

Correct! The process is only over when there are no more conflicts.  
Good job on the first try! This will count for your Understanding Bonus.

Proceed

### Prize Priorities:

| A | B | C | D |
|---|---|---|---|
| R | R | S | Y |
| S | S | T | T |
| T | Y | R | S |
| Y | T | Y | R |

### Participant Rankings:

| R | S | T | Y |
|---|---|---|---|
| A | A | B | C |
| C | C | A | A |
| D | D | D | B |
| B | B | C | D |

reset ↻

### Pick participants to pair →

|   |     |                                                   |
|---|-----|---------------------------------------------------|
| A | R T | R = Ruth<br>S = Shirley<br>T = Theresa<br>Y = You |
| B | Y   |                                                   |
| C | S   |                                                   |
| D |     |                                                   |

# How the Allocation Process Works: Training Round 1/3

Click for a reminder on the technical details of the allocation process

Find all conflicts and solve them like before. First, find all prizes that are paired to two (or more) participants. Then, perform the two steps:

- **Unpair:** for each such prize, keep only the participant with the highest priority for getting that prize paired to it.  
**Unpair** the other participants from that prize.
- **Re-pair:** re-pair these participants to their highest-rank prize among the prizes they were **not yet paired with**.

Hint: You can easily find which prize you should re-pair the unpaired participant to, using the Participant Rankings table: this is the prize right below the one that is currently colored purple under the unpaired participant's name.

**Only solve the conflict you see first on this screen!** If new conflicts emerge after solving the current one, wait. You will solve them one-by-one on the next screens.

Click Submit when done.

(Get it right on first try to increase your bonus)

Correct!

Good job on the first try! This will count for your Understanding Bonus.

Proceed

| Prize Priorities: |   |   |   | Participant Rankings: |   |   |   | reset ↻ |
|-------------------|---|---|---|-----------------------|---|---|---|---------|
| A                 | B | C | D | R                     | S | T | Y |         |
| R                 | R | S | Y | A                     | A | B | C |         |
| S                 | S | T | T | C                     | C | A | A |         |
| T                 | Y | R | S | D                     | D | D | B |         |
| Y                 | T | Y | R | B                     | B | C | D |         |

**Pick participants to pair →**

|   |                                |                                                   |
|---|--------------------------------|---------------------------------------------------|
| A | <input type="text" value="R"/> | R = Ruth<br>S = Shirley<br>T = Theresa<br>Y = You |
| B | <input type="text" value="Y"/> |                                                   |
| C | <input type="text" value="S"/> |                                                   |
| D | <input type="text" value="T"/> |                                                   |

# How the Allocation Process Works: Training Round 1/3

Click for a reminder on the technical details of the allocation process

Is the process determining the allocation of prizes to participants over?  
(Get it right on first try to increase your bonus)

- No
- Yes

Correct! There are no more conflicts.  
Good job on the first try! This will count for your Understanding Bonus.

Proceed

### Prize Priorities:

| A | B | C | D |
|---|---|---|---|
| R | R | S | Y |
| S | S | T | T |
| T | Y | R | S |
| Y | T | Y | R |

### Participant Rankings:

| R | S | T | Y |
|---|---|---|---|
| A | A | B | C |
| C | C | A | A |
| D | D | D | B |
| B | B | C | D |

reset ↻

---

**Pick participants to pair →**

|   |   |
|---|---|
| A | R |
| B | Y |
| C | S |
| D | T |

R = Ruth  
S = Shirley  
T = Theresa  
Y = You

# How the Allocation Process Works: Training Round 1/3

Click for a reminder on the technical details of the allocation process

The allocation is the following:

- Prize A is allocated to Ruth.
- Prize B is allocated to You.
- Prize C is allocated to Shirely.
- Prize D is allocated to Theresa.

**Which of the following is true?**

(Get it right on first try to increase your bonus)

- I can get any of the four prizes with equal chances.
- I can get any prize I was paired with at some point in the allocation process, but I cannot know which one.
- I will get one of the prizes I was paired with at some point in the allocation process, chosen at random.
- I will get the prize allocated to me at the end of the allocation process.

Correct! Each participant **gets the prize they were paired with** at the end of the allocation process.  
Good job on the first try! This will count for your Understanding Bonus.

Proceed

### Prize Priorities:

| A | B | C | D |
|---|---|---|---|
| R | R | S | Y |
| S | S | T | T |
| T | Y | R | S |
| Y | T | Y | R |

### Participant Rankings:

| R | S | T | Y |
|---|---|---|---|
| A | A | B | C |
| C | C | A | A |
| D | D | D | B |
| B | B | C | D |

reset ↻

### Pick participants to pair →

|   |   |
|---|---|
| A | R |
| B | Y |
| C | S |
| D | T |

R = Ruth  
S = Shirley  
T = Theresa  
Y = You

# How the Allocation Process Works: Training Round 1/3

Click for a reminder on the technical details of the allocation process

## Which of the following is true?

(Get it right on first try to increase your bonus)

- Only the other participants' rankings are used to determine the allocation of prizes.
- Only my own ranking is used to determine the allocation of prizes.
- Only the prize priorities are used to determine the allocation of prizes.
- The prize priorities and all participants' rankings are used to determine the allocation of prizes.

Correct! The allocation process depends on all prize priorities and on each participant's ranking.  
Good job on the first try! This will count for your Understanding Bonus.

Proceed

### Prize Priorities:

|   |   |   |   |
|---|---|---|---|
| A | B | C | D |
| R | R | S | Y |
| S | S | T | T |
| T | Y | R | S |
| Y | T | Y | R |

### Participant Rankings:

|   |   |   |   |
|---|---|---|---|
| R | S | T | Y |
| A | A | B | C |
| C | C | A | A |
| D | D | D | B |
| B | B | C | D |

reset ↻

---

### Pick participants to pair →

|   |                                |                                                                               |
|---|--------------------------------|-------------------------------------------------------------------------------|
| A | <input type="text" value="R"/> | <b>R</b> = Ruth<br><b>S</b> = Shirley<br><b>T</b> = Theresa<br><b>Y</b> = You |
| B | <input type="text" value="Y"/> |                                                                               |
| C | <input type="text" value="S"/> |                                                                               |
| D | <input type="text" value="T"/> |                                                                               |

# How the Allocation Process Works: Training Round 1/3

Click for a reminder on the technical details of the allocation process

Now please verify you understand what participant each prize is allocated to. Choose the participant that each prize is allocated to next to all the prizes below:

Prize A : (Get it right on first try to increase your bonus)

Correct! Prize A is allocated to Ruth.  
Good job on the first try! This will count for your Understanding Bonus.

Proceed

### Prize Priorities:

|   |   |   |   |
|---|---|---|---|
| A | B | C | D |
| R | R | S | Y |
| S | S | T | T |
| T | Y | R | S |
| Y | T | Y | R |

### Participant Rankings:

|   |   |   |   |
|---|---|---|---|
| R | S | T | Y |
| A | A | B | C |
| C | C | A | A |
| D | D | D | B |
| B | B | C | D |

reset ↻

### Pick participants to pair →

|   |                                |
|---|--------------------------------|
| A | <input type="text" value="R"/> |
| B | <input type="text" value="Y"/> |
| C | <input type="text" value="S"/> |
| D | <input type="text" value="T"/> |

**R** = Ruth  
**S** = Shirley  
**T** = Theresa  
**Y** = You

# How the Allocation Process Works: Training Round 1/3

Click for a reminder on the technical details of the allocation process

Now please verify you understand what participant each prize is allocated to. Choose the participant that each prize is allocated to next to all the prizes below:

Prize B : (Get it right on first try to increase your bonus)

Correct! Prize B is allocated to You.

Proceed

### Prize Priorities:

| A | B | C | D |
|---|---|---|---|
| R | R | S | Y |
| S | S | T | T |
| T | Y | R | S |
| Y | T | Y | R |

### Participant Rankings:

| R | S | T | Y |
|---|---|---|---|
| A | A | B | C |
| C | C | A | A |
| D | D | D | B |
| B | B | C | D |

reset ↻

### Pick participants to pair →

|   |                                |                                                   |
|---|--------------------------------|---------------------------------------------------|
| A | <input type="text" value="R"/> | R = Ruth<br>S = Shirley<br>T = Theresa<br>Y = You |
| B | <input type="text" value="Y"/> |                                                   |
| C | <input type="text" value="S"/> |                                                   |
| D | <input type="text" value="T"/> |                                                   |

# How the Allocation Process Works: Training Round 1/3

Click for a reminder on the technical details of the allocation process

Now please verify you understand what participant each prize is allocated to. Choose the participant that each prize is allocated to next to all the prizes below:

Prize C : (Get it right on first try to increase your bonus)

Correct! Prize C is allocated to Shirley.  
Good job on the first try! This will count for your Understanding Bonus.

Proceed

### Prize Priorities:

| A | B | C | D |
|---|---|---|---|
| R | R | S | Y |
| S | S | T | T |
| T | Y | R | S |
| Y | T | Y | R |

### Participant Rankings:

| R | S | T | Y |
|---|---|---|---|
| A | A | B | C |
| C | C | A | A |
| D | D | D | B |
| B | B | C | D |

reset ↻

### Pick participants to pair →

|   |                                |                                                   |
|---|--------------------------------|---------------------------------------------------|
| A | <input type="text" value="R"/> | R = Ruth<br>S = Shirley<br>T = Theresa<br>Y = You |
| B | <input type="text" value="Y"/> |                                                   |
| C | <input type="text" value="S"/> |                                                   |
| D | <input type="text" value="T"/> |                                                   |

# How the Allocation Process Works: Training Round 1/3

Click for a reminder on the technical details of the allocation process

Now please verify you understand what participant each prize is allocated to. Choose the participant that each prize is allocated to next to all the prizes below:

Prize D : (Get it right on first try to increase your bonus)

Correct! Prize D is allocated to Theresa.  
Good job on the first try! This will count for your Understanding Bonus.

Proceed

### Prize Priorities:

| A | B | C | D |
|---|---|---|---|
| R | R | S | Y |
| S | S | T | T |
| T | Y | R | S |
| Y | T | Y | R |

### Participant Rankings:

| R | S | T | Y |
|---|---|---|---|
| A | A | B | C |
| C | C | A | A |
| D | D | D | B |
| B | B | C | D |

reset ↻

### Pick participants to pair →

|   |                                |                                                   |
|---|--------------------------------|---------------------------------------------------|
| A | <input type="text" value="R"/> | R = Ruth<br>S = Shirley<br>T = Theresa<br>Y = You |
| B | <input type="text" value="Y"/> |                                                   |
| C | <input type="text" value="S"/> |                                                   |
| D | <input type="text" value="T"/> |                                                   |

Allocation Dashboard

# How the Allocation Process Works: Training Round 1/3

Click for a reminder on the technical details of the allocation process

## Which of the following is true?

(Get it right on first try to increase your bonus)

- I will get the prize I ranked the lowest.
- If another participant does not want the prize allocated to them, then I may be able to switch prizes with them.
- I will get the last prize I was paired with during the allocation process.
- I might end up not getting any prize.

Correct! The last prize you were paired with is the prize allocated to you at the end of the allocation process, and you get this prize.

Good job on the first try! This will count for your Understanding Bonus.

Proceed

### Prize Priorities:

|   |   |   |   |
|---|---|---|---|
| A | B | C | D |
| R | R | S | Y |
| S | S | T | T |
| T | Y | R | S |
| Y | T | Y | R |

### Participant Rankings:

|   |   |   |   |
|---|---|---|---|
| R | S | T | Y |
| A | A | B | C |
| C | C | A | A |
| D | D | D | B |
| B | B | C | D |

reset ↻

### Pick participants to pair →

|   |   |
|---|---|
| A | R |
| B | Y |
| C | S |
| D | T |

R = Ruth  
S = Shirley  
T = Theresa  
Y = You

# How the Allocation Process Works: Training Round 1/3

Click for a reminder on the technical details of the allocation process

Based on the outcome of the allocation process, choose the prize that you ("Y") get in this round.  
(Get it right on first try to increase your bonus)

Correct!

Good job on the first try! This will count for your Understanding Bonus.

Proceed

### Prize Priorities:

| A | B | C | D |
|---|---|---|---|
| R | R | S | Y |
| S | S | T | T |
| T | Y | R | S |
| Y | T | Y | R |

### Participant Rankings:

| R | S | T | Y |
|---|---|---|---|
| A | A | B | C |
| C | C | A | A |
| D | D | D | B |
| B | B | C | D |

reset ↻

---

**Pick participants to pair →**

|   |                                |                                                                               |
|---|--------------------------------|-------------------------------------------------------------------------------|
| A | <input type="text" value="R"/> | <b>R</b> = Ruth<br><b>S</b> = Shirley<br><b>T</b> = Theresa<br><b>Y</b> = You |
| B | <input type="text" value="Y"/> |                                                                               |
| C | <input type="text" value="S"/> |                                                                               |
| D | <input type="text" value="T"/> |                                                                               |

# How the Allocation Process Works: Training Round 1/3

Click for a reminder on the technical details of the allocation process

The allocation process is over. **You get Prize B.**

Proceed

### Prize Priorities:

| A | B | C | D |
|---|---|---|---|
| R | R | S | Y |
| S | S | T | T |
| T | Y | R | S |
| Y | T | Y | R |

### Participant Rankings:

| R | S | T | Y |
|---|---|---|---|
| A | A | B | C |
| C | C | A | A |
| D | D | D | B |
| B | B | C | D |

reset ↻

### Pick participants to pair →

|   |   |
|---|---|
| A | R |
| B | Y |
| C | S |
| D | T |

R = Ruth  
S = Shirley  
T = Theresa  
Y = You

Allocation Dashboard

### D.3.1.2 Traditional DA Mechanics: Training Round 2

## How the Allocation Process Works: Training Round 2/3

[Click for a general reminder on this study](#)

[Click for a reminder on the technical details of the allocation process](#)

*This is a training round.*

*Everything is **the same** as in the real rounds you will play later on, except that you will **not** earn the money worth of the prize you will get. Instead, we will ask you questions which can count for your **Understanding Bonus** at the end of the study.*

*Remember: each question increases your Understanding Bonus only if you answer it correctly on your first attempt. Think about your answers carefully!*

### Step 1: Round Information

In this round, the **prizes** are:

| Prize       | A                                           | B | C | D |
|-------------|---------------------------------------------|---|---|---|
| Money worth | - Training round. No earnings from prizes - |   |   |   |

[Click for a reminder on what the prizes mean](#)

The **prize priorities** for you and for the other participants are:

| Prize                  | A       | B       | C       | D       |
|------------------------|---------|---------|---------|---------|
| 1st priority (highest) | Shirley | Shirley | Theresa | Theresa |
| 2nd priority           | You     | Theresa | You     | Ruth    |
| 3rd priority           | Ruth    | You     | Ruth    | You     |
| 4th priority (lowest)  | Theresa | Ruth    | Shirley | Shirley |

Click for a reminder on what the priorities mean

## Step 2: Submit Your Ranking

Click for a reminder on what this ranking means

Please rank the four prizes **in the fixed, specific order D-C-B-A**.

**D-C-B-A**

## Step 3: Allocation Process

You are going to perform the allocation process by yourself, according to what you learned.  
Click on the button below to start.

Proceed

---

# How the Allocation Process Works: Training Round 2/3

Click for a reminder on the technical details of the allocation process

In this training round, you will perform the allocation process by yourself, instead of the computer performing it.

Each step or question will count for your Understanding Bonus, so think about your answers carefully!

Proceed

| Prize Priorities: |  |          |  | Participant Rankings: |  |          |  | reset ↻  |  |          |  |          |  |          |
|-------------------|--|----------|--|-----------------------|--|----------|--|----------|--|----------|--|----------|--|----------|
| <b>A</b>          |  | <b>B</b> |  | <b>C</b>              |  | <b>D</b> |  | <b>R</b> |  | <b>S</b> |  | <b>T</b> |  | <b>Y</b> |
| S                 |  | S        |  | T                     |  | T        |  | D        |  | B        |  | B        |  | D        |
| Y                 |  | T        |  | Y                     |  | R        |  | A        |  | A        |  | C        |  | C        |
| R                 |  | Y        |  | R                     |  | Y        |  | B        |  | C        |  | D        |  | B        |
| T                 |  | R        |  | S                     |  | S        |  | C        |  | D        |  | A        |  | A        |

**Pick participants to pair →** R S T Y

|          |                      |  |                                                                               |
|----------|----------------------|--|-------------------------------------------------------------------------------|
| <b>A</b> | <input type="text"/> |  | <b>R</b> = Ruth<br><b>S</b> = Shirley<br><b>T</b> = Theresa<br><b>Y</b> = You |
| <b>B</b> | <input type="text"/> |  |                                                                               |
| <b>C</b> | <input type="text"/> |  |                                                                               |
| <b>D</b> | <input type="text"/> |  |                                                                               |

Allocation Dashboard

# How the Allocation Process Works: Training Round 2/3

Click for a reminder on the technical details of the allocation process

Find the **allocation** of prizes to participants using the Allocation Dashboard below. Use the multi-step process you learned.

**Note:** In this round, you should only submit once you find the **final allocation**. Do **not** separately submit steps of the process like in Training Round 1.

In case you are still not sure how to find the allocation by yourself, click on the button below to watch a helpful video explaining all the steps. Clicking on the video will pause/unpause it, and if you close and re-open the video, it will continue from the same point.

Click here for a video with step-by-step explanations

(To restart the video, please refresh the page)

Click Submit when you are done.

(Get it right on first try to increase your bonus; it will count as **5 questions**.)

If you only get it right on the second try it will still count for your bonus; it will count as **2 questions**.)

Correct allocation!

Good job on the first try! This will count as **5 questions** for your Understanding Bonus.

Proceed

### Prize Priorities:

|   |   |   |   |
|---|---|---|---|
| A | B | C | D |
| S | S | T | T |
| Y | T | Y | R |
| R | Y | R | Y |
| T | R | S | S |

### Participant Rankings:

|   |   |   |   |
|---|---|---|---|
| R | S | T | Y |
| D | B | B | D |
| A | A | C | C |
| B | C | D | B |
| C | D | A | A |

reset ↻

**Pick participants to pair →**

|   |   |
|---|---|
| A | Y |
| B | S |
| C | T |
| D | R |

R = Ruth  
S = Shirley  
T = Theresa  
Y = You

# How the Allocation Process Works: Training Round 2/3

Click for a reminder on the technical details of the allocation process

For each of the four prizes below, choose **the participant to whom this prize is allocated**, based on the result of the allocation process.

Click Submit when you are done.  
(Get it right on first try to increase your bonus)

|                                |                                |                                |                                |
|--------------------------------|--------------------------------|--------------------------------|--------------------------------|
| Prize A                        | Prize B                        | Prize C                        | Prize D                        |
| <input type="text" value="Y"/> | <input type="text" value="S"/> | <input type="text" value="T"/> | <input type="text" value="R"/> |

Correct!  
Good job on the first try! This will count for your Understanding Bonus.

Proceed

### Prize Priorities:

|   |   |   |   |
|---|---|---|---|
| A | B | C | D |
| S | S | T | T |
| Y | T | Y | R |
| R | Y | R | Y |
| T | R | S | S |

### Participant Rankings:

|   |   |   |   |
|---|---|---|---|
| R | S | T | Y |
| D | B | B | D |
| A | A | C | C |
| B | C | D | B |
| C | D | A | A |

reset ↻

### Pick participants to pair →

|   |                                |
|---|--------------------------------|
| A | <input type="text" value="Y"/> |
| B | <input type="text" value="S"/> |
| C | <input type="text" value="T"/> |
| D | <input type="text" value="R"/> |

R = Ruth  
S = Shirley  
T = Theresa  
Y = You

# How the Allocation Process Works: Training Round 2/3

Click for a reminder on the technical details of the allocation process

Finally, select **the prize that you get** based on the allocation.

Correct! At the end of the process, each participant gets the prize they were allocated with.  
Good job on the first try! This will count for your Understanding Bonus.

Proceed

### Prize Priorities:

| A | B | C | D |
|---|---|---|---|
| S | S | T | T |
| Y | T | Y | R |
| R | Y | R | Y |
| T | R | S | S |

### Participant Rankings:

| R | S | T | Y |
|---|---|---|---|
| D | B | B | D |
| A | A | C | C |
| B | C | D | B |
| C | D | A | A |

reset ↻

### Pick participants to pair →

|   |   |
|---|---|
| A | Y |
| B | S |
| C | T |
| D | R |

R = Ruth  
S = Shirley  
T = Theresa  
Y = You

Allocation Dashboard

# How the Allocation Process Works: Training Round 2/3

Click for a reminder on the technical details of the allocation process

The allocation process is over. **You get Prize A.**

Proceed

### Prize Priorities:

| A | B | C | D |
|---|---|---|---|
| S | S | T | T |
| Y | T | Y | R |
| R | Y | R | Y |
| T | R | S | S |

### Participant Rankings:

| R | S | T | Y |
|---|---|---|---|
| D | B | B | D |
| A | A | C | C |
| B | C | D | B |
| C | D | A | A |

reset ↻

### Pick participants to pair →

|   |   |
|---|---|
| A | Y |
| B | S |
| C | T |
| D | R |

R = Ruth  
S = Shirley  
T = Theresa  
Y = You

Allocation Dashboard

### D.3.1.3 Traditional DA Mechanics: Training Round 3

## How the Allocation Process Works: Training Round 3/3

[Click for a general reminder on this study](#)

[Click for a reminder on the technical details of the allocation process](#)

*This is a training round.*

*Everything is **the same** as in the real rounds you will play later on, except that you will **not** earn the money worth of the prize you will get. Instead, we will ask you questions which can count for your **Understanding Bonus** at the end of the study.*

*Remember: each question increases your Understanding Bonus only if you answer it correctly on your first attempt. Think about your answers carefully!*

### Step 1: Round Information

In this round, the **prizes** are:

| Prize       | A                                           | B | C | D |
|-------------|---------------------------------------------|---|---|---|
| Money worth | - Training round. No earnings from prizes - |   |   |   |

[Click for a reminder on what the prizes mean](#)

The **prize priorities** for you and for the other participants are:

| Prize                  | A       | B       | C       | D       |
|------------------------|---------|---------|---------|---------|
| 1st priority (highest) | You     | Ruth    | Shirley | Ruth    |
| 2nd priority           | Theresa | You     | Ruth    | You     |
| 3rd priority           | Shirley | Theresa | Theresa | Shirley |
| 4th priority (lowest)  | Ruth    | Shirley | You     | Theresa |

Click for a reminder on what the priorities mean

## Step 2: Submit Your Ranking

Click for a reminder on what this ranking means

Please rank the four prizes **in the fixed, specific order D-B-C-A**.

**D-B-C-A**

## Step 3: Allocation Process

You are going to perform the allocation process by yourself, according to what you learned.  
Click on the button below to start.

Proceed

---

# How the Allocation Process Works: Training Round 3/3

Click for a reminder on the technical details of the allocation process

In this training round, you will perform the allocation process by yourself, instead of the computer performing it.

Each step or question will count for your Understanding Bonus, so think about your answers carefully!

Proceed

| Prize Priorities: |  |          |  | Participant Rankings: |  |          |  | reset ↻  |  |          |  |          |  |          |
|-------------------|--|----------|--|-----------------------|--|----------|--|----------|--|----------|--|----------|--|----------|
| <b>A</b>          |  | <b>B</b> |  | <b>C</b>              |  | <b>D</b> |  | <b>R</b> |  | <b>S</b> |  | <b>T</b> |  | <b>Y</b> |
| Y                 |  | R        |  | S                     |  | R        |  | A        |  | B        |  | D        |  | D        |
| T                 |  | Y        |  | R                     |  | Y        |  | B        |  | A        |  | B        |  | B        |
| S                 |  | T        |  | T                     |  | S        |  | D        |  | D        |  | A        |  | C        |
| R                 |  | S        |  | Y                     |  | T        |  | C        |  | C        |  | C        |  | A        |

**Pick participants to pair** → R S T Y

|          |                      |  |                                                                               |
|----------|----------------------|--|-------------------------------------------------------------------------------|
| <b>A</b> | <input type="text"/> |  | <b>R</b> = Ruth<br><b>S</b> = Shirley<br><b>T</b> = Theresa<br><b>Y</b> = You |
| <b>B</b> | <input type="text"/> |  |                                                                               |
| <b>C</b> | <input type="text"/> |  |                                                                               |
| <b>D</b> | <input type="text"/> |  |                                                                               |

Allocation Dashboard

# How the Allocation Process Works: Training Round 3/3

Click for a reminder on the technical details of the allocation process

Find the **allocation** of prizes to participants using the Allocation Dashboard below. Use the multi-step process you learned.

Note: In this round, you should only submit once you find the **final allocation**. Do **not** separately submit steps of the process like in Training Round 1.

Click Submit when you are done.

(Get it right on first try to increase your bonus; it will count as **5 questions**.)

If you only get it right on the second try it will still count for your bonus; it will count as **2 questions**.)

Correct allocation!

Good job on the second try! This will count as **2 questions** for your Understanding Bonus.

Proceed

| Prize Priorities: |   |   |   | Participant Rankings: |   |   |   | reset ↻ |
|-------------------|---|---|---|-----------------------|---|---|---|---------|
| A                 | B | C | D | R                     | S | T | Y |         |
| Y                 | R | S | R | A                     | B | D | D |         |
| T                 | Y | R | Y | B                     | A | B | B |         |
| S                 | T | T | S | D                     | D | A | C |         |
| R                 | S | Y | T | C                     | C | C | A |         |

**Pick participants to pair →**

|   |                                |                                                   |
|---|--------------------------------|---------------------------------------------------|
| A | <input type="text" value="T"/> | R = Ruth<br>S = Shirley<br>T = Theresa<br>Y = You |
| B | <input type="text" value="R"/> |                                                   |
| C | <input type="text" value="S"/> |                                                   |
| D | <input type="text" value="Y"/> |                                                   |

# How the Allocation Process Works: Training Round 3/3

Click for a reminder on the technical details of the allocation process

For each of the four prizes below, choose the participant to whom this prize is allocated, based on the result of the allocation process.

Click Submit when you are done.  
(Get it right on first try to increase your bonus)

|                                |                                |                                |                                |
|--------------------------------|--------------------------------|--------------------------------|--------------------------------|
| Prize A                        | Prize B                        | Prize C                        | Prize D                        |
| <input type="text" value="T"/> | <input type="text" value="R"/> | <input type="text" value="S"/> | <input type="text" value="Y"/> |

Correct!  
Good job on the first try! This will count for your Understanding Bonus.

Proceed

### Prize Priorities:

|   |   |   |   |
|---|---|---|---|
| A | B | C | D |
| Y | R | S | R |
| T | Y | R | Y |
| S | T | T | S |
| R | S | Y | T |

### Participant Rankings:

|   |   |   |   |
|---|---|---|---|
| R | S | T | Y |
| A | B | D | D |
| B | A | B | B |
| D | D | A | C |
| C | C | C | A |

reset ↻

### Pick participants to pair →

|   |                                |
|---|--------------------------------|
| A | <input type="text" value="T"/> |
| B | <input type="text" value="R"/> |
| C | <input type="text" value="S"/> |
| D | <input type="text" value="Y"/> |

R = Ruth  
S = Shirley  
T = Theresa  
Y = You

# How the Allocation Process Works: Training Round 3/3

Click for a reminder on the technical details of the allocation process

Finally, select **the prize that you get** based on the allocation.

Correct! At the end of the process, each participant gets the prize they were allocated with.  
Good job on the first try! This will count for your Understanding Bonus.

Proceed

### Prize Priorities:

| A | B | C | D |
|---|---|---|---|
| Y | R | S | R |
| T | Y | R | Y |
| S | T | T | S |
| R | S | Y | T |

### Participant Rankings:

| R | S | T | Y |
|---|---|---|---|
| A | B | D | D |
| B | A | B | B |
| D | D | A | C |
| C | C | C | A |

reset ↻

### Pick participants to pair →

|   |   |
|---|---|
| A | T |
| B | R |
| C | S |
| D | Y |

R = Ruth  
S = Shirley  
T = Theresa  
Y = You

# How the Allocation Process Works: Training Round 3/3

Click for a reminder on the technical details of the allocation process

The allocation process is over. **You get Prize D.**

Proceed

| Prize Priorities: |   |   |   | Participant Rankings: |   |   |   | reset ↻ |
|-------------------|---|---|---|-----------------------|---|---|---|---------|
| A                 | B | C | D | R                     | S | T | Y |         |
| Y                 | R | S | R | A                     | B | D | D |         |
| T                 | Y | R | Y | B                     | A | B | B |         |
| S                 | T | T | S | D                     | D | A | C |         |
| R                 | S | Y | T | C                     | C | C | A |         |

**Pick participants to pair →**

|   |   |
|---|---|
| A | T |
| B | R |
| C | S |
| D | Y |

R = Ruth  
S = Shirley  
T = Theresa  
Y = You

Allocation Dashboard

### D.3.2.0 Menu DA Mechanics Description

## How the Allocation Process Works

*You will now learn the full technical details of the allocation process.*

***These details are important to learn:*** *You may be able to apply your knowledge of them to make better decisions in the upcoming real rounds of this study.*

*Some details may seem confusing at first. This is quite natural! But don't worry, we will show you step-by-step examples. Things will become clearer along the way.*

### Overview of allocation process

*The prize you get is determined using an allocation process with two main steps:*

- 1. The computer determines some group of **Obtainable Prizes** that you might receive. Your own ranking does not influence the Obtainable Prizes. Instead, they are determined using only the prize priorities and the rankings of the other participants.*
- 2. You get the Obtainable Prize that you **ranked highest** (in the ranking you submitted).*

***The important principle:*** *Your own ranking does **not** influence what the Obtainable Prizes are, but it **does** determine what you get from among the Obtainable Prizes—you get the Obtainable Prize that you ranked the **highest**.*

*The following image illustrates how your own ranking, the rankings of the other participants and the prize priorities affect the prize you get:*

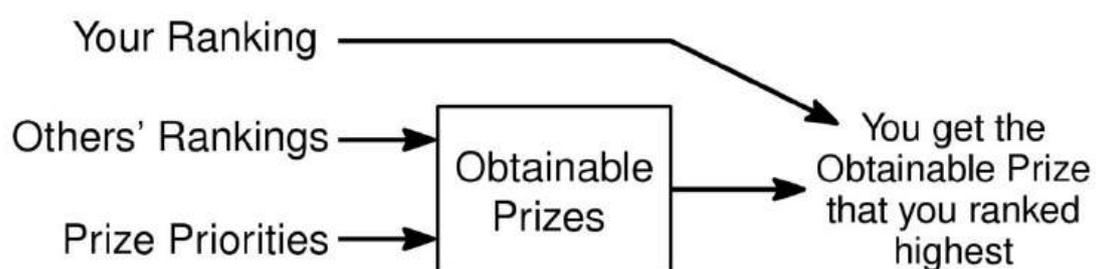

## Details of allocation process

### Priorities and rankings → Temporary allocation → Obtainable Prizes

The allocation process begins with a multi-step process. This process determines a “temporary allocation” of prizes to all participants **except for you**, and then determines your Obtainable Prizes based on this temporary allocation. This process **does not involve your own submitted ranking**, and works as follows (it may look complicated, but don’t worry, we will rehearse this in a moment):

In the first step, each prize is paired to its **highest**-priority participant, among all participants **except for you**.

In the next step, possible conflicts are detected and solved.  
If two (or more) prizes are paired to the same participant, this is a **conflict**.

Each conflict is solved in two steps:

- **Unpair**: only the prize highest in that participant's ranking remains paired to that participant. The others get unpaired.
- **Re-pair**: all unpaired prizes can only get re-paired to participants that they were not paired with before, and who are not you. Each unpaired prize is re-paired to its **highest**-priority participant, among the participants they **were not yet paired with** and **except for you**.

Later steps continue in the same way, by detecting and solving new conflicts. Like before, if two (or more) prizes are paired to the same participant, this is a **conflict**. The conflict is solved using the same **Unpair** and **Re-pair** steps from above.

A prize can get unpaired from a participant **even if it successfully got paired to that participant in a previous step**.

There is one **important thing to note about** the Re-pair step:

During the process, one prize will encounter a conflict with **every** participant, except for you, and will eventually get unpaired from all of them. That prize cannot be re-paired and will **remain unpaired** at the end of the process.

When there are no more conflicts and when one prize was unpaired from all participants (except for you), the process is over. The result is each prize, except for the unpaired one, being paired to a different participant (except for you).

Each prize except for the unpaired one is then **temporarily allocated** to the participant it is paired to.

The other participants do not get their prize from the temporary allocation; their prizes are determined by some other process. Instead, the temporary allocation is used to determine your Obtainable Prizes.

Next, we will tell you how the **Obtainable Prizes** are determined from the temporary allocation.

In this temporary allocation, no prize was allocated to you. To determine which prize is allocated to you, the computer first determines which prizes you can obtain in principle. These are the **Obtainable Prizes**.

You can obtain two kinds of prizes:

1. Any prize for which **your priority is higher** than that of the participant it is temporarily allocated to.
2. **The prize that was left unpaired in the temporary allocation.**

You cannot obtain any other prizes.

### **Obtainable Prizes → The prize you get**

Finally, we will remind you how the prize you get is selected from among the Obtainable Prizes, using your ranking.

In fact, this is the **only** time the allocation process uses your ranking.

From among the Obtainable Prizes, **you get the one that you ranked the highest**. In other words, the computer will look through your ranking from top to bottom, and you will get the first prize that is Obtainable.

On the next screens you will play training rounds of the game to master your understanding of the allocation process. Click the button below to proceed to these rounds.

Proceed to training rounds

### D.3.2.1 Menu DA Mechanics: Training Round 1

## How the Allocation Process Works: Training Round 1/3

[Click for a general reminder on this study](#)

[Click for a reminder on the technical details of the allocation process](#)

*This is a training round.*

*Everything is **the same** as in the real rounds you will play later on, except that you will **not** earn the money worth of the prize you will get. Instead, we will ask you questions which can count for your **Understanding Bonus** at the end of the study.*

*Remember: each question increases your Understanding Bonus only if you answer it correctly on your first attempt. Think about your answers carefully!*

### Step 1: Round Information

In this round, the **prizes** are:

| Prize       | A                                           | B | C | D |
|-------------|---------------------------------------------|---|---|---|
| Money worth | - Training round. No earnings from prizes - |   |   |   |

[Click for a reminder on what the prizes mean](#)

The **prize priorities** for you and for the other participants are:

| Prize                  | A       | B       | C       | D       |
|------------------------|---------|---------|---------|---------|
| 1st priority (highest) | Ruth    | Ruth    | Shirley | You     |
| 2nd priority           | Shirley | Shirley | Theresa | Theresa |
| 3rd priority           | Theresa | You     | Ruth    | Shirley |
| 4th priority (lowest)  | You     | Theresa | You     | Ruth    |

Click for a reminder on what the priorities mean

## Step 2: Submit Your Ranking

Click for a reminder on what this ranking means

Please rank the four prizes **in the fixed, specific order C-A-B-D**.

**C-A-B-D**

## Step 3: Allocation Process

You are going to perform the allocation process by yourself, according to what you learned.

Since this is the first time, we will help with hints along the way.

Click on the button below to start.

Proceed

# How the Allocation Process Works: Training Round 1/3

Click for a reminder on the technical details of the allocation process

The training round is not yet over. To complete it, you will perform the allocation process by yourself, instead of the computer performing it.

Remember: each step or question during the process will count for your Understanding Bonus only if you get it correctly on your first attempt. Think about your answers carefully!

Proceed

| Participant Rankings:        |                      |          |  | Prize Priorities: |  |          |  | reset ↻                |          |          |          |
|------------------------------|----------------------|----------|--|-------------------|--|----------|--|------------------------|----------|----------|----------|
| <b>R</b>                     |                      | <b>S</b> |  | <b>T</b>          |  | <b>Y</b> |  |                        |          |          |          |
| A                            |                      | A        |  | B                 |  | C        |  |                        |          |          |          |
| C                            |                      | C        |  | A                 |  | A        |  |                        |          |          |          |
| D                            |                      | D        |  | D                 |  | B        |  |                        |          |          |          |
| B                            |                      | B        |  | C                 |  | D        |  |                        |          |          |          |
|                              |                      |          |  |                   |  |          |  |                        |          |          |          |
| <b>A</b>                     |                      | <b>B</b> |  | <b>C</b>          |  | <b>D</b> |  |                        |          |          |          |
| R                            |                      | R        |  | S                 |  | Y        |  |                        |          |          |          |
| S                            |                      | S        |  | T                 |  | T        |  |                        |          |          |          |
| T                            |                      | Y        |  | R                 |  | S        |  |                        |          |          |          |
| Y                            |                      | T        |  | Y                 |  | R        |  |                        |          |          |          |
|                              |                      |          |  |                   |  |          |  |                        |          |          |          |
| <b>Pick prizes to pair</b> → |                      |          |  |                   |  |          |  | <b>A</b>               | <b>B</b> | <b>C</b> | <b>D</b> |
| <b>R</b>                     | <input type="text"/> |          |  |                   |  |          |  | <b>R = Ruth</b>        |          |          |          |
| <b>S</b>                     | <input type="text"/> |          |  |                   |  |          |  | <b>S = Shirley</b>     |          |          |          |
| <b>T</b>                     | <input type="text"/> |          |  |                   |  |          |  | <b>T = Theresa</b>     |          |          |          |
| <b>Y</b>                     | <input type="text"/> |          |  |                   |  |          |  | <b>Y = You</b>         |          |          |          |
| <b>U.P.</b>                  | <input type="text"/> |          |  |                   |  |          |  | <b>U.P. = Unpaired</b> |          |          |          |

# How the Allocation Process Works: Training Round 1/3

Click for a reminder on the technical details of the allocation process

Let's begin with a question about the **big picture**.

Please determine whether the following statement is true or false:

The allocation process first determines the Obtainable Prizes, which I **cannot affect with my own ranking**. Then, I always get the Obtainable Prize that is **placed highest in the ranking I submitted**. (Get it right on first try to increase your bonus)

- True
- False

Correct! In the allocation process, the group of Obtainable Prizes that you might receive is determined using only the other participants' rankings and the prize priorities. Then, from among the Obtainable Prizes, you get the one that you ranked highest.

Good job on the first try! This will count for your Understanding Bonus.

Proceed

| Participant Rankings: |   |   |   | Prize Priorities: |   |   |   | reset ↻ |
|-----------------------|---|---|---|-------------------|---|---|---|---------|
| R                     | S | T | Y | A                 | B | C | D |         |
| A                     | A | B | C | R                 | R | S | Y |         |
| C                     | C | A | A | S                 | S | T | T |         |
| D                     | D | D | B | T                 | Y | R | S |         |
| B                     | B | C | D | Y                 | T | Y | R |         |

Pick prizes to pair →

**A** **B** **C** **D**

|      |                      |                                                                      |
|------|----------------------|----------------------------------------------------------------------|
| R    | <input type="text"/> | R = Ruth<br>S = Shirley<br>T = Theresa<br>Y = You<br>U.P. = Unpaired |
| S    | <input type="text"/> |                                                                      |
| T    | <input type="text"/> |                                                                      |
| Y    | <input type="text"/> |                                                                      |
| U.P. | <input type="text"/> |                                                                      |

# How the Allocation Process Works: Training Round 1/3

[Click for a reminder on the technical details of the allocation process](#)

Now, you will perform all the steps determining the temporary allocation, the Obtainable Prizes, and finally the prize you get.

First, we will guide you how to use the **Allocation Dashboard** below to find the temporary allocation of prizes to all participants except for you, using the prize priorities and the rankings of all participants except for you.

Proceed

### Participant Rankings:

| R | S | T | Y |
|---|---|---|---|
| A | A | B | C |
| C | C | A | A |
| D | D | D | B |
| B | B | C | D |

### Prize Priorities:

| A | B | C | D |
|---|---|---|---|
| R | R | S | Y |
| S | S | T | T |
| T | Y | R | S |
| Y | T | Y | R |

reset ↻

### Pick prizes to pair →

**A** **B** **C** **D**

|             |                      |                                                                                                         |
|-------------|----------------------|---------------------------------------------------------------------------------------------------------|
| <b>R</b>    | <input type="text"/> | <b>R</b> = Ruth<br><b>S</b> = Shirley<br><b>T</b> = Theresa<br><b>Y</b> = You<br><b>U.P.</b> = Unpaired |
| <b>S</b>    | <input type="text"/> |                                                                                                         |
| <b>T</b>    | <input type="text"/> |                                                                                                         |
| <b>Y</b>    | <input type="text"/> |                                                                                                         |
| <b>U.P.</b> | <input type="text"/> |                                                                                                         |

Allocation Dashboard

# How the Allocation Process Works: Training Round 1/3

Click for a reminder on the technical details of the allocation process

On the upper left part of the dashboard below you see a condensed version of the **Participant Rankings**.

Each letter under a participant's initial indicates one of the four prizes. The higher it is placed in the column, the higher that prize was ranked by that participant.

**For example:** ... (click here to expand)

The column under the letter "R" indicates the ranking submitted by the computerized participant Ruth. She ranked Prize A ("A") first (highest), Prize C ("C") second, Prize D ("D") third, and Prize B ("B") fourth (lowest).

Notice: In real rounds of the game you do not see other participants' rankings, but now, since you are in charge of the allocation process, you are able to see them.

Proceed

| Participant Rankings: |   |   |   | Prize Priorities: |   |   |   | reset ↻ |
|-----------------------|---|---|---|-------------------|---|---|---|---------|
| R                     | S | T | Y | A                 | B | C | D |         |
| A                     | A | B | C | R                 | R | S | Y |         |
| C                     | C | A | A | S                 | S | T | T |         |
| D                     | D | D | B | T                 | Y | R | S |         |
| B                     | B | C | D | Y                 | T | Y | R |         |

Pick prizes to pair → A B C D

|      |                      |                                                                      |
|------|----------------------|----------------------------------------------------------------------|
| R    | <input type="text"/> | R = Ruth<br>S = Shirley<br>T = Theresa<br>Y = You<br>U.P. = Unpaired |
| S    | <input type="text"/> |                                                                      |
| T    | <input type="text"/> |                                                                      |
| Y    | <input type="text"/> |                                                                      |
| U.P. | <input type="text"/> |                                                                      |

Allocation Dashboard

# How the Allocation Process Works: Training Round 1/3

Click for a reminder on the technical details of the allocation process

On the upper right part of the dashboard below you see a condensed version of the **Prize Priorities** that you saw before.

Each letter under a prize name indicates one of the four participants. The higher it is placed in the column, the higher that participant's priority for getting that prize.

**For example:** ... (click here to expand)

The column under the letter **"A"** indicates the priorities of Prize A. Ruth (**"R"**) has the first (highest) priority for getting that prize, Shirley (**"S"**) has the second priority, Theresa (**"T"**) has the third priority, and you (**"Y"**) have the fourth (lowest) priority.

Proceed

| Participant Rankings: |   |   |   | Prize Priorities: |   |   |   | reset ↻ |
|-----------------------|---|---|---|-------------------|---|---|---|---------|
| R                     | S | T | Y | A                 | B | C | D |         |
| A                     | A | B | C | R                 | R | S | Y |         |
| C                     | C | A | A | S                 | S | T | T |         |
| D                     | D | D | B | T                 | Y | R | S |         |
| B                     | B | C | D | Y                 | T | Y | R |         |

Pick prizes to pair →

A B C D

|      |                      |                                                                      |
|------|----------------------|----------------------------------------------------------------------|
| R    | <input type="text"/> | R = Ruth<br>S = Shirley<br>T = Theresa<br>Y = You<br>U.P. = Unpaired |
| S    | <input type="text"/> |                                                                      |
| T    | <input type="text"/> |                                                                      |
| Y    | <input type="text"/> |                                                                      |
| U.P. | <input type="text"/> |                                                                      |

# How the Allocation Process Works: Training Round 1/3

Click for a reminder on the technical details of the allocation process

The middle and lower parts of the dashboard enable you to pair prizes to participants, as will be explained next.

Proceed

| Participant Rankings: |  |          |  | Prize Priorities: |  |          |  | reset ↻  |  |          |  |          |  |          |
|-----------------------|--|----------|--|-------------------|--|----------|--|----------|--|----------|--|----------|--|----------|
| <b>R</b>              |  | <b>S</b> |  | <b>T</b>          |  | <b>Y</b> |  | <b>A</b> |  | <b>B</b> |  | <b>C</b> |  | <b>D</b> |
| A                     |  | A        |  | B                 |  | C        |  | R        |  | R        |  | S        |  | Y        |
| C                     |  | C        |  | A                 |  | A        |  | S        |  | S        |  | T        |  | T        |
| D                     |  | D        |  | D                 |  | B        |  | T        |  | Y        |  | R        |  | S        |
| B                     |  | B        |  | C                 |  | D        |  | Y        |  | T        |  | Y        |  | R        |

**Pick prizes to pair** → A B C D

|             |                      |  |                        |
|-------------|----------------------|--|------------------------|
| <b>R</b>    | <input type="text"/> |  | <b>R</b> = Ruth        |
| <b>S</b>    | <input type="text"/> |  | <b>S</b> = Shirley     |
| <b>T</b>    | <input type="text"/> |  | <b>T</b> = Theresa     |
| <b>Y</b>    | <input type="text"/> |  | <b>Y</b> = You         |
| <b>U.P.</b> | <input type="text"/> |  | <b>U.P.</b> = Unpaired |

Allocation Dashboard

# How the Allocation Process Works: Training Round 1/3

Click for a reminder on the technical details of the allocation process

First, pair Prize A to its **highest-priority** participant. To do this:

1. Start from the "Pick prizes to pair" row, and click on **Prize A ("A")**.
2. Then, in the list of four participants at the bottom left part of the dashboard, click on "+" next to the participant, **except for you**, that is **highest in Prize A's priorities**.

Hint: the participant, except for you, that is highest in Prize A's priorities, is indicated by the letter just under "A" in the Prize Priorities table.

After pairing, "R" and "A" will be colored purple in the two tables, to indicate that they are paired.

Only pair **Prize A ("A")!** You will pair the other prizes in the next step.

Click Submit when done.

(Get it right on first try to increase your bonus)

Correct!

Good job on the first try! This will count for your Understanding Bonus.

Proceed

### Participant Rankings:

|   |   |   |   |
|---|---|---|---|
| R | S | T | Y |
| A | A | B | C |
| C | C | A | A |
| D | D | D | B |
| B | B | C | D |

### Prize Priorities:

|   |   |   |   |
|---|---|---|---|
| A | B | C | D |
| R | R | S | Y |
| S | S | T | T |
| T | Y | R | S |
| Y | T | Y | R |

---

**Pick prizes to pair →**

B

C

D

---

|      |   |
|------|---|
| R    | A |
| S    |   |
| T    |   |
| Y    |   |
| U.P. |   |

**R** = Ruth

**S** = Shirley

**T** = Theresa

**Y** = You

**U.P.** = Unpaired

# How the Allocation Process Works: Training Round 1/3

Click for a reminder on the technical details of the allocation process

Now do the same for the three other prizes. One by one, pair each of them to its **highest-priority** participant, except for you.

Hint: The highest-priority participant at Prize D is You, but You cannot be paired with it during this stage of the process.

Who is Prize D's highest-priority participant, **except for you**? (Another hint: it is Theresa)

Click Submit after completing all three.  
(Get it right on first try to increase your bonus)

Correct!  
Good job on the first try! This will count for your Understanding Bonus.

Proceed

### Participant Rankings:

|   |   |   |   |
|---|---|---|---|
| R | S | T | Y |
| A | A | B | C |
| C | C | A | A |
| D | D | D | B |
| B | B | C | D |

### Prize Priorities:

|   |   |   |   |
|---|---|---|---|
| A | B | C | D |
| R | R | S | Y |
| S | S | T | T |
| T | Y | R | S |
| Y | T | Y | R |

reset ↻

---

### Pick prizes to pair →

|      |                                                                                                                                                                                                                                                                                                                   |
|------|-------------------------------------------------------------------------------------------------------------------------------------------------------------------------------------------------------------------------------------------------------------------------------------------------------------------|
| R    | <div style="border: 1px solid gray; border-radius: 50%; width: 30px; height: 30px; display: flex; align-items: center; justify-content: center;">A</div> <div style="border: 1px solid gray; border-radius: 50%; width: 30px; height: 30px; display: flex; align-items: center; justify-content: center;">B</div> |
| S    | <div style="border: 1px solid gray; border-radius: 50%; width: 30px; height: 30px; display: flex; align-items: center; justify-content: center;">C</div>                                                                                                                                                          |
| T    | <div style="border: 1px solid gray; border-radius: 50%; width: 30px; height: 30px; display: flex; align-items: center; justify-content: center;">D</div>                                                                                                                                                          |
| Y    |                                                                                                                                                                                                                                                                                                                   |
| U.P. |                                                                                                                                                                                                                                                                                                                   |

**R** = Ruth

**S** = Shirley

**T** = Theresa

**Y** = You

**U.P.** = Unpaired

Allocation Dashboard

# How the Allocation Process Works: Training Round 1/3

Click for a reminder on the technical details of the allocation process

Each prize is now paired to a participant.

However, there are **conflicts**: two (or more) prizes are paired to the same participant.

Notice: **Prize A** and **Prize B** are both paired to **Ruth**. This is a conflict.

To solve a conflict, the first step is **Unpair**.

According to this step, only one prize should remain paired to Ruth. **Which prize should remain paired to Ruth?**

Please select one of the answers below and then click Submit.

(Get it right on first try to increase your bonus)

- It is determined at random.
- The prize that got paired to Ruth first.
- The prize where Ruth has higher priority.
- The prize highest in Ruth's ranking.

Correct! When there is a conflict at some participant, only the prize highest in that participant's ranking should remain paired to that participant. The others should get unpaired.  
Good job on the first try! This will count for your Understanding Bonus.

Proceed

| Participant Rankings: |   |   |   | Prize Priorities: |   |   |   | reset ↻ |
|-----------------------|---|---|---|-------------------|---|---|---|---------|
| R                     | S | T | Y | A                 | B | C | D |         |
| A                     | A | B | C | R                 | R | S | Y |         |
| C                     | C | A | A | S                 | S | T | T |         |
| D                     | D | D | B | T                 | Y | R | S |         |
| B                     | B | C | D | Y                 | T | Y | R |         |

**Pick prizes to pair →**

|      |                                  |                                                                      |
|------|----------------------------------|----------------------------------------------------------------------|
| R    | <input type="text" value="A B"/> | R = Ruth<br>S = Shirley<br>T = Theresa<br>Y = You<br>U.P. = Unpaired |
| S    | <input type="text" value="C"/>   |                                                                      |
| T    | <input type="text" value="D"/>   |                                                                      |
| Y    | <input type="text" value=""/>    |                                                                      |
| U.P. | <input type="text" value=""/>    |                                                                      |

# How the Allocation Process Works: Training Round 1/3

Click for a reminder on the technical details of the allocation process

The second step in solving conflicts is **Re-pair**.

After a prize gets unpaired, what new participant does it get paired to?

Please select one of the answers below and then click Submit.  
(Get it right on first try to increase your bonus)

- A random participant that is currently unpaired to any prize.
- Its highest-priority participant, among the participants it was not yet paired with and except for you.
- Its highest-priority participant.

Correct! Each unpaired prize is re-paired to its highest-priority participant, among the participants it was **not yet paired with and except for you**.  
Good job on the first try! This will count for your Understanding Bonus.

Proceed

### Participant Rankings:

|   |   |   |   |
|---|---|---|---|
| R | S | T | Y |
| A | A | B | C |
| C | C | A | A |
| D | D | D | B |
| B | B | C | D |

### Prize Priorities:

|   |   |   |   |
|---|---|---|---|
| A | B | C | D |
| R | R | S | Y |
| S | S | T | T |
| T | Y | R | S |
| Y | T | Y | R |

---

**Pick prizes to pair →**

|      |     |
|------|-----|
| R    | A B |
| S    | C   |
| T    | D   |
| Y    |     |
| U.P. |     |

**R** = Ruth

**S** = Shirley

**T** = Theresa

**Y** = You

**U.P.** = Unpaired

# How the Allocation Process Works: Training Round 1/3

Click for a reminder on the technical details of the allocation process

Now, let's solve the conflict.

According to the Participant Rankings, **Ruth** ranked **Prize A** higher than **Prize B**. Hence, Prize B should get unpaired from **Ruth**, and then get re-paired to its second highest-priority participant, among all participants **except for you**.

Perform this using the two steps:

- Unpair:** at the lower part of the dashboard, next to Ruth ("R"), click on **Prize B ("B")**.
- Re-pair:** at the same lower part of the dashboard, click on "+" next to Prize B's ("B") **second highest-priority participant**, among all participants **except for you**.

Hint: You can easily find which participant it is, using the Prize Priorities table: this is the participant right below the one that is currently colored purple under Prize B's name ("B"), or, in case that participant is you ("Y"), the one right below "Y".

Click Submit when done.

(Get it right on first try to increase your bonus)

Correct!

Good job on the first try! This will count for your Understanding Bonus.

Proceed

### Participant Rankings:

| R | S | T | Y |
|---|---|---|---|
| A | A | B | C |
| C | C | A | A |
| D | D | D | B |
| B | B | C | D |

### Prize Priorities:

| A | B | C | D |
|---|---|---|---|
| R | R | S | Y |
| S | S | T | T |
| T | Y | R | S |
| Y | T | Y | R |

---

**Pick prizes to pair →**

|      |     |
|------|-----|
| R    | A   |
| S    | C B |
| T    | D   |
| Y    |     |
| U.P. |     |

R = Ruth

S = Shirley

T = Theresa

Y = You

U.P. = Unpaired

# How the Allocation Process Works: Training Round 1/3

Click for a reminder on the technical details of the allocation process

Is the process determining the temporary allocation over?

(Remember: this process is only a first step, after which your Obtainable Prizes are determined, and then the prize you get is determined.)

(Get it right on first try to increase your bonus)

- No, there are new conflicts: two (or more) prizes are paired to the same participant.
- No, some prizes are paired to participants that do not have the highest priority for getting them.
- Yes, it is fine that two (or more) prizes are paired to the same participant because they all get different amounts of money anyway.
- Yes, there are no more conflicts.

Correct! The process is only over when there are no more conflicts.  
Good job on the first try! This will count for your Understanding Bonus.

Proceed

### Participant Rankings:

| R | S | T | Y |
|---|---|---|---|
| A | A | B | C |
| C | C | A | A |
| D | D | D | B |
| B | B | C | D |

### Prize Priorities:

| A | B | C | D |
|---|---|---|---|
| R | R | S | Y |
| S | S | T | T |
| T | Y | R | S |
| Y | T | Y | R |

---

**Pick prizes to pair →**

|      |     |
|------|-----|
| R    | A   |
| S    | C B |
| T    | D   |
| Y    |     |
| U.P. |     |

**R** = Ruth

**S** = Shirley

**T** = Theresa

**Y** = You

**U.P.** = Unpaired

# How the Allocation Process Works: Training Round 1/3

Click for a reminder on the technical details of the allocation process

Find the next conflict and solve it like before. First, find all participants that are paired to two (or more) prizes. Then, perform the two steps:

- **Unpair:** for each such participant, keep only the prize with the highest rank by that participant paired to her. **Unpair** the other prizes from that participant.
- **Re-pair:** re-pair these prizes to their highest-priority participant, among the participants they were **not yet paired with** and **except for you**.

Hint: You can easily find which participant you should re-pair the unpaired prize to, using the Prize Priorities table: this is the participant right below the one that is currently colored purple under the unpaired prize's name, or, in case that participant is you ("Y"), the one right below "Y".

**Only solve the conflict you see first on this screen!** If new conflicts emerge after solving the current one, wait. You will solve them one-by-one on the next screens.

Click Submit when done.  
(Get it right on first try to increase your bonus)

Correct!  
Good job on the first try! This will count for your Understanding Bonus.

Proceed

### Participant Rankings:

|   |   |   |   |
|---|---|---|---|
| R | S | T | Y |
| A | A | B | C |
| C | C | A | A |
| D | D | D | B |
| B | B | C | D |

### Prize Priorities:

|   |   |   |   |
|---|---|---|---|
| A | B | C | D |
| R | R | S | Y |
| S | S | T | T |
| T | Y | R | S |
| Y | T | Y | R |

reset ↻

---

### Pick prizes to pair →

|      |     |
|------|-----|
| R    | A   |
| S    | C   |
| T    | D B |
| Y    |     |
| U.P. |     |

R = Ruth

S = Shirley

T = Theresa

Y = You

U.P. = Unpaired

# How the Allocation Process Works: Training Round 1/3

Click for a reminder on the technical details of the allocation process

Is the process determining the temporary allocation over?

(Remember: this process is only a first step, after which your Obtainable Prizes are determined, and then the prize you get is determined.)

(Get it right on first try to increase your bonus)

- No
- Yes

Correct! The process is only over when there are no more conflicts.  
Good job on the first try! This will count for your Understanding Bonus.

Proceed

| Participant Rankings: |   |   |   | Prize Priorities: |   |   |   | reset ↻ |
|-----------------------|---|---|---|-------------------|---|---|---|---------|
| R                     | S | T | Y | A                 | B | C | D |         |
| A                     | A | B | C | R                 | R | S | Y |         |
| C                     | C | A | A | S                 | S | T | T |         |
| D                     | D | D | B | T                 | Y | R | S |         |
| B                     | B | C | D | Y                 | T | Y | R |         |

**Pick prizes to pair →**

|      |     |  |
|------|-----|--|
| R    | A   |  |
| S    | C   |  |
| T    | D B |  |
| Y    |     |  |
| U.P. |     |  |

R = Ruth  
S = Shirley  
T = Theresa  
Y = You  
U.P. = Unpaired

# How the Allocation Process Works: Training Round 1/3

Click for a reminder on the technical details of the allocation process

Find the next conflict and solve it like before. First, find all participants that are paired to two (or more) prizes. Then, perform the two steps:

- **Unpair:** for each such participant, keep only the prize with the highest rank by that participant paired to her. **Unpair** the other prizes from that participant.
- **Re-pair:** re-pair these prizes to their highest-priority participant, among the participants they were **not yet paired with** and **except for you**.

Hint: You can easily find which participant you should re-pair the unpaired prize to, using the Prize Priorities table: this is the participant right below the one that is currently colored purple under the unpaired prize's name, or, in case that participant is you ("Y"), the one right below "Y".

**Only solve the conflict you see first on this screen!** If new conflicts emerge after solving the current one, wait. You will solve them one-by-one on the next screens.

Click Submit when done.

(Get it right on first try to increase your bonus)

Correct!

Good job on the first try! This will count for your Understanding Bonus.

Proceed

### Participant Rankings:

| R | S | T | Y |
|---|---|---|---|
| A | A | B | C |
| C | C | A | A |
| D | D | D | B |
| B | B | C | D |

### Prize Priorities:

| A | B | C | D |
|---|---|---|---|
| R | R | S | Y |
| S | S | T | T |
| T | Y | R | S |
| Y | T | Y | R |

reset ↻

---

**Pick prizes to pair →**

|             |     |                                                                                                    |
|-------------|-----|----------------------------------------------------------------------------------------------------|
| R           | A   | <p>R = Ruth</p> <p>S = Shirley</p> <p>T = Theresa</p> <p>Y = You</p> <p><b>U.P.</b> = Unpaired</p> |
| S           | C D |                                                                                                    |
| T           | B   |                                                                                                    |
| Y           |     |                                                                                                    |
| <b>U.P.</b> |     |                                                                                                    |

Allocation Dashboard

# How the Allocation Process Works: Training Round 1/3

Click for a reminder on the technical details of the allocation process

Is the process determining the temporary allocation over?

(Remember: this process is only a first step, after which your Obtainable Prizes are determined, and then the prize you get is determined.)

(Get it right on first try to increase your bonus)

- No
- Yes

Correct! The process is only over when there are no more conflicts.  
Good job on the first try! This will count for your Understanding Bonus.

Proceed

### Participant Rankings:

|   |   |   |   |
|---|---|---|---|
| R | S | T | Y |
| A | A | B | C |
| C | C | A | A |
| D | D | D | B |
| B | B | C | D |

### Prize Priorities:

|   |   |   |   |
|---|---|---|---|
| A | B | C | D |
| R | R | S | Y |
| S | S | T | T |
| T | Y | R | S |
| Y | T | Y | R |

reset ↻

### Pick prizes to pair →

|      |   |   |
|------|---|---|
| R    | A |   |
| S    | C | D |
| T    | B |   |
| Y    |   |   |
| U.P. |   |   |

R = Ruth  
S = Shirley  
T = Theresa  
Y = You  
U.P. = Unpaired

# How the Allocation Process Works: Training Round 1/3

[Click for a reminder on the technical details of the allocation process](#)

Find the next conflict and solve it like before. First, find all participants that are paired to two (or more) prizes. Then, perform the two steps:

- **Unpair:** for each such participant, keep only the prize with the highest rank by that participant paired to her. **Unpair** the other prizes from that participant.
- **Re-pair:** re-pair these prizes to their highest-priority participant, among the participants they were **not yet paired with** and **except for you**.

Hint: You can easily find which participant you should re-pair the unpaired prize to, using the Prize Priorities table: this is the participant right below the one that is currently colored purple under the unpaired prize's name, or, in case that participant is you ("Y"), the one right below "Y".

**Only solve the conflict you see first on this screen!** If new conflicts emerge after solving the current one, wait. You will solve them one-by-one on the next screens.

Click Submit when done.  
(Get it right on first try to increase your bonus)

Correct!  
Good job on the first try! This will count for your Understanding Bonus.

Proceed

### Participant Rankings:

|   |   |   |   |
|---|---|---|---|
| R | S | T | Y |
| A | A | B | C |
| C | C | A | A |
| D | D | D | B |
| B | B | C | D |

### Prize Priorities:

|   |   |   |   |
|---|---|---|---|
| A | B | C | D |
| R | R | S | Y |
| S | S | T | T |
| T | Y | R | S |
| Y | T | Y | R |

reset ↻

---

**Pick prizes to pair →**

|             |                                                                                                                                                                                                                                                                                                                                                   |                                                                                                    |
|-------------|---------------------------------------------------------------------------------------------------------------------------------------------------------------------------------------------------------------------------------------------------------------------------------------------------------------------------------------------------|----------------------------------------------------------------------------------------------------|
| R           | <div style="background-color: purple; color: white; border-radius: 50%; width: 30px; height: 30px; display: flex; align-items: center; justify-content: center;">A</div> <div style="background-color: purple; color: white; border-radius: 50%; width: 30px; height: 30px; display: flex; align-items: center; justify-content: center;">D</div> | <p>R = Ruth</p> <p>S = Shirley</p> <p>T = Theresa</p> <p>Y = You</p> <p><b>U.P.</b> = Unpaired</p> |
| S           | <div style="background-color: purple; color: white; border-radius: 50%; width: 30px; height: 30px; display: flex; align-items: center; justify-content: center;">C</div>                                                                                                                                                                          |                                                                                                    |
| T           | <div style="background-color: purple; color: white; border-radius: 50%; width: 30px; height: 30px; display: flex; align-items: center; justify-content: center;">B</div>                                                                                                                                                                          |                                                                                                    |
| Y           |                                                                                                                                                                                                                                                                                                                                                   |                                                                                                    |
| <b>U.P.</b> |                                                                                                                                                                                                                                                                                                                                                   |                                                                                                    |

# How the Allocation Process Works: Training Round 1/3

Click for a reminder on the technical details of the allocation process

Is the process determining the temporary allocation over?

(Remember: this process is only a first step, after which your Obtainable Prizes are determined, and then the prize you get is determined.)

(Get it right on first try to increase your bonus)

- No
- Yes

Correct! The process is only over when there are no more conflicts.  
Good job on the first try! This will count for your Understanding Bonus.

Proceed

| Participant Rankings: |   |   |   | Prize Priorities: |   |   |   | reset ↻ |
|-----------------------|---|---|---|-------------------|---|---|---|---------|
| R                     | S | T | Y | A                 | B | C | D |         |
| A                     | A | B | C | R                 | R | S | Y |         |
| C                     | C | A | A | S                 | S | T | T |         |
| D                     | D | D | B | T                 | Y | R | S |         |
| B                     | B | C | D | Y                 | T | Y | R |         |

**Pick prizes to pair →**

|      |                                  |                                                                      |
|------|----------------------------------|----------------------------------------------------------------------|
| R    | <input type="text" value="A D"/> | R = Ruth<br>S = Shirley<br>T = Theresa<br>Y = You<br>U.P. = Unpaired |
| S    | <input type="text" value="C"/>   |                                                                      |
| T    | <input type="text" value="B"/>   |                                                                      |
| Y    | <input type="text" value=""/>    |                                                                      |
| U.P. | <input type="text" value=""/>    |                                                                      |

# How the Allocation Process Works: Training Round 1/3

Click for a reminder on the technical details of the allocation process

Find the next conflict and solve it like before. First, find all participants that are paired to two (or more) prizes. Then, perform the two steps:

- **Unpair:** for each such participant, keep only the prize with the highest rank by that participant paired to her. **Unpair** the other prizes from that participant.

**Notice:** at this stage, **Prize D** should be unpaired from Ruth, who has the least priority for getting it. Hence, there are no participants left to re-pair it to, and **it will remain unpaired**. To leave Prize D unpaired, do the following: After clicking on "D" at the **lower** part of the dashboard, click on "+" at the bottom Unpaired ("U.P.") row.

**Only solve the conflict you see first on this screen!** If new conflicts emerge after solving the current one, wait. You will solve them one-by-one on the next screens.

Click Submit when done.

(Get it right on first try to increase your bonus)

Correct!

Good job on the first try! This will count for your Understanding Bonus.

Proceed

### Participant Rankings:

|   |   |   |   |
|---|---|---|---|
| R | S | T | Y |
| A | A | B | C |
| C | C | A | A |
| D | D | D | B |
| B | B | C | D |

### Prize Priorities:

|   |   |   |   |
|---|---|---|---|
| A | B | C | D |
| R | R | S | Y |
| S | S | T | T |
| T | Y | R | S |
| Y | T | Y | R |

---

### Pick prizes to pair →

|             |   |                                                                                                    |
|-------------|---|----------------------------------------------------------------------------------------------------|
| R           | A | <p>R = Ruth</p> <p>S = Shirley</p> <p>T = Theresa</p> <p>Y = You</p> <p><b>U.P.</b> = Unpaired</p> |
| S           | C |                                                                                                    |
| T           | B |                                                                                                    |
| Y           |   |                                                                                                    |
| <b>U.P.</b> | D |                                                                                                    |

Allocation Dashboard

# How the Allocation Process Works: Training Round 1/3

Click for a reminder on the technical details of the allocation process

Is the process determining the temporary allocation over?

(Remember: this process is only a first step, after which your Obtainable Prizes are determined, and then the prize you get is determined.)

(Get it right on first try to increase your bonus)

- No
- Yes

Correct! The process is only over when there are no more conflicts.  
Good job on the first try! This will count for your Understanding Bonus.

Proceed

### Participant Rankings:

|   |   |   |   |
|---|---|---|---|
| R | S | T | Y |
| A | A | B | C |
| C | C | A | A |
| D | D | D | B |
| B | B | C | D |

### Prize Priorities:

|   |   |   |   |
|---|---|---|---|
| A | B | C | D |
| R | R | S | Y |
| S | S | T | T |
| T | Y | R | S |
| Y | T | Y | R |

reset ↻

### Pick prizes to pair →

|      |   |
|------|---|
| R    | A |
| S    | C |
| T    | B |
| Y    |   |
| U.P. | D |

R = Ruth  
S = Shirley  
T = Theresa  
Y = You  
U.P. = Unpaired

# How the Allocation Process Works: Training Round 1/3

Click for a reminder on the technical details of the allocation process

The **temporary** allocation is the following:

- Prize A is temporarily allocated to Ruth.
- Prize B is temporarily allocated to Theresa.
- Prize C is temporarily allocated to Shirley.
- Prize D is temporarily left unpaired.

All participants **except for you** are temporarily matched to prizes.

What about you? Given the temporary allocation, which prizes can you obtain, in principle? In other words, **what are your Obtainable Prizes?**

(Get it right on first try to increase your bonus)

- All four prizes, since I can obtain any prize where the other participant temporarily allocated to that prize does not want it.
- Any prize where my priority is higher than that of the participant who is temporarily allocated the prize.
- Only the prize that was left unpaired in the temporary allocation.
- Any prize where my priority is higher than that of the participant who is temporarily allocated the prize, and the prize that was left unpaired in the temporary allocation.

Correct! The **Obtainable Prizes** are any prize where your priority is higher than that of the participant it is temporarily allocated to, and the prize that was left unpaired in the temporary allocation.

Good job on the first try! This will count for your Understanding Bonus.

Proceed

### Participant Rankings:

| R | S | T | Y |
|---|---|---|---|
| A | A | B | C |
| C | C | A | A |
| D | D | D | B |
| B | B | C | D |

### Prize Priorities:

| A | B | C | D |
|---|---|---|---|
| R | R | S | Y |
| S | S | T | T |
| T | Y | R | S |
| Y | T | Y | R |

---

**Pick prizes to pair** →

|      |   |                                                                                                    |
|------|---|----------------------------------------------------------------------------------------------------|
| R    | A | <p>R = Ruth</p> <p>S = Shirley</p> <p>T = Theresa</p> <p>Y = You</p> <p><b>U.P.</b> = Unpaired</p> |
| S    | C |                                                                                                    |
| T    | B |                                                                                                    |
| Y    |   |                                                                                                    |
| U.P. | D |                                                                                                    |

# How the Allocation Process Works: Training Round 1/3

Click for a reminder on the technical details of the allocation process

## Which of the following is true?

(Get it right on first try to increase your bonus)

- Only the rankings of all participants except for me are used to determine the Obtainable Prizes.
- My own ranking can affect which prizes are Obtainable.
- Only the prize priorities are used to determine the Obtainable Prizes.
- The prize priorities and the rankings of all participants except for me are used to determine the Obtainable Prizes.

Correct! The **Obtainable Prizes** are determined using the prize priorities and the rankings of all participants except for you. Your own ranking cannot influence which prizes are Obtainable.

Good job on the first try! This will count for your Understanding Bonus.

Proceed

### Participant Rankings:

| R | S | T | Y |
|---|---|---|---|
| A | A | B | C |
| C | C | A | A |
| D | D | D | B |
| B | B | C | D |

### Prize Priorities:

| A | B | C | D |
|---|---|---|---|
| R | R | S | Y |
| S | S | T | T |
| T | Y | R | S |
| Y | T | Y | R |

reset ↻

### Pick prizes to pair →

|      |   |
|------|---|
| R    | A |
| S    | C |
| T    | B |
| Y    |   |
| U.P. | D |

R = Ruth  
S = Shirley  
T = Theresa  
Y = You  
U.P. = Unpaired

# How the Allocation Process Works: Training Round 1/3

Click for a reminder on the technical details of the allocation process

Now use this rule to determine your **Obtainable Prizes**.

Note: Now is the first time that your priority for getting the different prizes matters. Remember, it is indicated by the "Y"s in the [Prize Priorities table](#), which are now colored blue.

Choose "Obtainable" or "Unobtainable" next to all the prizes below:

Prize A : (Get it right on first try to increase your bonus)

Unobtainable ▾

Correct! Prize A is temporarily allocated to Ruth, and your priority for getting that prize is **lower** than hers. Hence **you cannot obtain Prize A**.

Good job on the first try! This will count for your Understanding Bonus.

Proceed

### Participant Rankings:

| R | S | T | Y |
|---|---|---|---|
| A | A | B | C |
| C | C | A | A |
| D | D | D | B |
| B | B | C | D |

### Prize Priorities:

| A | B | C | D |
|---|---|---|---|
| R | R | S | Y |
| S | S | T | T |
| T | Y | R | S |
| Y | T | Y | R |

reset ↻

---

**Pick prizes to pair →**

|             |   |                                                                                                    |
|-------------|---|----------------------------------------------------------------------------------------------------|
| R           | A | <p>R = Ruth</p> <p>S = Shirley</p> <p>T = Theresa</p> <p>Y = You</p> <p><b>U.P.</b> = Unpaired</p> |
| S           | C |                                                                                                    |
| T           | B |                                                                                                    |
| Y           |   |                                                                                                    |
| <b>U.P.</b> | D |                                                                                                    |

# How the Allocation Process Works: Training Round 1/3

Click for a reminder on the technical details of the allocation process

Now use this rule to determine your **Obtainable Prizes**.

Note: Now is the first time that your priority for getting the different prizes matters. Remember, it is indicated by the "Y"s in the Prize Priorities table, which are now colored blue.

Choose "Obtainable" or "Unobtainable" next to all the prizes below:

Prize B : (Get it right on first try to increase your bonus)

Obtainable

Correct! Prize B is temporarily allocated to Theresa, but your priority for getting that prize is **higher** than hers. Hence **you can obtain Prize B**.

Good job on the first try! This will count for your Understanding Bonus.

Proceed

### Participant Rankings:

| R | S | T | Y |
|---|---|---|---|
| A | A | B | C |
| C | C | A | A |
| D | D | D | B |
| B | B | C | D |

### Prize Priorities:

| A | B | C | D |
|---|---|---|---|
| R | R | S | Y |
| S | S | T | T |
| T | Y | R | S |
| Y | T | Y | R |

---

**Pick prizes to pair →**

|      |   |  |
|------|---|--|
| R    | A |  |
| S    | C |  |
| T    | B |  |
| Y    |   |  |
| U.P. | D |  |

R = Ruth

S = Shirley

T = Theresa

Y = You

U.P. = Unpaired

# How the Allocation Process Works: Training Round 1/3

Click for a reminder on the technical details of the allocation process

Now use this rule to determine your **Obtainable Prizes**.

Note: Now is the first time that your priority for getting the different prizes matters. Remember, it is indicated by the "Y"s in the Prize Priorities table, which are now colored blue.

Choose "Obtainable" or "Unobtainable" next to all the prizes below:

Prize C : (Get it right on first try to increase your bonus)

Unobtainable ▾

Correct! Prize C is temporarily allocated to Shirley, and your priority for getting that prize is lower than hers. Hence **you cannot obtain Prize C**.

Good job on the first try! This will count for your Understanding Bonus.

Proceed

### Participant Rankings:

| R | S | T | Y |
|---|---|---|---|
| A | A | B | C |
| C | C | A | A |
| D | D | D | B |
| B | B | C | D |

### Prize Priorities:

| A | B | C | D |
|---|---|---|---|
| R | R | S | Y |
| S | S | T | T |
| T | Y | R | S |
| Y | T | Y | R |

reset ↻

---

**Pick prizes to pair →**

|      |   |  |
|------|---|--|
| R    | A |  |
| S    | C |  |
| T    | B |  |
| Y    |   |  |
| U.P. | D |  |

**R** = Ruth

**S** = Shirley

**T** = Theresa

**Y** = You

**U.P.** = Unpaired

# How the Allocation Process Works: Training Round 1/3

Click for a reminder on the technical details of the allocation process

Now use this rule to determine your **Obtainable Prizes**.

Note: Now is the first time that your priority for getting the different prizes matters. Remember, it is indicated by the "Y"s in the Prize Priorities table, which are now colored blue.

Choose "Obtainable" or "Unobtainable" next to all the prizes below:

Prize D : (Get it right on first try to increase your bonus)

Obtainable

Correct! Prize D was left unpaired in the temporary allocation. Hence **you can obtain Prize D**.  
 Good job on the first try! This will count for your Understanding Bonus.

Proceed

### Participant Rankings:

|   |   |   |   |
|---|---|---|---|
| R | S | T | Y |
| A | A | B | C |
| C | C | A | A |
| D | D | D | B |
| B | B | C | D |

### Prize Priorities:

|   |   |   |   |
|---|---|---|---|
| A | B | C | D |
| R | R | S | Y |
| S | S | T | T |
| T | Y | R | S |
| Y | T | Y | R |

---

**Pick prizes to pair →**

|      |   |  |
|------|---|--|
| R    | A |  |
| S    | C |  |
| T    | B |  |
| Y    |   |  |
| U.P. | D |  |

R = Ruth

S = Shirley

T = Theresa

Y = You

**U.P.** = Unpaired

Allocation Dashboard

# How the Allocation Process Works: Training Round 1/3

Click for a reminder on the technical details of the allocation process

Your **Obtainable Prizes** are:

**Prize B and Prize D**

Among these Obtainable Prizes, which prize do **you actually get?**

(Get it right on first try to increase your bonus)

- The prize that was left unpaired in the temporary allocation.
- The prize that other participants placed last in rankings on average.
- The prize that I ranked the highest.
- The prize which I have the highest priority for getting.

Correct! Among the **Obtainable Prizes**, you get the one that you ranked the highest.

Good job on the first try! This will count for your Understanding Bonus.

Proceed

### Participant Rankings:

| R | S | T | Y |
|---|---|---|---|
| A | A | B | C |
| C | C | A | A |
| D | D | D | B |
| B | B | C | D |

### Prize Priorities:

| A | B | C | D |
|---|---|---|---|
| R | R | S | Y |
| S | S | T | T |
| T | Y | R | S |
| Y | T | Y | R |

reset ↻

### Pick prizes to pair →

|      |   |
|------|---|
| R    | A |
| S    | C |
| T    | B |
| Y    |   |
| U.P. | D |

R = Ruth  
S = Shirley  
T = Theresa  
Y = You  
U.P. = Unpaired

# How the Allocation Process Works: Training Round 1/3

Click for a reminder on the technical details of the allocation process

Your **Obtainable Prizes** are:

**Prize B and Prize D**

Now, your ranking is used to determine which of the Obtainable Prizes you actually get. Out of these **Obtainable Prizes**, select the prize **you ("Y") ranked the highest** from the list below. This is the prize you get.

Note: Now is the first (and only) time that **your own ranking matters!** Remember, it is indicated by the "Y" column in the Participant Rankings table, which is now colored in blue.

(Get it right on first try to increase your bonus)

Correct!

Good job on the first try! This will count for your Understanding Bonus.

Proceed

### Participant Rankings:

| R | S | T | Y |
|---|---|---|---|
| A | A | B | C |
| C | C | A | A |
| D | D | D | B |
| B | B | C | D |

### Prize Priorities:

| A | B | C | D |
|---|---|---|---|
| R | R | S | Y |
| S | S | T | T |
| T | Y | R | S |
| Y | T | Y | R |

reset ↻

### Pick prizes to pair →

|      |   |
|------|---|
| R    | A |
| S    | C |
| T    | B |
| Y    |   |
| U.P. | D |

R = Ruth  
S = Shirley  
T = Theresa  
Y = You  
U.P. = Unpaired

# How the Allocation Process Works: Training Round 1/3

Click for a reminder on the technical details of the allocation process

The allocation process is over. **You get Prize B.**

Proceed

| Participant Rankings: |   |   |   | Prize Priorities: |   |   |   | reset ↻ |
|-----------------------|---|---|---|-------------------|---|---|---|---------|
| R                     | S | T | Y | A                 | B | C | D |         |
| A                     | A | B | C | R                 | R | S | Y |         |
| C                     | C | A | A | S                 | S | T | T |         |
| D                     | D | D | B | T                 | Y | R | S |         |
| B                     | B | C | D | Y                 | T | Y | R |         |

**Pick prizes to pair →**

|      |   |
|------|---|
| R    | A |
| S    | C |
| T    | B |
| Y    |   |
| U.P. | D |

**R** = Ruth  
**S** = Shirley  
**T** = Theresa  
**Y** = You  
**U.P.** = Unpaired

Allocation Dashboard

### D.3.2.2 Menu DA Mechanics: Training Round 2

## How the Allocation Process Works: Training Round 2/3

[Click for a general reminder on this study](#)

[Click for a reminder on the technical details of the allocation process](#)

*This is a training round.*

*Everything is **the same** as in the real rounds you will play later on, except that you will **not** earn the money worth of the prize you will get. Instead, we will ask you questions which can count for your **Understanding Bonus** at the end of the study.*

*Remember: each question increases your Understanding Bonus only if you answer it correctly on your first attempt. Think about your answers carefully!*

### Step 1: Round Information

In this round, the **prizes** are:

| Prize       | A                                           | B | C | D |
|-------------|---------------------------------------------|---|---|---|
| Money worth | - Training round. No earnings from prizes - |   |   |   |

[Click for a reminder on what the prizes mean](#)

The **prize priorities** for you and for the other participants are:

| Prize                  | A       | B       | C       | D       |
|------------------------|---------|---------|---------|---------|
| 1st priority (highest) | Shirley | Shirley | Theresa | Theresa |
| 2nd priority           | You     | Theresa | You     | Ruth    |
| 3rd priority           | Ruth    | You     | Ruth    | You     |
| 4th priority (lowest)  | Theresa | Ruth    | Shirley | Shirley |

Click for a reminder on what the priorities mean

## Step 2: Submit Your Ranking

Click for a reminder on what this ranking means

Please rank the four prizes **in the fixed, specific order D-C-B-A**.

**D-C-B-A**

## Step 3: Allocation Process

You are going to perform the allocation process by yourself, according to what you learned.  
Click on the button below to start.

Proceed

# How the Allocation Process Works: Training Round 2/3

Click for a reminder on the technical details of the allocation process

In this training round, you will perform the allocation process by yourself, instead of the computer performing it.

Each step or question will count for your Understanding Bonus, so think about your answers carefully!

Proceed

| Participant Rankings: |  |          |  | Prize Priorities: |  |          |  | reset ↻  |  |          |  |          |  |          |
|-----------------------|--|----------|--|-------------------|--|----------|--|----------|--|----------|--|----------|--|----------|
| <b>R</b>              |  | <b>S</b> |  | <b>T</b>          |  | <b>Y</b> |  | <b>A</b> |  | <b>B</b> |  | <b>C</b> |  | <b>D</b> |
| D                     |  | B        |  | B                 |  | D        |  | S        |  | S        |  | T        |  | T        |
| A                     |  | A        |  | C                 |  | C        |  | Y        |  | T        |  | Y        |  | R        |
| B                     |  | C        |  | D                 |  | B        |  | R        |  | Y        |  | R        |  | Y        |
| C                     |  | D        |  | A                 |  | A        |  | T        |  | R        |  | S        |  | S        |

**Pick prizes to pair →** A B C D

|             |                      |                                                                                                         |
|-------------|----------------------|---------------------------------------------------------------------------------------------------------|
| <b>R</b>    | <input type="text"/> | <b>R</b> = Ruth<br><b>S</b> = Shirley<br><b>T</b> = Theresa<br><b>Y</b> = You<br><b>U.P.</b> = Unpaired |
| <b>S</b>    | <input type="text"/> |                                                                                                         |
| <b>T</b>    | <input type="text"/> |                                                                                                         |
| <b>Y</b>    | <input type="text"/> |                                                                                                         |
| <b>U.P.</b> | <input type="text"/> |                                                                                                         |

Allocation Dashboard

# How the Allocation Process Works: Training Round 2/3

Click for a reminder on the technical details of the allocation process

First, find the **temporary allocation** of prizes to all participants **except for you** using the Allocation Dashboard below. Use the multi-step process you learned.

**Note:** In this round, you should only submit once you find the **final temporary allocation**. Do **not** separately submit steps of the process like in Training Round 1.

In case you are still not sure how to find the allocation by yourself, click on the button below to watch a helpful video explaining all the steps. Clicking on the video will pause/unpause it, and if you close and re-open the video, it will continue from the same point.

Click here for a video with step-by-step explanations

(To restart the video, please refresh the page)

Click Submit when you are done.

(Get it right on first try to increase your bonus; it will count as **5 questions**.)

If you only get it right on the second try it will still count for your bonus; it will count as **2 questions**.)

Correct temporary allocation!

Good job on the first try! This will count as **5 questions** for your Understanding Bonus.

Proceed

### Participant Rankings:

| R | S | T | Y |
|---|---|---|---|
| D | B | B | D |
| A | A | C | C |
| B | C | D | B |
| C | D | A | A |

### Prize Priorities:

| A | B | C | D |
|---|---|---|---|
| S | S | T | T |
| Y | T | Y | R |
| R | Y | R | Y |
| T | R | S | S |

---

**Pick prizes to pair →**

|      |   |  |
|------|---|--|
| R    | D |  |
| S    | B |  |
| T    | C |  |
| Y    |   |  |
| U.P. | A |  |

R = Ruth  
 S = Shirley  
 T = Theresa  
 Y = You  
 U.P. = Unpaired

# How the Allocation Process Works: Training Round 2/3

Click for a reminder on the technical details of the allocation process

Next, find your **Obtainable Prizes**. For each of the four prizes below, choose "Obtainable" or "Unobtainable," based on what you learned in the previous screens.

Click Submit when you are done.

(Get it right on first try to increase your bonus)

|                                         |                                           |                                           |                                           |
|-----------------------------------------|-------------------------------------------|-------------------------------------------|-------------------------------------------|
| Prize A                                 | Prize B                                   | Prize C                                   | Prize D                                   |
| <input type="text" value="Obtainable"/> | <input type="text" value="Unobtainable"/> | <input type="text" value="Unobtainable"/> | <input type="text" value="Unobtainable"/> |

Correct! The **Obtainable Prizes** are any prize where your priority is higher than that of the participant it is temporarily allocated to, and the prize that was left unpaired in the temporary allocation.

Good job on the first try! This will count for your Understanding Bonus.

Proceed

### Participant Rankings:

|   |   |   |   |
|---|---|---|---|
| R | S | T | Y |
| D | B | B | D |
| A | A | C | C |
| B | C | D | B |
| C | D | A | A |

### Prize Priorities:

|   |   |   |   |
|---|---|---|---|
| A | B | C | D |
| S | S | T | T |
| Y | T | Y | R |
| R | Y | R | Y |
| T | R | S | S |

---

**Pick prizes to pair →**

|      |                                |                                                                                                         |
|------|--------------------------------|---------------------------------------------------------------------------------------------------------|
| R    | <input type="text" value="D"/> | <b>R</b> = Ruth<br><b>S</b> = Shirley<br><b>T</b> = Theresa<br><b>Y</b> = You<br><b>U.P.</b> = Unpaired |
| S    | <input type="text" value="B"/> |                                                                                                         |
| T    | <input type="text" value="C"/> |                                                                                                         |
| Y    | <input type="text"/>           |                                                                                                         |
| U.P. | <input type="text" value="A"/> |                                                                                                         |

# How the Allocation Process Works: Training Round 2/3

Click for a reminder on the technical details of the allocation process

Your **Obtainable Prizes** are:

**Prize A**

Finally, select **the prize that you get** out of the Obtainable Prizes from the list below.

A ▾

Correct! Among the **Obtainable Prizes**, Prize A is the one you **ranked highest**. Hence you get this prize.  
Good job on the first try! This will count for your Understanding Bonus.

Proceed

### Participant Rankings:

|   |   |   |   |
|---|---|---|---|
| R | S | T | Y |
| D | B | B | D |
| A | A | C | C |
| B | C | D | B |
| C | D | A | A |

### Prize Priorities:

|   |   |   |   |
|---|---|---|---|
| A | B | C | D |
| S | S | T | T |
| Y | T | Y | R |
| R | Y | R | Y |
| T | R | S | S |

reset ↻

### Pick prizes to pair →

|      |   |
|------|---|
| R    | D |
| S    | B |
| T    | C |
| Y    |   |
| U.P. | A |

R = Ruth  
S = Shirley  
T = Theresa  
Y = You  
U.P. = Unpaired

# How the Allocation Process Works: Training Round 2/3

Click for a reminder on the technical details of the allocation process

The allocation process is over. **You get Prize A.**

Proceed

| Participant Rankings:                                                                                                                                                                                                                                                | Prize Priorities:              | reset ↻                                                                                                 |   |   |   |   |   |   |   |   |   |   |   |   |   |   |   |   |   |   |                                                                                                                                                                                                                                                                      |   |   |   |   |   |   |   |   |   |   |   |   |   |   |   |   |   |   |   |   |  |
|----------------------------------------------------------------------------------------------------------------------------------------------------------------------------------------------------------------------------------------------------------------------|--------------------------------|---------------------------------------------------------------------------------------------------------|---|---|---|---|---|---|---|---|---|---|---|---|---|---|---|---|---|---|----------------------------------------------------------------------------------------------------------------------------------------------------------------------------------------------------------------------------------------------------------------------|---|---|---|---|---|---|---|---|---|---|---|---|---|---|---|---|---|---|---|---|--|
| <table><tr><td>R</td><td>S</td><td>T</td><td>Y</td></tr><tr><td>D</td><td>B</td><td>B</td><td>D</td></tr><tr><td>A</td><td>A</td><td>C</td><td>C</td></tr><tr><td>B</td><td>C</td><td>D</td><td>B</td></tr><tr><td>C</td><td>D</td><td>A</td><td>A</td></tr></table> | R                              | S                                                                                                       | T | Y | D | B | B | D | A | A | C | C | B | C | D | B | C | D | A | A | <table><tr><td>A</td><td>B</td><td>C</td><td>D</td></tr><tr><td>S</td><td>S</td><td>T</td><td>T</td></tr><tr><td>Y</td><td>T</td><td>Y</td><td>R</td></tr><tr><td>R</td><td>Y</td><td>R</td><td>Y</td></tr><tr><td>T</td><td>R</td><td>S</td><td>S</td></tr></table> | A | B | C | D | S | S | T | T | Y | T | Y | R | R | Y | R | Y | T | R | S | S |  |
| R                                                                                                                                                                                                                                                                    | S                              | T                                                                                                       | Y |   |   |   |   |   |   |   |   |   |   |   |   |   |   |   |   |   |                                                                                                                                                                                                                                                                      |   |   |   |   |   |   |   |   |   |   |   |   |   |   |   |   |   |   |   |   |  |
| D                                                                                                                                                                                                                                                                    | B                              | B                                                                                                       | D |   |   |   |   |   |   |   |   |   |   |   |   |   |   |   |   |   |                                                                                                                                                                                                                                                                      |   |   |   |   |   |   |   |   |   |   |   |   |   |   |   |   |   |   |   |   |  |
| A                                                                                                                                                                                                                                                                    | A                              | C                                                                                                       | C |   |   |   |   |   |   |   |   |   |   |   |   |   |   |   |   |   |                                                                                                                                                                                                                                                                      |   |   |   |   |   |   |   |   |   |   |   |   |   |   |   |   |   |   |   |   |  |
| B                                                                                                                                                                                                                                                                    | C                              | D                                                                                                       | B |   |   |   |   |   |   |   |   |   |   |   |   |   |   |   |   |   |                                                                                                                                                                                                                                                                      |   |   |   |   |   |   |   |   |   |   |   |   |   |   |   |   |   |   |   |   |  |
| C                                                                                                                                                                                                                                                                    | D                              | A                                                                                                       | A |   |   |   |   |   |   |   |   |   |   |   |   |   |   |   |   |   |                                                                                                                                                                                                                                                                      |   |   |   |   |   |   |   |   |   |   |   |   |   |   |   |   |   |   |   |   |  |
| A                                                                                                                                                                                                                                                                    | B                              | C                                                                                                       | D |   |   |   |   |   |   |   |   |   |   |   |   |   |   |   |   |   |                                                                                                                                                                                                                                                                      |   |   |   |   |   |   |   |   |   |   |   |   |   |   |   |   |   |   |   |   |  |
| S                                                                                                                                                                                                                                                                    | S                              | T                                                                                                       | T |   |   |   |   |   |   |   |   |   |   |   |   |   |   |   |   |   |                                                                                                                                                                                                                                                                      |   |   |   |   |   |   |   |   |   |   |   |   |   |   |   |   |   |   |   |   |  |
| Y                                                                                                                                                                                                                                                                    | T                              | Y                                                                                                       | R |   |   |   |   |   |   |   |   |   |   |   |   |   |   |   |   |   |                                                                                                                                                                                                                                                                      |   |   |   |   |   |   |   |   |   |   |   |   |   |   |   |   |   |   |   |   |  |
| R                                                                                                                                                                                                                                                                    | Y                              | R                                                                                                       | Y |   |   |   |   |   |   |   |   |   |   |   |   |   |   |   |   |   |                                                                                                                                                                                                                                                                      |   |   |   |   |   |   |   |   |   |   |   |   |   |   |   |   |   |   |   |   |  |
| T                                                                                                                                                                                                                                                                    | R                              | S                                                                                                       | S |   |   |   |   |   |   |   |   |   |   |   |   |   |   |   |   |   |                                                                                                                                                                                                                                                                      |   |   |   |   |   |   |   |   |   |   |   |   |   |   |   |   |   |   |   |   |  |
| <b>Pick prizes to pair →</b>                                                                                                                                                                                                                                         |                                |                                                                                                         |   |   |   |   |   |   |   |   |   |   |   |   |   |   |   |   |   |   |                                                                                                                                                                                                                                                                      |   |   |   |   |   |   |   |   |   |   |   |   |   |   |   |   |   |   |   |   |  |
| R                                                                                                                                                                                                                                                                    | <input type="text" value="D"/> | <b>R</b> = Ruth<br><b>S</b> = Shirley<br><b>T</b> = Theresa<br><b>Y</b> = You<br><b>U.P.</b> = Unpaired |   |   |   |   |   |   |   |   |   |   |   |   |   |   |   |   |   |   |                                                                                                                                                                                                                                                                      |   |   |   |   |   |   |   |   |   |   |   |   |   |   |   |   |   |   |   |   |  |
| S                                                                                                                                                                                                                                                                    | <input type="text" value="B"/> |                                                                                                         |   |   |   |   |   |   |   |   |   |   |   |   |   |   |   |   |   |   |                                                                                                                                                                                                                                                                      |   |   |   |   |   |   |   |   |   |   |   |   |   |   |   |   |   |   |   |   |  |
| T                                                                                                                                                                                                                                                                    | <input type="text" value="C"/> |                                                                                                         |   |   |   |   |   |   |   |   |   |   |   |   |   |   |   |   |   |   |                                                                                                                                                                                                                                                                      |   |   |   |   |   |   |   |   |   |   |   |   |   |   |   |   |   |   |   |   |  |
| Y                                                                                                                                                                                                                                                                    | <input type="text" value=""/>  |                                                                                                         |   |   |   |   |   |   |   |   |   |   |   |   |   |   |   |   |   |   |                                                                                                                                                                                                                                                                      |   |   |   |   |   |   |   |   |   |   |   |   |   |   |   |   |   |   |   |   |  |
| U.P.                                                                                                                                                                                                                                                                 | <input type="text" value="A"/> |                                                                                                         |   |   |   |   |   |   |   |   |   |   |   |   |   |   |   |   |   |   |                                                                                                                                                                                                                                                                      |   |   |   |   |   |   |   |   |   |   |   |   |   |   |   |   |   |   |   |   |  |

Allocation Dashboard

### D.3.2.3 Menu DA Mechanics: Training Round 3

## How the Allocation Process Works: Training Round 3/3

[Click for a general reminder on this study](#)

[Click for a reminder on the technical details of the allocation process](#)

*This is a training round.*

*Everything is **the same** as in the real rounds you will play later on, except that you will **not** earn the money worth of the prize you will get. Instead, we will ask you questions which can count for your **Understanding Bonus** at the end of the study.*

*Remember: each question increases your Understanding Bonus only if you answer it correctly on your first attempt. Think about your answers carefully!*

### Step 1: Round Information

In this round, the **prizes** are:

| Prize       | A                                           | B | C | D |
|-------------|---------------------------------------------|---|---|---|
| Money worth | - Training round. No earnings from prizes - |   |   |   |

[Click for a reminder on what the prizes mean](#)

The **prize priorities** for you and for the other participants are:

| Prize                  | A       | B       | C       | D       |
|------------------------|---------|---------|---------|---------|
| 1st priority (highest) | You     | Ruth    | Shirley | Ruth    |
| 2nd priority           | Theresa | You     | Ruth    | You     |
| 3rd priority           | Shirley | Theresa | Theresa | Shirley |
| 4th priority (lowest)  | Ruth    | Shirley | You     | Theresa |

Click for a reminder on what the priorities mean

## Step 2: Submit Your Ranking

Click for a reminder on what this ranking means

Please rank the four prizes **in the fixed, specific order D-B-C-A**.

**D-B-C-A**

## Step 3: Allocation Process

You are going to perform the allocation process by yourself, according to what you learned.  
Click on the button below to start.

Proceed

---

# How the Allocation Process Works: Training Round 3/3

Click for a reminder on the technical details of the allocation process

In this training round, you will perform the allocation process by yourself, instead of the computer performing it.

Each step or question will count for your Understanding Bonus, so think about your answers carefully!

Proceed

| Participant Rankings: |  |          |  | Prize Priorities: |  |          |  | reset ↻  |  |          |  |          |  |          |
|-----------------------|--|----------|--|-------------------|--|----------|--|----------|--|----------|--|----------|--|----------|
| <b>R</b>              |  | <b>S</b> |  | <b>T</b>          |  | <b>Y</b> |  | <b>A</b> |  | <b>B</b> |  | <b>C</b> |  | <b>D</b> |
| A                     |  | B        |  | D                 |  | D        |  | Y        |  | R        |  | S        |  | R        |
| B                     |  | A        |  | B                 |  | B        |  | T        |  | Y        |  | R        |  | Y        |
| D                     |  | D        |  | A                 |  | C        |  | S        |  | T        |  | T        |  | S        |
| C                     |  | C        |  | C                 |  | A        |  | R        |  | S        |  | Y        |  | T        |

**Pick prizes to pair** → A B C D

|             |                      |                                                                                                         |
|-------------|----------------------|---------------------------------------------------------------------------------------------------------|
| <b>R</b>    | <input type="text"/> | <b>R</b> = Ruth<br><b>S</b> = Shirley<br><b>T</b> = Theresa<br><b>Y</b> = You<br><b>U.P.</b> = Unpaired |
| <b>S</b>    | <input type="text"/> |                                                                                                         |
| <b>T</b>    | <input type="text"/> |                                                                                                         |
| <b>Y</b>    | <input type="text"/> |                                                                                                         |
| <b>U.P.</b> | <input type="text"/> |                                                                                                         |

Allocation Dashboard

# How the Allocation Process Works: Training Round 3/3

Click for a reminder on the technical details of the allocation process

First, find the **temporary allocation** of prizes to all participants **except for you** using the Allocation Dashboard below. Use the multi-step process you learned.

Note: In this round, you should only submit once you find the **final temporary allocation**. Do **not** separately submit steps of the process like in Training Round 1.

Click Submit when you are done.

(Get it right on first try to increase your bonus; it will count as **5 questions**.)

If you only get it right on the second try it will still count for your bonus; it will count as **2 questions**.)

Correct temporary allocation!

Good job on the first try! This will count as **5 questions** for your Understanding Bonus.

Proceed

### Participant Rankings:

|   |   |   |   |
|---|---|---|---|
| R | S | T | Y |
| A | B | D | D |
| B | A | B | B |
| D | D | A | C |
| C | C | C | A |

### Prize Priorities:

|   |   |   |   |
|---|---|---|---|
| A | B | C | D |
| Y | R | S | R |
| T | Y | R | Y |
| S | T | T | S |
| R | S | Y | T |

reset ↻

---

### Pick prizes to pair →

|      |   |
|------|---|
| R    | B |
| S    | D |
| T    | A |
| Y    |   |
| U.P. | C |

**R** = Ruth

**S** = Shirley

**T** = Theresa

**Y** = You

**U.P.** = Unpaired

# How the Allocation Process Works: Training Round 3/3

Click for a reminder on the technical details of the allocation process

Next, find your **Obtainable Prizes**. For each of the four prizes below, choose "Obtainable" or "Unobtainable," based on what you learned in the previous screens.

Click Submit when you are done.  
(Get it right on first try to increase your bonus)

|                                         |                                           |                                         |                                         |
|-----------------------------------------|-------------------------------------------|-----------------------------------------|-----------------------------------------|
| Prize A                                 | Prize B                                   | Prize C                                 | Prize D                                 |
| <input type="text" value="Obtainable"/> | <input type="text" value="Unobtainable"/> | <input type="text" value="Obtainable"/> | <input type="text" value="Obtainable"/> |

Correct! The **Obtainable Prizes** are any prize where your priority is higher than that of the participant it is temporarily allocated to, and the prize that was left unpaired in the temporary allocation.

Proceed

### Participant Rankings:

|          |          |          |   |
|----------|----------|----------|---|
| R        | S        | T        | Y |
| A        | B        | D        | D |
| <b>B</b> | A        | B        | B |
| D        | <b>D</b> | <b>A</b> | C |
| C        | C        | C        | A |

### Prize Priorities:

|          |          |          |          |
|----------|----------|----------|----------|
| A        | B        | C        | D        |
| <b>Y</b> | <b>R</b> | S        | R        |
| <b>T</b> | <b>Y</b> | R        | <b>Y</b> |
| S        | T        | T        | <b>S</b> |
| R        | S        | <b>Y</b> | T        |

---

**Pick prizes to pair →**

|             |          |                                                                                                                                |
|-------------|----------|--------------------------------------------------------------------------------------------------------------------------------|
| R           | <b>B</b> | <p><b>R</b> = Ruth</p> <p><b>S</b> = Shirley</p> <p><b>T</b> = Theresa</p> <p><b>Y</b> = You</p> <p><b>U.P.</b> = Unpaired</p> |
| S           | <b>D</b> |                                                                                                                                |
| T           | <b>A</b> |                                                                                                                                |
| Y           |          |                                                                                                                                |
| <b>U.P.</b> | <b>C</b> |                                                                                                                                |

# How the Allocation Process Works: Training Round 3/3

Click for a reminder on the technical details of the allocation process

Your **Obtainable Prizes** are:

**Prize A, Prize C and Prize D**

Finally, select **the prize that you get** out of the Obtainable Prizes from the list below.

Correct! Among the **Obtainable Prizes**, Prize D is the one you **ranked highest**. Hence you get this prize.  
Good job on the first try! This will count for your Understanding Bonus.

Proceed

### Participant Rankings:

|   |   |   |   |
|---|---|---|---|
| R | S | T | Y |
| A | B | D | D |
| B | A | B | B |
| D | D | A | C |
| C | C | C | A |

### Prize Priorities:

|   |   |   |   |
|---|---|---|---|
| A | B | C | D |
| Y | R | S | R |
| T | Y | R | Y |
| S | T | T | S |
| R | S | Y | T |

reset ↻

### Pick prizes to pair →

|      |   |
|------|---|
| R    | B |
| S    | D |
| T    | A |
| Y    |   |
| U.P. | C |

R = Ruth  
S = Shirley  
T = Theresa  
Y = You  
U.P. = Unpaired

# How the Allocation Process Works: Training Round 3/3

Click for a reminder on the technical details of the allocation process

The allocation process is over. **You get Prize D.**

Proceed

### Participant Rankings:

|   |   |   |   |
|---|---|---|---|
| R | S | T | Y |
| A | B | D | D |
| B | A | B | B |
| D | D | A | C |
| C | C | C | A |

### Prize Priorities:

|   |   |   |   |
|---|---|---|---|
| A | B | C | D |
| Y | R | S | R |
| T | Y | R | Y |
| S | T | T | S |
| R | S | Y | T |

reset ↻

### Pick prizes to pair →

|      |   |
|------|---|
| R    | B |
| S    | D |
| T    | A |
| Y    |   |
| U.P. | C |

**R** = Ruth  
**S** = Shirley  
**T** = Theresa  
**Y** = You  
**U.P.** = Unpaired

Allocation Dashboard

### D.3.3.0 Menu SP Property Description

## The Key Principle of Your Ranking

*We will now tell you a general important principle of how your own ranking affects the allocation process.*

***This principle is important to learn:*** *You may be able to apply your knowledge of it to choose your rankings in the upcoming real rounds of this study.*

*The prize you get is determined using an allocation process with two main steps:*

- 1. The computer determines some group of **Obtainable Prizes** that you might receive. Your own ranking does not influence the Obtainable Prizes. Instead, they are determined using only the prize priorities and the rankings of the other participants.*
- 2. You get the Obtainable Prize that you **ranked highest** (in the ranking you submitted).*

***The important principle:*** *Your own ranking does **not** influence what the Obtainable Prizes are, but it **does** determine what you get from among the Obtainable Prizes—you get the Obtainable Prize that you ranked the **highest**.*

*The following image illustrates how your own ranking, the rankings of the other participants and the prize priorities affect the prize you get:*

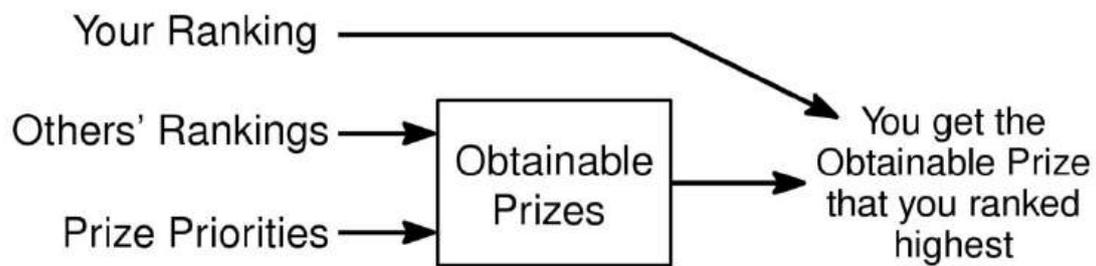

*For example, imagine that your Obtainable Prizes are C and D. If you submit the ranking A–B–C–D, you will get Prize C, which is the one you ranked highest among the Obtainable Prizes. No ranking you could possibly submit would get you Prize A or Prize B, since the Obtainable Prizes are C and D, and since your own ranking cannot influence the Obtainable Prizes.*

*On the next screens you will play training rounds of the game to master your understanding of this principle. Click the button below to proceed to these rounds.*

[Proceed to training rounds](#)

### D.3.3.1 Menu SP Property: Training Round 1

## The Key Principle of Your Ranking: Training Round 1/3

[Click for a general reminder on this study](#)

[Click for a reminder on the Key Principle of your ranking](#)

*This is a training round.*

*Everything is **the same** as in the real rounds you will play later on, except that you will **not** earn the money worth of the prize you will get. Instead, we will ask you questions which can count for your **Understanding Bonus** at the end of the study.*

*Remember: each question increases your Understanding Bonus only if you answer it correctly on your first attempt. Think about your answers carefully!*

### Step 1: Round Information

In this round, the **prizes** are:

| Prize       | A                                           | B | C | D |
|-------------|---------------------------------------------|---|---|---|
| Money worth | - Training round. No earnings from prizes - |   |   |   |

[Click for a reminder on what the prizes mean](#)

The **prize priorities** for you and for the other participants are:

| Prize                  | A       | B       | C       | D       |
|------------------------|---------|---------|---------|---------|
| 1st priority (highest) | Shirley | Shirley | Theresa | You     |
| 2nd priority           | Theresa | You     | Shirley | Theresa |
| 3rd priority           | You     | Theresa | You     | Ruth    |
| 4th priority (lowest)  | Ruth    | Ruth    | Ruth    | Shirley |

Click for a reminder on what the priorities mean

## Step 2: Submit Your Ranking

Click for a reminder on what this ranking means

Please rank the four prizes **in the fixed, specific order C-B-A-D**.

**C-B-A-D**

## Step 3: Allocation Process

**You get Prize A.**

*In this training round, you will answer a few questions about the Key Principle of your ranking and about this round's outcome. Remember: each question will count for your Understanding Bonus only if you answer it correctly on your first attempt. Think about your answers carefully!*

In all the following questions, imagine the computer has already determined some prize priorities and rankings of the other, computerized participants, so that the only component left undecided is your own ranking.

Please determine whether the following statements are true or false:

The allocation process first determines the Obtainable Prizes, which I **cannot affect with my own ranking**. Then, I always get the Obtainable Prize that is **placed highest in the ranking I submitted**. (Get it right on first try to increase your bonus)

- True  
 False

**Correct!** In the allocation process, the group of Obtainable Prizes that you might receive is determined using only the other participants' rankings and the prize priorities. Then, from among the Obtainable Prizes, you get the one that you ranked highest.

**Good job on the first try! This will count for your Understanding Bonus.**

Submitting some ranking **cannot** ensure that I will get the **highest-rank** prize in that ranking, but it **does** ensure that I will **not** get the **lowest-rank** prize in that ranking.

(Get it right on first try to increase your bonus)

- True  
 False

Correct! The allocation process only ensures that **out of the Obtainable Prizes** (which you cannot affect with your own ranking), you get the one that you ranked highest. On some occasions, the **prize you ranked lowest may be the only Obtainable Prize** and hence you would get it.

Good job on the first try! This will count for your Understanding Bonus.

Imagine I have a low priority for getting Prize A, which is the prize I want the most, but I have a high priority for getting Prize B, which I want the second most. Then, submitting a ranking that places Prize A first and Prize B second may lead to missing out on both prizes A and B, while submitting a different ranking could have gotten me Prize B.

(Get it right on first try to increase your bonus)

- True  
 False

Correct! Imagine submitting a ranking that places Prize A first and Prize B second, but getting some prize other than Prize A or Prize B. This means that both Prize A and Prize B are **non-Obtainable**. Remember that submitting different, alternative rankings would have no effect on your Obtainable Prizes, and cannot get you neither of these prizes. Hence, no alternative ranking can get you Prize A or Prize B. This is true **regardless of your specific priorities for getting these prizes**.

Good job on the first try! This will count for your Understanding Bonus.

Please answer the following question:

**Remember: You submitted the ranking C–B–A–D, and ended up getting Prize A.** Imagine you had instead submitted a different ranking (while all prize priorities and other participants' rankings remained the same). Which of the following is true? (select one answer)

(Hint: think about what the set of Obtainable Prizes could possibly be.)

(Get it right on first try to increase your bonus)

- It is certain that every possible ranking I could have submitted would have gotten me Prize A.  
 There might be some alternative ranking I could have submitted that would have gotten me Prize B.  
 There might be some alternative ranking I could have submitted that would have gotten me Prize C.  
 There might be some alternative ranking I could have submitted that would have gotten me Prize D.

Correct! You always get your highest-ranked Obtainable Prize, in this case, Prize A. If your Obtainable Prizes included Prize C and/or Prize B, which you ranked higher than Prize A, you would have gotten one of them instead. Thus, the Obtainable Prizes can only include Prize A, and possibly Prize D, but **do not** include Prize C nor Prize B. Your ranking does not affect your Obtainable Prizes, so submitting a different ranking could have only gotten you Prize A or Prize D.

Good job on the first try! This will count for your Understanding Bonus.

Proceed

### D.3.3.2 Menu SP Property: Training Round 2

## The Key Principle of Your Ranking: Training Round 2/3

[Click for a general reminder on this study](#)

[Click for a reminder on the Key Principle of your ranking](#)

*This is a training round.*

*Everything is **the same** as in the real rounds you will play later on, except that you will **not** earn the money worth of the prize you will get. Instead, we will ask you questions which can count for your **Understanding Bonus** at the end of the study.*

*Remember: each question increases your Understanding Bonus only if you answer it correctly on your first attempt. Think about your answers carefully!*

### Step 1: Round Information

In this round, the **prizes** are:

| Prize       | A                                           | B | C | D |
|-------------|---------------------------------------------|---|---|---|
| Money worth | - Training round. No earnings from prizes - |   |   |   |

[Click for a reminder on what the prizes mean](#)

The **prize priorities** for you and for the other participants are:

| Prize                  | A       | B       | C       | D       |
|------------------------|---------|---------|---------|---------|
| 1st priority (highest) | Shirley | You     | Shirley | Ruth    |
| 2nd priority           | Ruth    | Shirley | Theresa | You     |
| 3rd priority           | You     | Ruth    | Ruth    | Theresa |
| 4th priority (lowest)  | Theresa | Theresa | You     | Shirley |

Click for a reminder on what the priorities mean

## Step 2: Submit Your Ranking

Click for a reminder on what this ranking means

Please rank the four prizes **in the fixed, specific order A–B–D–C**.

**A–B–D–C**

## Step 3: Allocation Process

**You get Prize B.**

*In this training round, you will answer a few questions about the Key Principle of your ranking and about this round's outcome. Remember: each question will count for your Understanding Bonus only if you answer it correctly on your first attempt. Think about your answers carefully!*

**Remember: You submitted the ranking A–B–D–C, and ended up getting Prize B.**

Imagine you had instead submitted a different ranking, while all prize priorities and other participants' rankings remained the same.

Given the **Key Principle** of your ranking, which of the following might be true?

If I had instead submitted A–D–B–C, then it is possible (or certain) that I would have gotten Prize A.

(Get it right on first try to increase your bonus)

- True
- False

Correct! Given that you originally ranked Prize A above Prize B but got Prize B, Prize A is not an Obtainable Prize. Hence, **no ranking** could possibly get you Prize A. Good job on the first try! This will count for your Understanding Bonus.

If I had instead submitted A–D–B–C, then it is possible (or certain) that I would have gotten Prize D.  
(Get it right on first try to increase your bonus)

- True  
 False

Correct! Given that you originally ranked Prize B above Prize D but got Prize B, Prize D **could** be an Obtainable Prize. Hence, an alternative ranking could possibly get you Prize D.  
Good job on the first try! This will count for your Understanding Bonus.

If I had instead submitted A–D–B–C, then it is possible (or certain) that I would have gotten Prize C.  
(Get it right on first try to increase your bonus)

- True  
 False

Correct! Given that you originally got Prize B, Prize B is an Obtainable Prize. Since you still rank Prize B above Prize C, you **cannot** possibly get Prize C.  
Good job on the first try! This will count for your Understanding Bonus.

If I had instead submitted C–A–B–D, then it is possible (or certain) that I would have gotten Prize A.  
(Get it right on first try to increase your bonus)

- True  
 False

Correct! Given that you originally ranked Prize A above Prize B but got Prize B, Prize A is not an Obtainable Prize. Hence, **no ranking** could possibly get you Prize A.  
Good job on the first try! This will count for your Understanding Bonus.

If I had instead submitted C–A–B–D, then it is possible (or certain) that I would have gotten Prize C.  
(Get it right on first try to increase your bonus)

- True  
 False

Correct! Given that you originally ranked Prize B above Prize C but got Prize B, Prize C **could** be an Obtainable Prize. Hence, an alternative ranking could possibly get you Prize C.  
Good job on the first try! This will count for your Understanding Bonus.

Imagine you are able to try submitting many different possible rankings, while the prize priorities and other participants' rankings remain the same.

Imagine that you try out and submit **every** possible ranking.

After each such submission, you write down the prize that this submission gets you.

You end up with a log of some, but possibly not all, of the prizes.

Think about each of the prizes: is that prize **definitely** included in the log, **possibly** included in the log, or **definitely not** included in the log?

**(Remember: You submitted the ranking A–B–D–C, and ended up getting Prize B.)**

Choose the correct answer below:

Prize A (Get it right on first try to increase your bonus)

- Definitely included
- Possibly included
- Definitely not included

Correct! Given that you originally ranked Prize A above Prize B but got Prize B, Prize A is not an Obtainable Prize. Hence, **no ranking** could possibly get you Prize A.  
Good job on the first try! This will count for your Understanding Bonus.

Prize B (Get it right on first try to increase your bonus)

- Definitely included
- Possibly included
- Definitely not included

Correct! The ranking that you originally submitted gets you Prize B.  
Good job on the first try! This will count for your Understanding Bonus.

Prize C (Get it right on first try to increase your bonus)

- Definitely included
- Possibly included
- Definitely not included

Correct! Given that you originally ranked Prize B above Prize C but got Prize B, Prize C **could** be an Obtainable Prize. Hence, an alternative ranking could possibly get you Prize C.  
Good job on the first try! This will count for your Understanding Bonus.

Prize D (Get it right on first try to increase your bonus)

- Definitely included
- Possibly included
- Definitely not included

Correct! Given that you originally ranked Prize B above Prize D but got Prize B, Prize D **could** be an Obtainable Prize. Hence, an alternative ranking could possibly get you Prize D.  
Good job on the first try! This will count for your Understanding Bonus.

Proceed

### D.3.3.3 Menu SP Property: Training Round 3

## The Key Principle of Your Ranking: Training Round 3/3

[Click for a general reminder on this study](#)

[Click for a reminder on the Key Principle of your ranking](#)

*This is a training round.*

*Everything is **the same** as in the real rounds you will play later on, except that you will **not** earn the money worth of the prize you will get. Instead, we will ask you questions which can count for your **Understanding Bonus** at the end of the study.*

*Remember: each question increases your Understanding Bonus only if you answer it correctly on your first attempt. Think about your answers carefully!*

### Step 1: Round Information

In this round, the **prizes** are:

| Prize       | A                                           | B | C | D |
|-------------|---------------------------------------------|---|---|---|
| Money worth | - Training round. No earnings from prizes - |   |   |   |

[Click for a reminder on what the prizes mean](#)

The **prize priorities** for you and for the other participants are:

| Prize                  | A       | B       | C       | D       |
|------------------------|---------|---------|---------|---------|
| 1st priority (highest) | Shirley | Shirley | Shirley | Ruth    |
| 2nd priority           | Ruth    | You     | Theresa | Theresa |
| 3rd priority           | You     | Ruth    | Ruth    | You     |
| 4th priority (lowest)  | Theresa | Theresa | You     | Shirley |

Click for a reminder on what the priorities mean

## Step 2: Submit Your Ranking

Click for a reminder on what this ranking means

Please rank the four prizes **in the fixed, specific order D-B-C-A**.

**D-B-C-A**

## Step 3: Allocation Process

**You get Prize A.**

*In this training round, you will answer a few questions about the Key Principle of your ranking and about this round's outcome. Remember: each question will count for your Understanding Bonus only if you answer it correctly on your first attempt. Think about your answers carefully!*

**Remember: You submitted the ranking D-B-C-A, and ended up getting Prize A.**

Imagine you had instead submitted a different ranking, while all prize priorities and other participants' rankings remained the same.

Given the **Key Principle** of your ranking, which of the following might be true?

If I had instead submitted A-D-B-C, then it is possible (or certain) that I would have gotten Prize A. (Get it right on first try to increase your bonus)

- True  
 False

**Correct!** Given that you originally ranked Prize A last and got it, it is the only Obtainable Prize. Hence every possible alternative ranking would only get you Prize A.  
**Good job on the first try! This will count for your Understanding Bonus.**

If I had instead submitted A–D–B–C, then it is possible (or certain) that I would have gotten Prize D.  
(Get it right on first try to increase your bonus)

- True  
 False

Correct! Given that you originally ranked Prize A last and got it, it is the only Obtainable Prize. Hence every possible alternative ranking would only get you Prize A.  
Good job on the first try! This will count for your Understanding Bonus.

If I had instead submitted A–D–B–C, then it is possible (or certain) that I would have gotten Prize C.  
(Get it right on first try to increase your bonus)

- True  
 False

Correct! Given that you originally ranked Prize A last and got it, it is the only Obtainable Prize. Hence every possible alternative ranking would only get you Prize A.  
Good job on the first try! This will count for your Understanding Bonus.

If I had instead submitted C–A–B–D, then it is possible (or certain) that I would have gotten Prize A.  
(Get it right on first try to increase your bonus)

- True  
 False

Correct! Given that you originally ranked Prize A last and got it, it is the only Obtainable Prize. Hence every possible alternative ranking would only get you Prize A.  
Good job on the first try! This will count for your Understanding Bonus.

If I had instead submitted C–A–B–D, then it is possible (or certain) that I would have gotten Prize C.  
(Get it right on first try to increase your bonus)

- True  
 False

Correct! Given that you originally ranked Prize A last and got it, it is the only Obtainable Prize. Hence every possible alternative ranking would only get you Prize A.  
Good job on the first try! This will count for your Understanding Bonus.

Imagine you are able to try submitting many different possible rankings, while the prize priorities and other participants' rankings remain the same.

Imagine that you try out and submit **every** possible ranking.

After each such submission, you write down the prize that this submission gets you.

You end up with a log of some, but possibly not all, of the prizes.

Think about each of the prizes: is that prize **definitely** included in the log, **possibly** included in the log, or **definitely not** included in the log?

**(Remember: You submitted the ranking D–B–C–A, and ended up getting Prize A.)**

Choose the correct answer below:

Prize A (Get it right on first try to increase your bonus)

- Definitely included
- Possibly included
- Definitely not included

Correct! The ranking that you originally submitted gets you Prize A.  
Good job on the first try! This will count for your Understanding Bonus.

Prize B (Get it right on first try to increase your bonus)

- Definitely included
- Possibly included
- Definitely not included

Correct! Given that you originally ranked Prize B above Prize A but got Prize A, Prize B is not an Obtainable Prize. Hence, **no ranking** could possibly get you Prize B.  
Good job on the first try! This will count for your Understanding Bonus.

Prize C (Get it right on first try to increase your bonus)

- Definitely included
- Possibly included
- Definitely not included

Correct! Given that you originally ranked Prize C above Prize A but got Prize A, Prize C is not an Obtainable Prize. Hence, **no ranking** could possibly get you Prize C.  
Good job on the first try! This will count for your Understanding Bonus.

Prize D (Get it right on first try to increase your bonus)

- Definitely included
- Possibly included
- Definitely not included

Correct! Given that you originally ranked Prize D above Prize A but got Prize A, Prize D is not an Obtainable Prize. Hence, **no ranking** could possibly get you Prize D.  
Good job on the first try! This will count for your Understanding Bonus.

Proceed

### D.3.4.0 Textbook SP Property Description

## The Key Principle of Your Ranking

*We will now tell you a general important principle of how your own ranking affects the allocation process.*

***This principle is important to learn:*** *You may be able to apply your knowledge of it to choose your rankings in the upcoming real rounds of this study.*

*The prize you get is determined using an allocation process that uses your own ranking, the rankings of the other participants, and the prize priorities.*

*The following image illustrates this:*

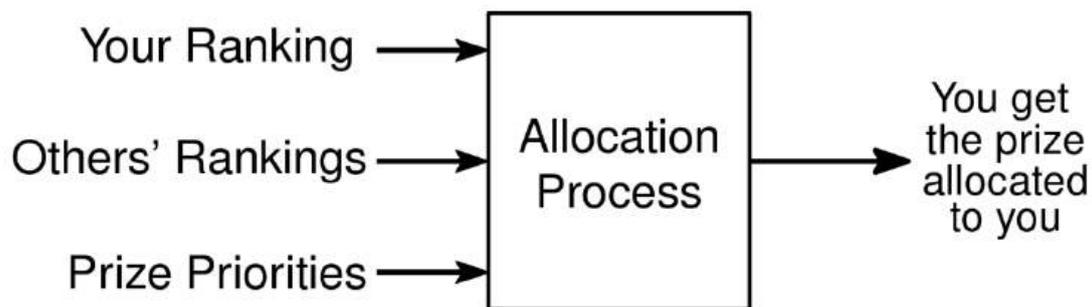

*Now, imagine that the computer already determined some prize priorities and rankings of the other, computerized participants. The only component left undecided is your own ranking. As you decide which ranking to submit, imagine there is some specific ranking that you are considering submitting. Let's call it "the considered ranking."*

***The important principle:*** *The prize you get if you submit the considered ranking is the **highest** that submitting any ranking could get you, **according to the considered ranking.***

*In other words, if you submit any alternative ranking, different from the considered ranking, you will either get **the same** prize you get when submitting the considered ranking, or some prize **lower on the considered ranking**.*

*No alternative ranking can get you a prize which you rank higher on the considered ranking, compared to the prize you get when you submit the considered ranking.*

*For example, imagine that you submitted the ranking A–B–C–D and ended up getting Prize C. This means that Prize C is the highest possible that you could get on the considered ranking A–B–C–D. Submitting any other, alternative ranking different from A–B–C–D could have only gotten you the same prize, Prize C, or possibly a lower-ranked prize on the considered ranking, Prize D. No other alternative ranking could have gotten you Prize A or Prize B.*

*On the next screens you will play training rounds of the game to master your understanding of the allocation process. Click the button below to proceed to these rounds.*

Proceed to training rounds

### D.3.4.1 Textbook SP Property: Training Round 1

## The Key Principle of Your Ranking: Training Round 1/3

[Click for a general reminder on this study](#)

[Click for a reminder on the Key Principle of your ranking](#)

*This is a training round.*

*Everything is **the same** as in the real rounds you will play later on, except that you will **not** earn the money worth of the prize you will get. Instead, we will ask you questions which can count for your **Understanding Bonus** at the end of the study.*

*Remember: each question increases your Understanding Bonus only if you answer it correctly on your first attempt. Think about your answers carefully!*

### Step 1: Round Information

In this round, the **prizes** are:

| Prize       | A                                           | B | C | D |
|-------------|---------------------------------------------|---|---|---|
| Money worth | - Training round. No earnings from prizes - |   |   |   |

[Click for a reminder on what the prizes mean](#)

The **prize priorities** for you and for the other participants are:

| Prize                  | A       | B       | C       | D       |
|------------------------|---------|---------|---------|---------|
| 1st priority (highest) | Shirley | Shirley | Theresa | You     |
| 2nd priority           | Theresa | You     | Shirley | Theresa |
| 3rd priority           | You     | Theresa | You     | Ruth    |
| 4th priority (lowest)  | Ruth    | Ruth    | Ruth    | Shirley |

Click for a reminder on what the priorities mean

## Step 2: Submit Your Ranking

Click for a reminder on what this ranking means

Please rank the four prizes **in the fixed, specific order C-B-A-D**.

**C-B-A-D**

## Step 3: Allocation Process

**You get Prize A.**

*In this training round, you will answer a few questions about the Key Principle of your ranking and about this round's outcome. Remember: each question will count for your Understanding Bonus only if you answer it correctly on your first attempt. Think about your answers carefully!*

In all the following questions, imagine the computer has already determined some prize priorities and rankings of the other, computerized participants, so that the only component left undecided is your own ranking.

Please determine whether the following statements are true or false:

Submitting any ranking of prizes that I consider always gets me a prize **at least as high according to that ranking** compared to the prize I would have gotten if I had submitted any different, alternative ranking.

(Get it right on first try to increase your bonus)

- True  
 False

Correct! The prize you get if you submit any different, alternative ranking can only be **the same** as the prize you get when submitting a ranking that follows that order, or some prize that is ranked **lower according to that order**.

Good job on the first try! This will count for your Understanding Bonus.

Submitting some ranking **cannot** ensure that I will get the **highest-rank** prize in that ranking, but it **does** ensure that I will **not** get the **lowest-rank** prize in that ranking.

(Get it right on first try to increase your bonus)

- True  
 False

Correct! The allocation process only ensures you a prize **at least as highly ranked in your submitted ranking** compared to the prize you would get if you submitted some different, alternative ranking. On some occasions, **the prize you get may be the one you ranked lowest.**

Good job on the first try! This will count for your Understanding Bonus.

Imagine I have a low priority for getting Prize A, which is the prize I want the most, but I have a high priority for getting Prize B, which I want the second most. Then, submitting a ranking that places Prize A first and Prize B second may lead to missing out on both prizes A and B, while submitting a different ranking could have gotten me Prize B.

(Get it right on first try to increase your bonus)

- True  
 False

Correct! Imagine submitting a ranking that places Prize A first and Prize B second, but getting some prize other than Prize A or Prize B. Remember that submitting different, alternative rankings can only get you that **same prize**, or some other **lower prize** according to your original ranking. Hence, no alternative ranking can get you Prize A or Prize B. This is true **regardless of your specific priorities for getting these prizes.**

Good job on the first try! This will count for your Understanding Bonus.

Please answer the following question:

**Remember: You submitted the ranking C–B–A–D, and ended up getting Prize A.** Imagine you had instead submitted a different ranking (while all prize priorities and other participants' rankings remained the same). Which of the following is true? (select one answer)

(Hint: think about a considered ranking and alternative rankings.)

(Get it right on first try to increase your bonus)

- It is certain that every possible ranking I could have submitted would have gotten me Prize A.  
 There might be some alternative ranking I could have submitted that would have gotten me Prize B.  
 There might be some alternative ranking I could have submitted that would have gotten me Prize C.  
 There might be some alternative ranking I could have submitted that would have gotten me Prize D.

Correct! Submitting a ranking different from C–B–A–D could have only gotten you the **same prize** as when submitting the ranking C–B–A–D, that is, Prize A, or some prize **lower** on the original ranking —Prize D. In other words, no alternative, different ranking could have gotten you Prize C or Prize B.

Good job on the first try! This will count for your Understanding Bonus.

Proceed

### D.3.4.2 Textbook SP Property: Training Round 2

## The Key Principle of Your Ranking: Training Round 2/3

[Click for a general reminder on this study](#)

[Click for a reminder on the Key Principle of your ranking](#)

*This is a training round.*

*Everything is **the same** as in the real rounds you will play later on, except that you will **not** earn the money worth of the prize you will get. Instead, we will ask you questions which can count for your **Understanding Bonus** at the end of the study.*

*Remember: each question increases your Understanding Bonus only if you answer it correctly on your first attempt. Think about your answers carefully!*

### Step 1: Round Information

In this round, the **prizes** are:

| Prize       | A                                           | B | C | D |
|-------------|---------------------------------------------|---|---|---|
| Money worth | - Training round. No earnings from prizes - |   |   |   |

[Click for a reminder on what the prizes mean](#)

The **prize priorities** for you and for the other participants are:

| Prize                  | A       | B       | C       | D       |
|------------------------|---------|---------|---------|---------|
| 1st priority (highest) | Shirley | You     | Shirley | Ruth    |
| 2nd priority           | Ruth    | Shirley | Theresa | You     |
| 3rd priority           | You     | Ruth    | Ruth    | Theresa |
| 4th priority (lowest)  | Theresa | Theresa | You     | Shirley |

Click for a reminder on what the priorities mean

## Step 2: Submit Your Ranking

Click for a reminder on what this ranking means

Please rank the four prizes **in the fixed, specific order A-B-D-C**.

**A-B-D-C**

## Step 3: Allocation Process

**You get Prize B.**

*In this training round, you will answer a few questions about the Key Principle of your ranking and about this round's outcome. Remember: each question will count for your Understanding Bonus only if you answer it correctly on your first attempt. Think about your answers carefully!*

**Remember: You submitted the ranking A-B-D-C, and ended up getting Prize B.**

Imagine you had instead submitted a different ranking, while all prize priorities and other participants' rankings remained the same.

Given the **Key Principle** of your ranking, which of the following might be true?

If I had instead submitted A-D-B-C, then it is possible (or certain) that I would have gotten Prize A.  
(Get it right on first try to increase your bonus)

- True  
 False

**Correct!** Given that you originally ranked Prize A above Prize B but got Prize B, **no ranking** could possibly get you Prize A.

**Good job on the first try! This will count for your Understanding Bonus.**

If I had instead submitted A–D–B–C, then it is possible (or certain) that I would have gotten Prize D.  
(Get it right on first try to increase your bonus)

- True  
 False

Correct! Given that you originally ranked Prize B above Prize D and got Prize B, an alternative ranking **could** possibly get you Prize D.

Good job on the first try! This will count for your Understanding Bonus.

If I had instead submitted A–D–B–C, then it is possible (or certain) that I would have gotten Prize C.  
(Get it right on first try to increase your bonus)

- True  
 False

Correct! If you would have gotten Prize C when submitting this new ranking, then getting Prize B by submitting your original ranking would have been **impossible**, since Prize B is ranked higher in this new ranking than Prize C.

Good job on the first try! This will count for your Understanding Bonus.

If I had instead submitted C–A–B–D, then it is possible (or certain) that I would have gotten Prize A.  
(Get it right on first try to increase your bonus)

- True  
 False

Correct! Given that you originally ranked Prize A above Prize B but got Prize B, **no ranking** could possibly get you Prize A.

Good job on the first try! This will count for your Understanding Bonus.

If I had instead submitted C–A–B–D, then it is possible (or certain) that I would have gotten Prize C.  
(Get it right on first try to increase your bonus)

- True  
 False

Correct! Given that you originally ranked Prize B above Prize C and got Prize B, an alternative ranking **could** possibly get you Prize C.

Good job on the first try! This will count for your Understanding Bonus.

Imagine you are able to try submitting many different possible rankings, while the prize priorities and other participants' rankings remain the same.

Imagine that you try out and submit **every** possible ranking.

After each such submission, you write down the prize that this submission gets you.

You end up with a log of some, but possibly not all, of the prizes.

Think about each of the prizes: is that prize **definitely** included in the log, **possibly** included in the log, or **definitely not** included in the log?

**(Remember: You submitted the ranking A–B–D–C, and ended up getting Prize B.)**

Choose the correct answer below:

Prize A (Get it right on first try to increase your bonus)

- Definitely included
- Possibly included
- Definitely not included

Correct! Given that you originally ranked Prize A above Prize B but got Prize B, **no ranking** could possibly get you Prize A.

Good job on the first try! This will count for your Understanding Bonus.

Prize B (Get it right on first try to increase your bonus)

- Definitely included
- Possibly included
- Definitely not included

Correct! The ranking that you originally submitted gets you Prize B.  
Good job on the first try! This will count for your Understanding Bonus.

Prize C (Get it right on first try to increase your bonus)

- Definitely included
- Possibly included
- Definitely not included

Correct! Given that you originally ranked Prize B above Prize C and got Prize B, an alternative ranking **could** possibly get you Prize C.

Good job on the first try! This will count for your Understanding Bonus.

Prize D (Get it right on first try to increase your bonus)

- Definitely included
- Possibly included
- Definitely not included

Correct! Given that you originally ranked Prize B above Prize D and got Prize B, an alternative ranking **could** possibly get you Prize D.

Good job on the first try! This will count for your Understanding Bonus.

Proceed

---

### D.3.4.3 Textbook SP Property: Training Round 3

## The Key Principle of Your Ranking: Training Round 3/3

[Click for a general reminder on this study](#)

[Click for a reminder on the Key Principle of your ranking](#)

*This is a training round.*

*Everything is **the same** as in the real rounds you will play later on, except that you will **not** earn the money worth of the prize you will get. Instead, we will ask you questions which can count for your **Understanding Bonus** at the end of the study.*

*Remember: each question increases your Understanding Bonus only if you answer it correctly on your first attempt. Think about your answers carefully!*

### Step 1: Round Information

In this round, the **prizes** are:

| Prize       | A                                           | B | C | D |
|-------------|---------------------------------------------|---|---|---|
| Money worth | - Training round. No earnings from prizes - |   |   |   |

[Click for a reminder on what the prizes mean](#)

The **prize priorities** for you and for the other participants are:

| Prize                  | A       | B       | C       | D       |
|------------------------|---------|---------|---------|---------|
| 1st priority (highest) | Shirley | Shirley | Shirley | Ruth    |
| 2nd priority           | Ruth    | You     | Theresa | Theresa |
| 3rd priority           | You     | Ruth    | Ruth    | You     |
| 4th priority (lowest)  | Theresa | Theresa | You     | Shirley |

Click for a reminder on what the priorities mean

## Step 2: Submit Your Ranking

Click for a reminder on what this ranking means

Please rank the four prizes **in the fixed, specific order D-B-C-A**.

**D-B-C-A**

## Step 3: Allocation Process

**You get Prize A.**

*In this training round, you will answer a few questions about the Key Principle of your ranking and about this round's outcome. Remember: each question will count for your Understanding Bonus only if you answer it correctly on your first attempt. Think about your answers carefully!*

**Remember: You submitted the ranking D-B-C-A, and ended up getting Prize A.**

Imagine you had instead submitted a different ranking, while all prize priorities and other participants' rankings remained the same.

Given the **Key Principle** of your ranking, which of the following might be true?

If I had instead submitted A-D-B-C, then it is possible (or certain) that I would have gotten Prize A. (Get it right on first try to increase your bonus)

- True  
 False

**Correct!** Given that you originally ranked Prize A last and got it, every possible alternative ranking would only get you Prize A.

**Good job on the first try! This will count for your Understanding Bonus.**

If I had instead submitted A–D–B–C, then it is possible (or certain) that I would have gotten Prize D.  
(Get it right on first try to increase your bonus)

- True  
 False

Correct! Given that you originally ranked Prize A last and got it, every possible alternative ranking would only get you Prize A.

Good job on the first try! This will count for your Understanding Bonus.

If I had instead submitted A–D–B–C, then it is possible (or certain) that I would have gotten Prize C.  
(Get it right on first try to increase your bonus)

- True  
 False

Correct! Given that you originally ranked Prize A last and got it, every possible alternative ranking would only get you Prize A.

Good job on the first try! This will count for your Understanding Bonus.

If I had instead submitted C–A–B–D, then it is possible (or certain) that I would have gotten Prize A.  
(Get it right on first try to increase your bonus)

- True  
 False

Correct! Given that you originally ranked Prize A last and got it, every possible alternative ranking would only get you Prize A.

Good job on the first try! This will count for your Understanding Bonus.

If I had instead submitted C–A–B–D, then it is possible (or certain) that I would have gotten Prize C.  
(Get it right on first try to increase your bonus)

- True  
 False

Correct! Given that you originally ranked Prize A last and got it, every possible alternative ranking would only get you Prize A.

Good job on the first try! This will count for your Understanding Bonus.

Imagine you are able to try submitting many different possible rankings, while the prize priorities and other participants' rankings remain the same.

Imagine that you try out and submit **every** possible ranking.

After each such submission, you write down the prize that this submission gets you.

You end up with a log of some, but possibly not all, of the prizes.

Think about each of the prizes: is that prize **definitely** included in the log, **possibly** included in the log, or **definitely not** included in the log?

**(Remember: You submitted the ranking D–B–C–A, and ended up getting Prize A.)**

Choose the correct answer below:

Prize A (Get it right on first try to increase your bonus)

- Definitely included
- Possibly included
- Definitely not included

Correct! The ranking that you originally submitted gets you Prize A.  
Good job on the first try! This will count for your Understanding Bonus.

Prize B (Get it right on first try to increase your bonus)

- Definitely included
- Possibly included
- Definitely not included

Correct! Given that you originally ranked Prize B above Prize A but got Prize A, **no ranking** could possibly get you Prize B.

Good job on the first try! This will count for your Understanding Bonus.

Prize C (Get it right on first try to increase your bonus)

- Definitely included
- Possibly included
- Definitely not included

Correct! Given that you originally ranked Prize C above Prize A but got Prize A, **no ranking** could possibly get you Prize C.

Good job on the first try! This will count for your Understanding Bonus.

Prize D (Get it right on first try to increase your bonus)

- Definitely included
- Possibly included
- Definitely not included

Correct! Given that you originally ranked Prize D above Prize A but got Prize A, **no ranking** could possibly get you Prize D.

Good job on the first try! This will count for your Understanding Bonus.

Proceed

---

### D.3.5.0 Null Description (Repeated)

## The Basics

*We will now remind you of the general details of the game and allocation process. This page includes the **exact same text** you read at the beginning of the study. Please read it again to make sure you understand.*

*In this study, you and three computerized participants, Ruth, Shirley, and Theresa, are going to play a game for four prizes. Each prize is worth money, but might be worth a different amount of money for each participant.*

*You and the computerized participants will each rank the four prizes in any order you wish. Then, an **allocation process** will use these rankings to allocate the prizes—one prize for each participant.*

*The allocation process attempts to give each participant a prize that they ranked higher rather than a prize that they ranked lower. However, this is not always possible, since the allocation process must take into account the rankings of all participants.*

*You will now learn about the game and allocation process. The text in blue bubbles, such as this text, provides explanations about the game and allocation process. **Make sure you read it carefully.***

*A round of the game has three steps.*

## Step 1: Round Information

*In Step 1, you first see the **prizes** you can get in this round and how much money they are worth to **you**.*

In this round, the **prizes** are:

| <b>Prize</b> | <b>A</b> | <b>B</b> | <b>C</b> | <b>D</b> |
|--------------|----------|----------|----------|----------|
| Money worth  | 67¢      | 7¢       | 95¢      | 45¢      |

*In the table above, under each prize A, B, C or D, you can see how much money it would add to **your** earnings.*

*Each prize might be worth a **different** amount of money for each participant, and each participant can only see the money amounts relevant to **themselves**. However, the prizes that earn **you** a large amount of money are also likely to earn the **other participants** a large amount of money. There is more likely to be **competition** for the high-earning prizes.*

*The money worth of prizes for you and for the other participants can be different in different rounds of the game, and they were **determined beforehand**. You and the other participants **cannot affect the money worth of prizes**.*

*Still in Step 1, you see next what we call the **prize priorities**.*

*All four participants have some **priority** for getting each of the four prizes.*

*These priorities can affect the allocation of prizes.*

*The higher your priority is for getting some prize, the more likely you generally are to get that prize at the end of the process.*

In this round, the **prize priorities** for you and for the other participants are:

| <b>Prize</b>           | <b>A</b> | <b>B</b> | <b>C</b> | <b>D</b> |
|------------------------|----------|----------|----------|----------|
| 1st priority (highest) | Ruth     | Shirley  | Theresa  | You      |
| 2nd priority           | Shirley  | You      | Shirley  | Theresa  |
| 3rd priority           | You      | Theresa  | You      | Ruth     |
| 4th priority (lowest)  | Theresa  | Ruth     | Ruth     | Shirley  |

Each column shows the priorities of all participants for getting some prize, written from highest to lowest

The prize priorities can be different in different rounds of the game, and they were **determined beforehand**.

You and the other participants **cannot affect the prize priorities**.

## Step 2: Submit Your Ranking

In Step 2, you are asked to **rank the four prizes**.

Please type your ranking of the four prizes in an order of your choice in the box below. For example, if you want to rank Prize A first, Prize B second, Prize C third and Prize D fourth, type "A" followed by "B" followed by "C" followed by "D," and then click "Submit Ranking."

**D-A-C-B**

The computerized participants simultaneously submit their own rankings. They **do not know your own ranking**.

Their rankings are aimed at getting them their high-earning prizes. Your own ranking **cannot affect the computerized participants' rankings**.

### Step 3: Allocation Process

*In Step 3, the allocation process allocates the prizes to participants. Then, you get the prize that was allocated to you.*

*Remember:*

*The allocation process attempts to give each participant a prize that they ranked higher rather than a prize that they ranked lower. However, this is not always possible, since the allocation process must take into account the rankings of all participants.*

*Additionally, the prize priorities can affect the allocation of prizes.*

*The higher your priority is for getting some prize, the more likely you generally are to get that prize at the end of the process.*

#### **You get Prize D.**

If this were a real round, your total earning would increase by 45¢.

*That's it!*

*Click on the button below to proceed to training rounds.*

Proceed to training rounds

### D.3.5.1 Null Description (Repeated): Training Round 1

## Additional Training Round 1/3

Click for a general reminder on this study

*Note: This training round includes the exact questions that you already answered before. Nevertheless, please read them and answer again to make sure you understand.*

*This is a training round.*

*Everything is **the same** as in the real rounds you will play later on, except that you will **not** earn the money worth of the prize you will get. Instead, we will ask you questions which can count for your **Understanding Bonus** at the end of the study.*

*Remember: each question increases your Understanding Bonus only if you answer it correctly on your first attempt. Think about your answers carefully!*

### Step 1: Round Information

In this round, your **prizes** are:

| Prize       | A   | B  | C   | D   |
|-------------|-----|----|-----|-----|
| Money worth | 79¢ | 9¢ | 45¢ | 94¢ |

Click for a reminder on what the prizes mean

Please determine whether the following statement is true or false:

If I rank some prize very **low** and get it, I may earn **less** than its money worth, shown in the table above. If I rank some prize very **high** and get it, I may earn **more** than its money worth.

(Get it right on first try to increase your bonus)

- True  
 False

**Correct!** Your own ranking cannot affect the money worth of prizes shown in your table, which are determined beforehand.

**Good job on the first try!** This will count for your Understanding Bonus.

Please determine whether the following statement is true or false:

Every participant, including me and the computerized participants, has the same earnings table.  
(Get it right on first try to increase your bonus)

- True  
 False

Correct! Each prize might be worth a different amount for each participant.  
Good job on the first try! This will count for your Understanding Bonus.

The **prize priorities** for you and for the other participants are:

| Prize                  | A       | B       | C       | D       |
|------------------------|---------|---------|---------|---------|
| 1st priority (highest) | You     | Theresa | Shirley | Ruth    |
| 2nd priority           | Shirley | You     | Ruth    | You     |
| 3rd priority           | Theresa | Shirley | Theresa | Theresa |
| 4th priority (lowest)  | Ruth    | Ruth    | You     | Shirley |

[Click here for a reminder on what the priorities mean](#)

Please determine whether the following statement is true or false:

If I place a prize very **low** in my ranking, then my priority for getting that prize (in the table above) might **decrease**. If I place a prize very **high** in my ranking, then my priority for getting that prize (in the table above) might **increase**.

(Get it right on first try to increase your bonus)

- True  
 False

Correct! Your own ranking cannot affect the prize priorities. Instead, they are determined beforehand.  
Good job on the first try! This will count for your Understanding Bonus.

## Step 2: Submit Your Ranking

Click for a reminder on what this ranking means

Please rank the four prizes in an order of your choice.

**D-A-C-B**

## Step 3: Allocation Process

*Remember:*

*The allocation process attempts to give each participant a prize that they ranked higher rather than a prize that they ranked lower. However, this is not always possible, since the allocation process must take into account the rankings of all participants.*

*The prize priorities can affect the allocation of prizes.*

*The higher your priority is at some prize, the more likely you generally are to get that prize at the end of the process.*

### **You get Prize A.**

If this were a real round, your total earning would increase by 79¢.

Since this is a training round, the questions you answer correctly on the first attempt count for your Understanding Bonus.

Please answer the following question:

How many prizes can you get at most at the end of the allocation process? The correct answer is that you **always** get one prize, no more and no less, so you should select the number one.

(Get it right on first try to increase your bonus)

Answer:

**Correct! You always get one prize at the end of the allocation process.  
Good job on the first try! This will count for your Understanding Bonus.**

Please determine whether the following statement is true or false:

I just submitted some ranking and got some prize. It is possible that if I had submitted a different ranking, my ranking would have **affected the other participants' rankings** such that I would have gotten a different prize.

(Get it right on first try to increase your bonus)

- True  
 False

**Correct! Your own ranking cannot affect the other participants' rankings.  
Good job on the first try! This will count for your Understanding Bonus.**

Proceed

## Step 2: Submit Your Ranking

Click for a reminder on what this ranking means

Please rank the four prizes in an order of your choice.

**D-A-C-B**

## Step 3: Allocation Process

*Remember:*

*The allocation process attempts to give each participant a prize that they ranked higher rather than a prize that they ranked lower. However, this is not always possible, since the allocation process must take into account the rankings of all participants.*

*The prize priorities can affect the allocation of prizes.*

*The higher your priority is at some prize, the more likely you generally are to get that prize at the end of the process.*

### **You get Prize A.**

If this were a real round, your total earning would increase by 79¢.

Since this is a training round, the questions you answer correctly on the first attempt count for your Understanding Bonus.

Please answer the following question:

How many prizes can you get at most at the end of the allocation process? The correct answer is that you **always** get one prize, no more and no less, so you should select the number one.

(Get it right on first try to increase your bonus)

Answer:

**Correct! You always get one prize at the end of the allocation process.  
Good job on the first try! This will count for your Understanding Bonus.**

Please determine whether the following statement is true or false:

I just submitted some ranking and got some prize. It is possible that if I had submitted a different ranking, my ranking would have **affected the other participants' rankings** such that I would have gotten a different prize.

(Get it right on first try to increase your bonus)

- True  
 False

**Correct! Your own ranking cannot affect the other participants' rankings.  
Good job on the first try! This will count for your Understanding Bonus.**

Proceed

### D.3.5.2 Null Description (Repeated): Training Round 2

## Additional Training Round 2/3

[Click for a general reminder on this study](#)

*This is a training round.*

*Everything is **the same** as in the real rounds you will play later on, except that you will **not** earn the money worth of the prize you will get. Instead, completing this round will count for your **Understanding Bonus** at the end of the study.*

### Step 1: Round Information

In this round, your **prizes** are:

| Prize       | A   | B   | C  | D   |
|-------------|-----|-----|----|-----|
| Money worth | 30¢ | 99¢ | 8¢ | 86¢ |

[Click for a reminder on what the prizes mean](#)

The **prize priorities** for you and for the other participants are:

| Prize                  | A       | B       | C       | D       |
|------------------------|---------|---------|---------|---------|
| 1st priority (highest) | You     | You     | Shirley | Theresa |
| 2nd priority           | Shirley | Theresa | Ruth    | Ruth    |
| 3rd priority           | Theresa | Shirley | Theresa | You     |
| 4th priority (lowest)  | Ruth    | Ruth    | You     | Shirley |

[Click here for a reminder on what the priorities mean](#)

## Step 2: Submit Your Ranking

[Click for a reminder on what this ranking means](#)

Please rank the four prizes in an order of your choice.

**B-D-A-C**

## Step 3: Allocation Process

**You get Prize B.**

If this were a real round, your total earning would increase by 99¢.

Since this is a training round, it will count for your Understanding Bonus like answering one question correctly.

Proceed

---

### D.3.5.3 Null Description (Repeated): Training Round 3

## Additional Training Round 3/3

[Click for a general reminder on this study](#)

*This is a training round.*

*Everything is **the same** as in the real rounds you will play later on, except that you will **not** earn the money worth of the prize you will get. Instead, completing this round will count for your **Understanding Bonus** at the end of the study.*

### Step 1: Round Information

In this round, your **prizes** are:

| Prize       | A   | B  | C   | D   |
|-------------|-----|----|-----|-----|
| Money worth | 45¢ | 0¢ | 78¢ | 96¢ |

[Click for a reminder on what the prizes mean](#)

The **prize priorities** for you and for the other participants are:

| Prize                  | A       | B       | C       | D       |
|------------------------|---------|---------|---------|---------|
| 1st priority (highest) | Shirley | Theresa | Ruth    | Shirley |
| 2nd priority           | Ruth    | You     | Theresa | Ruth    |
| 3rd priority           | You     | Ruth    | Shirley | Theresa |
| 4th priority (lowest)  | Theresa | Shirley | You     | You     |

[Click here for a reminder on what the priorities mean](#)

## Step 2: Submit Your Ranking

Click for a reminder on what this ranking means

Please rank the four prizes in an order of your choice.

**D-C-A-B**

## Step 3: Allocation Process

**You get Prize C.**

If this were a real round, your total earning would increase by 78¢.

Since this is a training round, it will count for your Understanding Bonus like answering one question correctly.

Proceed

## D.4 Real Rounds

You completed the training rounds.

Click the button below to proceed to real rounds of the game.

Next

## Round 1/10

[Click for a general reminder on this study](#)

[Click for a reminder on the technical details of the allocation process](#)

***This is a real round!***

*Your total earnings will increase according to the prize you will get at the end of the round.*

### Step 1: Round Information

In this round, your **prizes** are:

| Prize       | A   | B   | C  | D   |
|-------------|-----|-----|----|-----|
| Money worth | 84¢ | 95¢ | 3¢ | 30¢ |

[Click here for a reminder on what the prizes mean](#)

The **prize priorities** for you and for the other participants are:

| Prize                  | A       | B       | C       | D       |
|------------------------|---------|---------|---------|---------|
| 1st priority (highest) | Ruth    | Ruth    | Shirley | Theresa |
| 2nd priority           | Shirley | Shirley | Theresa | You     |
| 3rd priority           | You     | You     | Ruth    | Shirley |
| 4th priority (lowest)  | Theresa | Theresa | You     | Ruth    |

[Click here for a reminder on what the priorities mean](#)

## Step 2: Submit Your Ranking

Please rank the four prizes in an order of your choice.

[Click here for a reminder on what this ranking means](#)

**B-A-D-C**

**You get Prize C**, and your total earnings increase by **3¢**.

[Next](#)

Your earnings in the real rounds so far are: 3¢

## Round 2/10

[Click for a general reminder on this study](#)

[Click for a reminder on the technical details of the allocation process](#)

### ***This is a real round!***

*Your total earnings will increase according to the prize you will get at the end of the round.*

## Step 1: Round Information

In this round, your **prizes** are:

| <b>Prize</b> | <b>A</b> | <b>B</b> | <b>C</b> | <b>D</b> |
|--------------|----------|----------|----------|----------|
| Money worth  | 53¢      | 1¢       | 34¢      | 95¢      |

[Click here for a reminder on what the prizes mean](#)

The **prize priorities** for you and for the other participants are:

| <b>Prize</b>           | <b>A</b> | <b>B</b> | <b>C</b> | <b>D</b> |
|------------------------|----------|----------|----------|----------|
| 1st priority (highest) | You      | You      | Shirley  | Ruth     |
| 2nd priority           | Theresa  | Ruth     | You      | You      |
| 3rd priority           | Shirley  | Theresa  | Theresa  | Shirley  |
| 4th priority (lowest)  | Ruth     | Shirley  | Ruth     | Theresa  |

[Click here for a reminder on what the priorities mean](#)

## Step 2: Submit Your Ranking

Please rank the four prizes in an order of your choice.

[Click here for a reminder on what this ranking means](#)

**D-A-C-B**

**You get Prize A**, and your total earnings increase by **53¢**.

[Next](#)

## Round 3/10

[Click for a general reminder on this study](#)

[Click for a reminder on the technical details of the allocation process](#)

***This is a real round!***

*Your total earnings will increase according to the prize you will get at the end of the round.*

### Step 1: Round Information

In this round, your **prizes** are:

| Prize       | A  | B   | C   | D   |
|-------------|----|-----|-----|-----|
| Money worth | 3¢ | 90¢ | 39¢ | 58¢ |

[Click here for a reminder on what the prizes mean](#)

The **prize priorities** for you and for the other participants are:

| Prize                  | A       | B       | C       | D       |
|------------------------|---------|---------|---------|---------|
| 1st priority (highest) | Theresa | Ruth    | Ruth    | Shirley |
| 2nd priority           | Ruth    | Shirley | You     | Theresa |
| 3rd priority           | Shirley | Theresa | Shirley | Ruth    |
| 4th priority (lowest)  | You     | You     | Theresa | You     |

[Click here for a reminder on what the priorities mean](#)

## Step 2: Submit Your Ranking

Please rank the four prizes in an order of your choice.

[Click here for a reminder on what this ranking means](#)

**B-D-C-A**

**You get Prize C**, and your total earnings increase by **39¢**.

[Next](#)

## Round 4/10

[Click for a general reminder on this study](#)

[Click for a reminder on the technical details of the allocation process](#)

***This is a real round!***

*Your total earnings will increase according to the prize you will get at the end of the round.*

### Step 1: Round Information

In this round, your **prizes** are:

| Prize       | A   | B   | C   | D  |
|-------------|-----|-----|-----|----|
| Money worth | 34¢ | 91¢ | 88¢ | 2¢ |

[Click here for a reminder on what the prizes mean](#)

The **prize priorities** for you and for the other participants are:

| Prize                  | A       | B       | C       | D       |
|------------------------|---------|---------|---------|---------|
| 1st priority (highest) | You     | Ruth    | Ruth    | Ruth    |
| 2nd priority           | Ruth    | Shirley | Theresa | You     |
| 3rd priority           | Theresa | You     | You     | Shirley |
| 4th priority (lowest)  | Shirley | Theresa | Shirley | Theresa |

[Click here for a reminder on what the priorities mean](#)

## Step 2: Submit Your Ranking

Please rank the four prizes in an order of your choice.

[Click here for a reminder on what this ranking means](#)

**B-C-A-D**

**You get Prize A**, and your total earnings increase by **34¢**.

[Next](#)

Your earnings in the real rounds so far are: \$1.29

## Round 5/10

[Click for a general reminder on this study](#)

[Click for a reminder on the technical details of the allocation process](#)

### ***This is a real round!***

*Your total earnings will increase according to the prize you will get at the end of the round.*

## Step 1: Round Information

In this round, your **prizes** are:

| <b>Prize</b> | <b>A</b> | <b>B</b> | <b>C</b> | <b>D</b> |
|--------------|----------|----------|----------|----------|
| Money worth  | 96¢      | 5¢       | 72¢      | 19¢      |

[Click here for a reminder on what the prizes mean](#)

The **prize priorities** for you and for the other participants are:

| <b>Prize</b>           | <b>A</b> | <b>B</b> | <b>C</b> | <b>D</b> |
|------------------------|----------|----------|----------|----------|
| 1st priority (highest) | Ruth     | Theresa  | You      | Theresa  |
| 2nd priority           | You      | You      | Shirley  | Shirley  |
| 3rd priority           | Theresa  | Ruth     | Theresa  | You      |
| 4th priority (lowest)  | Shirley  | Shirley  | Ruth     | Ruth     |

[Click here for a reminder on what the priorities mean](#)

## Step 2: Submit Your Ranking

Please rank the four prizes in an order of your choice.

[Click here for a reminder on what this ranking means](#)

**A-C-D-B**

**You get Prize C**, and your total earnings increase by **72¢**.

[Next](#)

Your earnings in the real rounds so far are: \$2.01

## Round 6/10

[Click for a general reminder on this study](#)

[Click for a reminder on the technical details of the allocation process](#)

***This is a real round!***

*Your total earnings will increase according to the prize you will get at the end of the round.*

### Step 1: Round Information

In this round, your **prizes** are:

| Prize       | A  | B   | C   | D   |
|-------------|----|-----|-----|-----|
| Money worth | 4¢ | 94¢ | 18¢ | 83¢ |

[Click here for a reminder on what the prizes mean](#)

The **prize priorities** for you and for the other participants are:

| Prize                  | A       | B       | C       | D       |
|------------------------|---------|---------|---------|---------|
| 1st priority (highest) | Ruth    | Shirley | Theresa | You     |
| 2nd priority           | You     | Theresa | Ruth    | Ruth    |
| 3rd priority           | Shirley | Ruth    | Shirley | Shirley |
| 4th priority (lowest)  | Theresa | You     | You     | Theresa |

[Click here for a reminder on what the priorities mean](#)

## Step 2: Submit Your Ranking

Please rank the four prizes in an order of your choice.

[Click here for a reminder on what this ranking means](#)

**B-D-C-A**

**You get Prize D**, and your total earnings increase by **83¢**.

[Next](#)

Your earnings in the real rounds so far are: \$2.84

## Round 7/10

[Click for a general reminder on this study](#)

[Click for a reminder on the technical details of the allocation process](#)

***This is a real round!***

*Your total earnings will increase according to the prize you will get at the end of the round.*

### Step 1: Round Information

In this round, your **prizes** are:

| Prize       | A   | B   | C  | D   |
|-------------|-----|-----|----|-----|
| Money worth | 57¢ | 37¢ | 7¢ | 93¢ |

[Click here for a reminder on what the prizes mean](#)

The **prize priorities** for you and for the other participants are:

| Prize                  | A       | B       | C       | D       |
|------------------------|---------|---------|---------|---------|
| 1st priority (highest) | Shirley | Theresa | Ruth    | Shirley |
| 2nd priority           | Theresa | Shirley | Theresa | Theresa |
| 3rd priority           | Ruth    | You     | Shirley | Ruth    |
| 4th priority (lowest)  | You     | Ruth    | You     | You     |

[Click here for a reminder on what the priorities mean](#)

## Step 2: Submit Your Ranking

Please rank the four prizes in an order of your choice.

[Click here for a reminder on what this ranking means](#)

**D-A-B-C**

**You get Prize B**, and your total earnings increase by **37¢**.

[Next](#)

Your earnings in the real rounds so far are: \$3.21

## Round 8/10

[Click for a general reminder on this study](#)

[Click for a reminder on the technical details of the allocation process](#)

### ***This is a real round!***

*Your total earnings will increase according to the prize you will get at the end of the round.*

## Step 1: Round Information

In this round, your **prizes** are:

| <b>Prize</b> | <b>A</b> | <b>B</b> | <b>C</b> | <b>D</b> |
|--------------|----------|----------|----------|----------|
| Money worth  | 97¢      | 2¢       | 84¢      | 11¢      |

[Click here for a reminder on what the prizes mean](#)

The **prize priorities** for you and for the other participants are:

| <b>Prize</b>           | <b>A</b> | <b>B</b> | <b>C</b> | <b>D</b> |
|------------------------|----------|----------|----------|----------|
| 1st priority (highest) | Theresa  | Theresa  | Ruth     | Ruth     |
| 2nd priority           | Shirley  | Ruth     | You      | Theresa  |
| 3rd priority           | Ruth     | You      | Shirley  | Shirley  |
| 4th priority (lowest)  | You      | Shirley  | Theresa  | You      |

[Click here for a reminder on what the priorities mean](#)

## Step 2: Submit Your Ranking

Please rank the four prizes in an order of your choice.

[Click here for a reminder on what this ranking means](#)

**A-C-D-B**

**You get Prize B**, and your total earnings increase by **2¢**.

[Next](#)

Your earnings in the real rounds so far are: \$3.23

## Round 9/10

[Click for a general reminder on this study](#)

[Click for a reminder on the technical details of the allocation process](#)

### ***This is a real round!***

*Your total earnings will increase according to the prize you will get at the end of the round.*

## Step 1: Round Information

In this round, your **prizes** are:

| <b>Prize</b> | <b>A</b> | <b>B</b> | <b>C</b> | <b>D</b> |
|--------------|----------|----------|----------|----------|
| Money worth  | 96¢      | 57¢      | 3¢       | 13¢      |

[Click here for a reminder on what the prizes mean](#)

The **prize priorities** for you and for the other participants are:

| <b>Prize</b>           | <b>A</b> | <b>B</b> | <b>C</b> | <b>D</b> |
|------------------------|----------|----------|----------|----------|
| 1st priority (highest) | Ruth     | Ruth     | You      | Shirley  |
| 2nd priority           | You      | You      | Ruth     | Theresa  |
| 3rd priority           | Theresa  | Shirley  | Shirley  | You      |
| 4th priority (lowest)  | Shirley  | Theresa  | Theresa  | Ruth     |

[Click here for a reminder on what the priorities mean](#)

## Step 2: Submit Your Ranking

Please rank the four prizes in an order of your choice.

[Click here for a reminder on what this ranking means](#)

**A-B-D-C**

**You get Prize B**, and your total earnings increase by **57¢**.

[Next](#)

Your earnings in the real rounds so far are: \$3.80

## Round 10/10

[Click for a general reminder on this study](#)

[Click for a reminder on the technical details of the allocation process](#)

### ***This is a real round!***

*Your total earnings will increase according to the prize you will get at the end of the round.*

## Step 1: Round Information

In this round, your **prizes** are:

| <b>Prize</b> | <b>A</b> | <b>B</b> | <b>C</b> | <b>D</b> |
|--------------|----------|----------|----------|----------|
| Money worth  | 99¢      | 46¢      | 7¢       | 57¢      |

[Click here for a reminder on what the prizes mean](#)

The **prize priorities** for you and for the other participants are:

| <b>Prize</b>           | <b>A</b> | <b>B</b> | <b>C</b> | <b>D</b> |
|------------------------|----------|----------|----------|----------|
| 1st priority (highest) | Ruth     | You      | You      | You      |
| 2nd priority           | You      | Shirley  | Theresa  | Ruth     |
| 3rd priority           | Theresa  | Theresa  | Ruth     | Theresa  |
| 4th priority (lowest)  | Shirley  | Ruth     | Shirley  | Shirley  |

[Click here for a reminder on what the priorities mean](#)

## Step 2: Submit Your Ranking

Please rank the four prizes in an order of your choice.

[Click here for a reminder on what this ranking means](#)

**A-D-B-C**

**You get Prize D**, and your total earnings increase by **57¢**.

[Next](#)

### D.5.1 Strategyproofness Understanding Test "AbstractHard"

## Final Questions (1/4)

You completed all rounds of the game. We will now ask you some final questions about the game and about yourself and some general questions. This will take about 15 more minutes. Please answer thoughtfully.

First, **imagine** that you have participated in a round with the following scenario.

The prizes in this imaginary round were:

| <b>Prize</b> | <b>A</b> | <b>B</b> | <b>C</b> | <b>D</b> |
|--------------|----------|----------|----------|----------|
| Money worth  | 74¢      | 98¢      | 36¢      | 9¢       |

The prize priorities in this imaginary round were:

| <b>Prize</b>           | <b>A</b> | <b>B</b> | <b>C</b> | <b>D</b> |
|------------------------|----------|----------|----------|----------|
| 1st priority (highest) | Ruth     | Shirley  | You      | Shirley  |
| 2nd priority           | Shirley  | You      | Shirley  | Theresa  |
| 3rd priority           | You      | Theresa  | Theresa  | Ruth     |
| 4th priority (lowest)  | Theresa  | Ruth     | Ruth     | You      |

Finally, imagine that you have submitted the ranking **B-A-C-D**, and got **Prize C**.

Please answer the following questions.

(Each Yes/No you determine correctly will count as **2 questions** for your Understanding Bonus)

If you had instead submitted **A-B-C-D**, and the prize priorities and other participants' rankings did not change, is it possible (or certain) that you would have gotten...?

Prize A

Yes

No

Prize B

Yes

No

Prize C

Yes

No

Prize D

Yes

No

---

If you had instead submitted **D-A-B-C**, and the prize priorities and other participants' rankings did not change, is it possible (or certain) that you would have gotten...?

Prize A

Yes

No

Prize B

Yes

No

Prize C

Yes

No

Prize D

Yes

No

---

If you had instead submitted **D-A-B-C**, this would be unimportant for this question. Instead of answering this question according to the problem, you should choose the next four answers in the order yes, yes, no, yes...

Prize A

- Yes
- No

Prize B

- Yes
- No

Prize C

- Yes
- No

Prize D

- Yes
- No

---

Submit

## D.5.2 Strategyproofness Understanding Test "AbstractMedium"

### Final Questions (1/4)

Now we will ask you several similar questions. In each of these questions, the prize values and prize priorities will be different, but we will now **only** show you **which ranking you submit** and **which prize you get**.

In these next two questions, if you cannot tell for sure what prize you would have gotten in some case, please simply check the box saying "I do not have enough information to know what prize I would have gotten."

(Each answer you determine correctly will count as **2 questions** for your Understanding Bonus.)

Imagine that in some round you submit **D-C-B-A**, and get **Prize C**.

If you had instead submitted **D-B-C-A**, and the prize priorities and other participants' rankings did not change, then which of the following is true?

- I do not have enough information to know what prize I would have gotten.
- I would have gotten prize A.
- I would have gotten prize B.
- I would have gotten prize C.
- I would have gotten prize D.

---

Now, imagine a different round.

Imagine that you submit **C-D-B-A**, and get **Prize B**.

If you had instead submitted **D-C-B-A**, and the prize priorities and other participants' rankings did not change, then which of the following is true?

- I do not have enough information to know what prize I would have gotten.
- I would have gotten prize A.
- I would have gotten prize B.
- I would have gotten prize C.
- I would have gotten prize D.

Submit

### D.5.3 Strategyproofness Understanding Test "AbstractEasy"

## Final Questions (1/4)

Now we will ask you three questions concerning one possible round.

(Each answer you determine correctly will count as 2 questions for your Understanding Bonus.)

Imagine that in some round you submit **B–D–C–A**, and get **Prize C**.

If you had submitted some alternative ranking, and the prize priorities and other participants' rankings did not change, then which of the following is true about **Prize A**?

- There is no alternative ranking such that I would have gotten Prize A.
- There may be (or there definitely is) some alternative ranking such that I would have gotten Prize A.

If you had submitted some alternative ranking, and the prize priorities and other participants' rankings did not change, then which of the following is true about **Prize B**?

- There is no alternative ranking that would have gotten me Prize B.
- There may be (or there definitely is) some alternative ranking that would have gotten me Prize B.

If you had submitted some alternative ranking, and the prize priorities and other participants' rankings did not change, then which of the following is true about **Prize D**?

- There is no alternative ranking that would have gotten me Prize D.
- There may be (or there definitely is) some alternative ranking that would have gotten me Prize D.

Submit

## D.5.4 Strategyproofness Understanding Test "Practical"

### Final Questions (1/4)

Now, please answer these last questions for this part:

(Each True/False you determine correctly will count as **2 questions** for your Understanding Bonus)

If I want to **maximize my earnings** in a given round, then...

Sometimes I might have to rank the prize that earns me the most in second place or lower.

- True
- False

I should consider **only** how much each prize earns me while choosing my own ranking.

- True
- False

I should rank from the highest-earning to lowest-earning prize regardless of anything else.

- True
- False

I should consider the possible rankings of the other participants while choosing my own ranking.

- True
- False

I should consider the prize priorities while choosing my own rankings.

- True
- False

Submit

## D.6 Reflections Questionnaire

### Final Questions (2/4)

From this point on we no longer care about right or wrong answers, we are only interested in your **honest** reflections and opinions.

None of the questions from this point on will count for your Understanding Bonus.

Please answer the following questions about your experience playing the game.

We'll start with a general question: **How did you typically rank the four prizes** in the 10 real rounds? Please share with us your main considerations, even if you are not sure that you always thought about them all.

A

Did you **change** the way you rank throughout the game? If so, in which way and at which point?

B

In your view, did the explanations given during the game **lead you to use a specific method** of ranking the four prizes?

- No  
 Yes

**If you answered "No" above:** Why do you think the explanations did not lead you to use a specific method of ranking the four prizes?

C

**If you answered "Yes" above:** What was that specific ranking method, and why did you use it?

D

How well do you think you now understand how to **best choose** your own ranking?

(Note: you have to drag the sliders below to fill in a response. In case you want to keep a slider in the leftmost position, please drag it and return it to that position.)

I do not understand at all

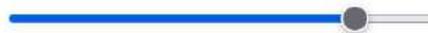

I understand very well

6

How well do you think you now understand the **key principle** of your ranking?

I do not understand at all

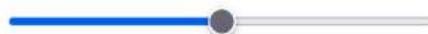

I understand very well

4

How well do you think you now understand how the allocation process **works**?

I do not understand at all

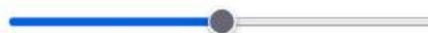

I understand very well

4

Imagine that the allocation process was used to give prizes to real people in a real-world setting. In particular, suppose that each participant is separately awarded prizes in the same way you were awarded prizes.

To what extent do you agree with the following statements?

The allocation process always ends with **each** participant getting a **different** prize, and **each** prize given to **some** participant.

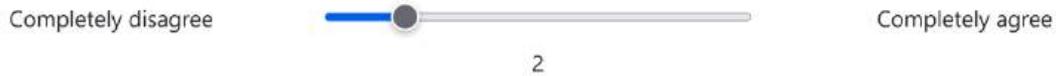

For a process that has to produce an allocation from given prize priorities and participants' rankings, the allocation process is **fair**.

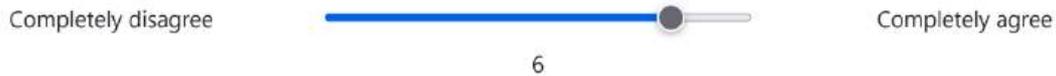

For a process that has to produce an allocation from given prize priorities and participants' rankings, the allocation process is **an overall good way** to allocate the prizes.

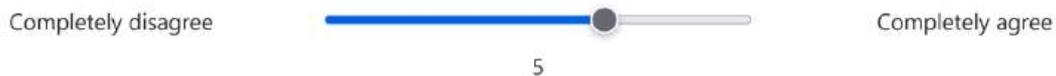

How much would you be willing to **rely on the allocation process** in an important situation in real life (for example, assignment of students to public schools)?

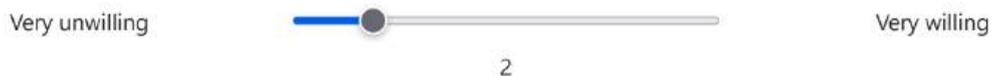

How **transparent is the allocation process**, meaning that you received a full explanation of how the allocation process really works, and no details were kept away from you?

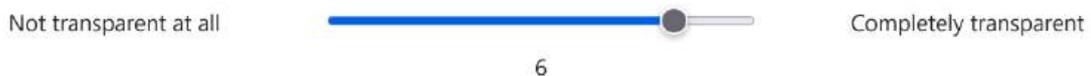

How **predictable** is the final allocation?

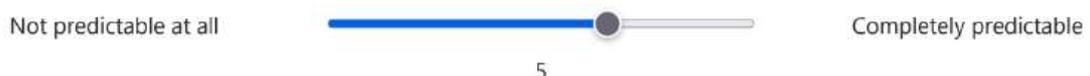

To what extent do you think that **your submitted ranking matters** for the final allocation?

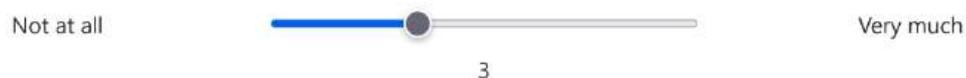

Next

## D.7 Cognitive-Abilities Test

### Final Questions (3/4)

Please answer the following questions:

---

A bat and a ball cost \$1.10 in total. The bat costs \$1.00 more than the ball.  
How much does the ball cost? Please enter an amount in cents:

cents

---

If it takes 5 machines 5 minutes to make 5 widgets, how long would it take 100 machines to make 100 widgets? Please enter a number of minutes:

minutes

---

In a lake, there is a patch of lily pads.  
Every day, the patch doubles in size. If it takes 48 days for the patch to cover the entire lake, how long would it take for the patch to cover half of the lake? Please enter a number of days:

days

---

Out of 1,000 people in a small town 500 are members of a choir. Out of these 500 members in the choir 100 are men.  
Out of the 500 inhabitants that are not in the choir 300 are men. What is the probability that a randomly drawn man is a member of the choir? Please enter a percent chance between 0 and 100:

percent chance

---

Submit

## Final Questions (4/4)

We are almost done. This is the last part of the study. We just have a few more questions to get a little background information for statistical purposes.

What is your state of residence?

 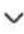

What is your zip code? (5 digits)?

Including you, how many people live in your household?

How many people who live in this household are 18 or older?

What is your year of birth?

 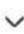

What is your gender?

- Male
- Female
- Non-binary
- Other
- Prefer not to answer

What is your race/ethnicity?

- White and/or European-American
- Black and/or African-American
- Native American and/or First Nations
- Hispanic and/or Latino
- Asian and/or Pacific Islander
- Middle-Eastern and/or North African
- Multiracial and/or Mixed
- Other
- Prefer not to answer

What is the highest level of education you have completed?

- Middle School or less
- Some high school
- High school diploma
- GED (HS Equivalent)
- Some college, but did not finish
- Two years college degree / Associate degree / A.A. / A.S.
- Four-year college degree / B.A. / B.S.
- Some graduate school
- Master's degree (MA / MS / MBA / MFA / MDiv)
- Advanced degree (PhD / MD / JD)

During your educational career, which of the following best describes your primary focus?

- Humanities
- Social Sciences
- Natural Sciences or Math
- Applied Science or Engineering
- None

How would you describe your knowledge of the Deferred Acceptance (DA) matching mechanism, also known as the Gale-Shapley mechanism?

- I have never heard of it
- I heard of it but I don't know/remember what it is
- I only vaguely know what it intends to do
- I know some details about the mechanism
- I am pretty familiar with it and understand reasonably well its principles and/or how it works
- I know it so well that I could easily explain its principles and/or how it works

Have you ever participated, or are you soon going to participate, in a real-life implementation of the Deferred Acceptance (or Gale-Shapley) mechanism?

- No
- Yes, I have
- Yes, I am going to

What is your current marital status?

- Married
- Widowed
- Separated
- Divorced
- Single
- Living with a significant other

Which of the following best describes your main activity or your employment status?

- Working
- Unemployed
- Retired
- Stay-at-home parent
- Student
- Other

In general, how do you consider your views on social issues?

- Very liberal
- Liberal
- Slightly liberal
- Moderate
- Slightly conservative
- Conservative
- Very conservative
- Other

In general, how do you consider your views on economic issues?

- Very liberal
- Liberal
- Slightly liberal
- Moderate
- Slightly conservative
- Conservative
- Very conservative
- Other

Do you consider yourself a...

- Republican
- Democrat
- Independent
- Other
- None of the above

For whom did you vote in the last presidential elections of 2020?

- Joe Biden
- Donald Trump
- Other candidate
- I did not vote

What is your combined annual household income?

- Less than \$20,000
- \$20,000 – \$39,999
- \$40,000 – \$59,999
- \$60,000 – \$79,999
- \$80,000 – \$99,999
- \$100,000 – \$149,999
- \$150,000 – \$199,999
- \$200,000 or more

Were the study instructions clear and simple to understand? Please briefly mention anything that was unclear. Please share with us any other comments about the study, we highly value any feedback!

Submit

## D.9.1 Exit Page (Cornell)

Thank you for participating in this study!

Your total earnings are as follows:

1. Your participation fee is **\$17.00**.
2. The earnings you accumulated in game rounds are **\$5.42**.
3. 72 out of 72 questions (100.0%) count for your Understanding Bonus. Hence, out of the full Understanding Bonus of \$4.50, you get **\$4.50**.

Well done! Your total earnings are **\$26.92**

Thank you!

## D.9.2 Exit Page (Prolific)

Thank you for participating in this study!

Your total earnings are as follows:

1. Your participation fee is **£7.00**.
2. The earnings you accumulated in game rounds are **£4.17**.
3. 72 out of 72 questions (100.0%) count for your Understanding Bonus. Hence, out of the full Understanding Bonus of £4.50, you get **£4.50**.

Well done! Your total earnings are **£15.67**

Your completion code is **C16U845Z**.

Thank you!

## D.10.1 General Reminder

×

In this study, you and three computerized participants, Ruth, Shirley, and Theresa, are going to play a game for four prizes.

Each prize is worth money, but might be worth a different amount of money for each participant.

You and the computerized participants will each rank the four prizes in any order you wish.

Then, an **allocation process** will use these rankings to allocate the prizes—one prize for each participant.

The allocation process attempts to give each participant a prize that they ranked higher rather than a prize that they ranked lower. However, this is not always possible, since the allocation process must take into account the rankings of all participants.

## D.10.2 Prizes Reminder

×

In Step 1, you first see the **prizes** you can get in this round and how much money they are worth to **you**. In the table, under each prize A, B, C or D, you can see how much money it would add to **your** earnings if **you get it**.

Each prize might be worth a **different** amount of money for each participant, and each participant can only see the money amounts relevant to **themselves**. However, the prizes that earn you a large amount of money are also likely to earn the **other participants** a large amount of money. There is more likely to be **competition** for the high-earning prizes.

The money worth of prizes for you and for the other participants can be different in different rounds of the game, and they were **determined beforehand**. You and the other participants **cannot affect the money worth of prizes**.

### D.10.3 Priorities Reminder

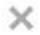

All four participants have some **priority** for getting each of the four prizes. These priorities can affect the allocation of prizes.

The higher your priority is for getting some prize, the more likely you generally are to get that prize at the end of the process.

Each column shows the priorities of all participants for getting some prize, written from highest to lowest.

The prize priorities can be different in different rounds of the game, and they were **determined beforehand**.

You and the other participants **cannot affect the prize priorities**.

#### D.10.4 Ranking Reminder

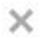

In Step 2, you are asked to **rank the four prizes** in an order of your choice.

The computerized participants simultaneously submit their own rankings. They **do not know** your own ranking.

Their rankings are aimed at getting them their high-earning prizes. Your own ranking **cannot affect the computerized participants' rankings**.

### D.10.5.1 Traditional DA Mechanics Description Reminder

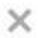

**These details are important to learn:** You may be able to apply your knowledge of them to make better decisions in the upcoming real rounds of this study.

Some details may seem confusing at first. This is quite natural! But don't worry, we will show you step-by-step examples. Things will become clearer along the way.

#### Overview of allocation process

The following image illustrates how your own ranking, the rankings of the other participants and the prize priorities affect the prize you get:

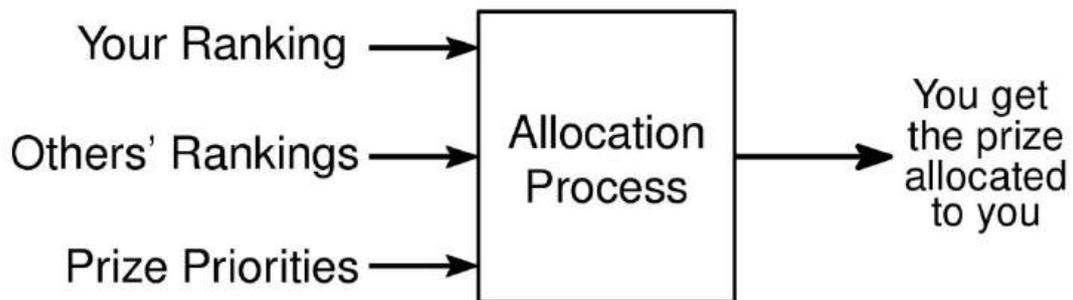

#### Details of allocation process

The allocation process is a multi-step process, as follows (it may look complicated, but don't worry, we will rehearse this in a moment):

1. In the first step, each participant is paired to their **highest**-rank prize.
2. In the next step, possible conflicts are detected and solved.  
If two (or more) participants are paired to the same prize, this is a **conflict**.

Each conflict is solved in two steps:

- **Unpair**: only the participant highest in that prize's priorities remains paired to that prize. The others get unpaired.
- **Re-pair**: all unpaired participants can only get re-paired to prizes that they were not paired with before. Each unpaired participant is re-paired to their **highest-rank** prize among the prizes they **were not yet paired with**.

3. Later steps continue in the same way, by detecting and solving new conflicts.  
Like before, if two (or more) participants are paired to the same prize, this is a **conflict**.  
The conflict is solved using the same **Unpair** and **Re-pair** steps from above.

A participant can get unpaired from a prize **even if they successfully got paired to that prize in a previous step**.

When there are no more conflicts, the process is over. The result is each participant being paired to a different prize.

Each prize is then allocated to the participant paired to it.

## D.10.5.2 Menu DA Mechanics Description Reminder

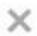

**These details are important to learn:** You may be able to apply your knowledge of them to make better decisions in the upcoming real rounds of this study. Some details may seem confusing at first. This is quite natural! But don't worry, we will show you step-by-step examples. Things will become clearer along the way.

### Overview of allocation process

The prize you get is determined using an allocation process with two main steps:

1. The computer determines some group of **Obtainable Prizes** that you might receive. Your own ranking does not influence the Obtainable Prizes. Instead, they are determined using only the prize priorities and the rankings of the other participants.
2. You get the Obtainable Prize that you **ranked highest** (in the ranking you submitted).

**The important principle:** Your own ranking does **not** influence what the Obtainable Prizes are, but it **does** determine what you get from among the Obtainable Prizes—you get the Obtainable Prize that you ranked the **highest**.

The following image illustrates how your own ranking, the rankings of the other participants and the prize priorities affect the prize you get:

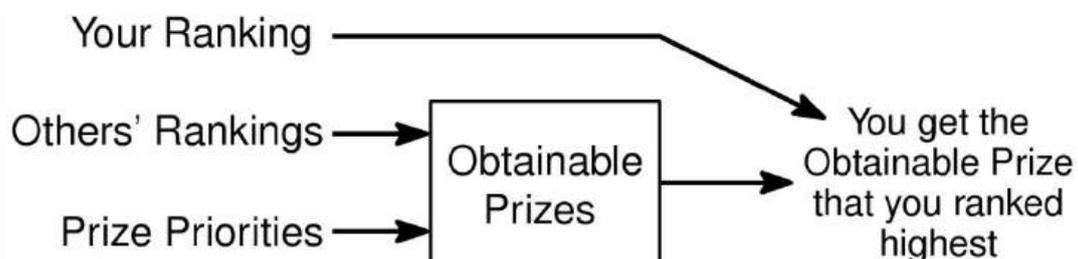

### Details of allocation process

#### Priorities and rankings → Temporary allocation → Obtainable Prizes

The allocation process begins with a multi-step process. This process determines a “temporary allocation” of prizes to all participants **except for you**, and then determines your Obtainable Prizes based on this temporary allocation. This process **does not involve your own submitted ranking**, and works as follows (it may look complicated, but don't worry, we will rehearse this in a moment):

1. In the first step, each prize is paired to its **highest**-priority participant, among all participants **except for you**.
2. In the next step, possible conflicts are detected and solved.  
If two (or more) prizes are paired to the same participant, this is a **conflict**.

Each conflict is solved in two steps:

- **Unpair:** only the prize highest in that participant's ranking remains paired to that participant. The others get unpaired.
- **Re-pair:** all unpaired prizes can only get re-paired to participants that they were not paired with before, and who are not you. Each unpaired prize is re-paired to its **highest**-priority participant, among the participants they **were not yet paired with** and **except for you**.

3. Later steps continue in the same way, by detecting and solving new conflicts. Like before, if two (or more) prizes are paired to the same participant, this is a **conflict**. The conflict is solved using the same **Unpair** and **Re-pair** steps from above.

A prize can get unpaired from a participant **even if it successfully got paired to that participant in a previous step**.

There is one **important thing to note about** the Re-pair step:

During the process, one prize will encounter a conflict with **every** participant, except for you, and will eventually get unpaired from all of them. That prize cannot be re-paired and will **remain unpaired** at the end of the process.

When there are no more conflicts and when one prize was unpaired from all participants (except for you), the process is over. The result is each prize, except for the unpaired one, being paired to a different participant (except for you).

Each prize except for the unpaired one is then **temporarily allocated** to the participant it is paired to.

The other participants do not get their prize from the temporary allocation; their prizes are determined by some other process.

Instead, the temporary allocation is used to determine your Obtainable Prizes.

Next, we will tell you how the **Obtainable Prizes** are determined from the temporary allocation.

In this temporary allocation, no prize was allocated to you. To determine which prize is allocated to you, the computer first determines which prizes you can obtain in principle. These are the **Obtainable Prizes**.

You can obtain two kinds of prizes:

1. Any prize for which **your priority is higher** than that of the participant it is temporarily allocated to.
2. **The prize that was left unpaired in the temporary allocation.**

You cannot obtain any other prizes.

### **Obtainable Prizes → The prize you get**

Finally, we will remind you how the prize you get is selected from among the Obtainable Prizes, using your ranking.

In fact, this is the **only** time the allocation process uses your ranking.

From among the Obtainable Prizes, **you get the one that you ranked the highest**.

In other words, the computer will look through your ranking from top to bottom, and you will get the first prize that is Obtainable.

### D.10.5.3 Menu SP Property Description Reminder

**This principle is important to learn:** You may be able to apply your knowledge of it to choose your rankings in the upcoming real rounds of this study.

The prize you get is determined using an allocation process with two main steps:

1. The computer determines some group of **Obtainable Prizes** that you might receive. Your own ranking does not influence the Obtainable Prizes. Instead, they are determined using only the prize priorities and the rankings of the other participants.
2. You get the Obtainable Prize that you **ranked highest** (in the ranking you submitted).

**The important principle:** Your own ranking does **not** influence what the Obtainable Prizes are, but it **does** determine what you get from among the Obtainable Prizes—you get the Obtainable Prize that you ranked the **highest**.

The following image illustrates how your own ranking, the rankings of the other participants and the prize priorities affect the prize you get:

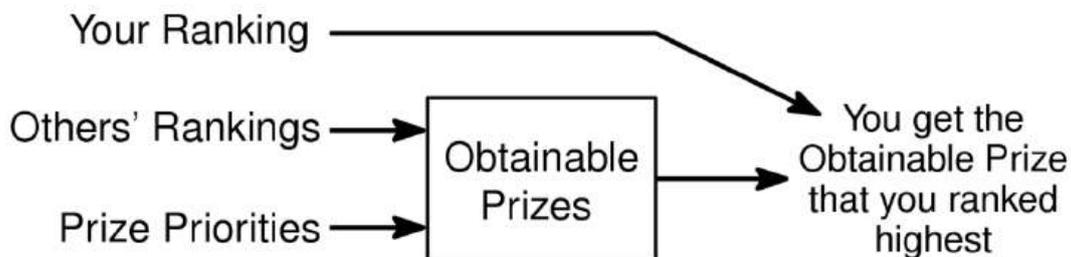

For example, imagine that your Obtainable Prizes are C and D. If you submit the ranking A–B–C–D, you will get Prize C, which is the one you ranked highest among the Obtainable Prizes. No ranking you could possibly submit would get you Prize A or Prize B, since the Obtainable Prizes are C and D, and since your own ranking cannot influence the Obtainable Prizes.

#### D.10.5.4 Textbook SP Property Description Reminder

×

**This principle is important to learn:** You may be able to apply your knowledge of it to choose your rankings in the upcoming real rounds of this study.

The prize you get is determined using an **allocation process** that uses your own ranking, the rankings of the other participants, and the prize priorities.

The following image illustrates this:

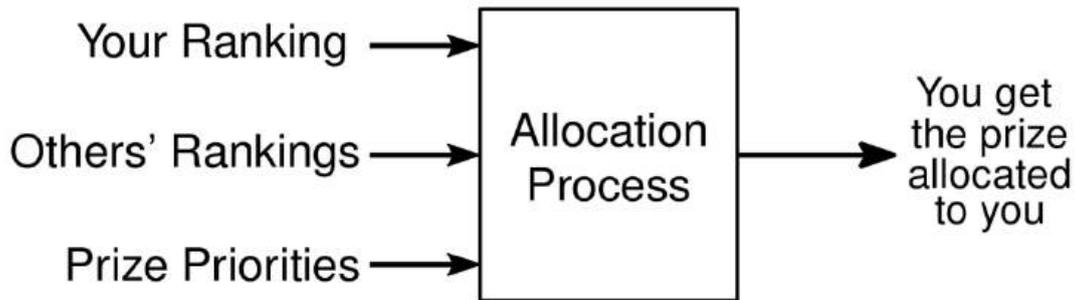

Now, imagine that the computer already determined some prize priorities and rankings of the other, computerized participants. The only component left undecided is your own ranking.

Now, as you decide which ranking to submit, imagine there is some specific ranking that you are considering submitting. Let's call it "the considered ranking".

**The important principle:** The prize you get if you submit the considered ranking is the **highest** that submitting any ranking could get you, **according to the considered ranking**.

In other words, if you submit any alternative ranking, different from the considered ranking, you will either get **the same** prize you get when submitting the considered ranking, or some prize **lower on the considered ranking**.

No alternative ranking can get you a prize which you rank higher on the considered ranking, compared to the prize you get when you submit the considered ranking.

For example, imagine that you submitted the ranking A–B–C–D and ended up getting Prize C. This means that Prize C is the highest possible that you could get on the considered ranking A–B–C–D. Submitting any other, alternative ranking different from A–B–C–D could have only gotten you the same prize, Prize C, or possibly a lower-ranked prize on the considered ranking, Prize D. No other alternative ranking could have gotten you Prize A or Prize B.

### D.11.1 Messages Following Correct and Incorrect Responses: All Questions Except for DA Mechanics Allocation-Calculation GUI

\* The messages below are shown for an example training question, but are presented identically in all training questions (except for the feedback relevant to the content of the specific question).

#### D.11.1.1 Correct answer on first attempt

Please determine whether the following statement is true or false:

If I rank some prize very **low** and get it, I may earn **less** than its money worth, shown in the table above. If I rank some prize very **high** and get it, I may earn **more** than its money worth.

(Get it right on first try to increase your bonus)

- True  
 False

Correct! Your own ranking cannot affect the money worth of prizes shown in your table, which are determined beforehand.

Good job on the first try! This will count for your Understanding Bonus.

#### D.11.1.2 Correct answer on second or later attempt

Please determine whether the following statement is true or false:

If I rank some prize very **low** and get it, I may earn **less** than its money worth, shown in the table above. If I rank some prize very **high** and get it, I may earn **more** than its money worth.

(Get it right on first try to increase your bonus)

- True  
 False

Correct! Your own ranking cannot affect the money worth of prizes shown in your table, which are determined beforehand.

#### D.11.1.3 Incorrect answer

Please determine whether the following statement is true or false:

If I rank some prize very **low** and get it, I may earn **less** than its money worth, shown in the table above. If I rank some prize very **high** and get it, I may earn **more** than its money worth.

(Get it right on first try to increase your bonus)

- True  
 False

Incorrect answer. Please try again.

## D.11.2 Messages Following Correct and Incorrect Responses: DA Mechanics Allocation-Calculation GUI

\* The messages below are shown for an example allocation-calculation step in Trad-DA training round 1, but are presented identically in both Trad-DA and Menu-DA in all other calculation steps in that round.

### D.11.2.1 Correct answer on first attempt: round 1

## How the Allocation Process Works: Training Round 1/3

Click for a reminder on the technical details of the allocation process

First, pair Ruth to her **highest-rank** prize. To do this:

1. Start from the "Pick participants to pair" row, and click on **Ruth ("R")**.
2. Then, in the list of four prizes at the bottom left part of the dashboard, click on "+" next to the prize that is **highest in Ruth's ranking**.

Hint: the prize that is highest in Ruth's ranking is indicated by the letter just under "R" in the Participant Rankings table.

After pairing, "A" and "R" will be colored purple in the two tables, to indicate that they are paired.

Only pair **Ruth ("R")!** You will pair the other participants in the next step.

Click Submit when done.

(Get it right on first try to increase your bonus)

Correct!

Good job on the first try! This will count for your Understanding Bonus.

Proceed

### Prize Priorities:

| A | B | C | D |
|---|---|---|---|
| R | R | S | Y |
| S | S | T | T |
| T | Y | R | S |
| Y | T | Y | R |

### Participant Rankings:

reset ↻

| R | S | T | Y |
|---|---|---|---|
| A | A | B | C |
| C | C | A | A |
| D | D | D | B |
| B | B | C | D |

---

### Pick participants to pair →

S

T

Y

---

**A**

**B**

**C**

**D**

R

R = Ruth

S = Shirley

T = Theresa

Y = You

### D.11.2.2 Correct answer on second and third attempts: round 1

## How the Allocation Process Works: Training Round 1/3

Click for a reminder on the technical details of the allocation process

First, pair Ruth to her **highest-rank** prize. To do this:

1. Start from the "Pick participants to pair" row, and click on **Ruth ("R")**.
2. Then, in the list of four prizes at the bottom left part of the dashboard, click on "+" next to the prize that is **highest in Ruth's ranking**.

Hint: the prize that is highest in Ruth's ranking is indicated by the letter just under "R" in the Participant Rankings table.

After pairing, "A" and "R" will be colored purple in the two tables, to indicate that they are paired.

Only pair **Ruth ("R")!** You will pair the other participants in the next step.

Click Submit when done.

(Get it right on first try to increase your bonus)

Correct!

Proceed

| Prize Priorities: |   |   |   | Participant Rankings: |   |   |   | reset ↻ |
|-------------------|---|---|---|-----------------------|---|---|---|---------|
| A                 | B | C | D | R                     | S | T | Y |         |
| R                 | R | S | Y | A                     | A | B | C |         |
| S                 | S | T | T | C                     | C | A | A |         |
| T                 | Y | R | S | D                     | D | D | B |         |
| Y                 | T | Y | R | B                     | B | C | D |         |

Pick participants to pair → S T Y

|   |                                |                                                   |
|---|--------------------------------|---------------------------------------------------|
| A | <input type="text" value="R"/> | R = Ruth<br>S = Shirley<br>T = Theresa<br>Y = You |
| B | <input type="text"/>           |                                                   |
| C | <input type="text"/>           |                                                   |
| D | <input type="text"/>           |                                                   |

Allocation Dashboard

### D.11.2.3 Incorrect answer on first and second attempts: round 1

## How the Allocation Process Works: Training Round 1/3

Click for a reminder on the technical details of the allocation process

First, pair Ruth to her **highest-rank** prize. To do this:

1. Start from the "Pick participants to pair" row, and click on **Ruth ("R")**.
2. Then, in the list of four prizes at the bottom left part of the dashboard, click on "+" next to the prize that is **highest in Ruth's ranking**.

Hint: the prize that is highest in Ruth's ranking is indicated by the letter just under "R" in the Participant Rankings table.

After pairing, "A" and "R" will be colored purple in the two tables, to indicate that they are paired.

Only pair **Ruth ("R")!** You will pair the other participants in the next step.

Click Submit when done.

(Get it right on first try to increase your bonus)

Submit

Incorrect answer. Please try again.

| Prize Priorities: |   |   |   | Participant Rankings: |   |   |   | reset ↻ |
|-------------------|---|---|---|-----------------------|---|---|---|---------|
| A                 | B | C | D | R                     | S | T | Y |         |
| R                 | R | S | Y | A                     | A | B | C |         |
| S                 | S | T | T | C                     | C | A | A |         |
| T                 | Y | R | S | D                     | D | D | B |         |
| Y                 | T | Y | R | B                     | B | C | D |         |

Pick participants to pair → S T Y

|   |                                |                                                   |
|---|--------------------------------|---------------------------------------------------|
| A | <input type="text"/>           | R = Ruth<br>S = Shirley<br>T = Theresa<br>Y = You |
| B | <input type="text" value="R"/> |                                                   |
| C | <input type="text"/>           |                                                   |
| D | <input type="text"/>           |                                                   |

Allocation Dashboard

### D.11.2.4 Incorrect answer on third attempt: round 1

## How the Allocation Process Works: Training Round 1/3

Click for a reminder on the technical details of the allocation process

First, pair Ruth to her **highest-rank** prize. To do this:

1. Start from the "Pick participants to pair" row, and click on **Ruth ("R")**.
2. Then, in the list of four prizes at the bottom left part of the dashboard, click on "+" next to the prize that is **highest in Ruth's ranking**.

Hint: the prize that is highest in Ruth's ranking is indicated by the letter just under "R" in the Participant Rankings table.

After pairing, "A" and "R" will be colored purple in the two tables, to indicate that they are paired.

Only pair **Ruth ("R")!** You will pair the other participants in the next step.

Click Submit when done.

(Get it right on first try to increase your bonus)

**Incorrect answer. We set the dashboard correctly for you this time. Please make sure you understand your mistake.**

Proceed

| Prize Priorities: |          |          |          | Participant Rankings: |          |          |          | reset ↻ |
|-------------------|----------|----------|----------|-----------------------|----------|----------|----------|---------|
| <b>A</b>          | <b>B</b> | <b>C</b> | <b>D</b> | <b>R</b>              | <b>S</b> | <b>T</b> | <b>Y</b> |         |
| <b>R</b>          | R        | S        | Y        | <b>A</b>              | A        | B        | C        |         |
| S                 | S        | T        | T        | C                     | C        | A        | A        |         |
| T                 | Y        | R        | S        | D                     | D        | D        | B        |         |
| Y                 | T        | Y        | R        | B                     | B        | C        | D        |         |

Pick participants to pair → **S** **T** **Y**

|          |          |                                                                               |
|----------|----------|-------------------------------------------------------------------------------|
| <b>A</b> | <b>R</b> | <b>R</b> = Ruth<br><b>S</b> = Shirley<br><b>T</b> = Theresa<br><b>Y</b> = You |
| <b>B</b> |          |                                                                               |
| <b>C</b> |          |                                                                               |
| <b>D</b> |          |                                                                               |

Allocation Dashboard

\* The messages below are shown for an example allocation-calculation problem in Trad-DA training round 2, but are presented identically in both Trad-DA and Menu-DA in both calculation problems of rounds 2 and 3.

### D.11.2.5 Correct answer on first attempt: rounds 2 and 3

## How the Allocation Process Works: Training Round 2/3

[Click for a reminder on the technical details of the allocation process](#)

Find the **allocation** of prizes to participants using the Allocation Dashboard below. Use the multi-step process you learned.

**Note:** In this round, you should only submit once you find the **final allocation**. Do **not** separately submit steps of the process like in Training Round 1.

In case you are still not sure how to find the allocation by yourself, click on the button below to watch a helpful video explaining all the steps. Clicking on the video will pause/unpause it, and if you close and re-open the video, it will continue from the same point.

[Click here for a video with step-by-step explanations](#)

(To restart the video, please refresh the page)

Click Submit when you are done.

(Get it right on first try to increase your bonus; it will count as **5 questions**.)

If you only get it right on the second try it will still count for your bonus; it will count as **2 questions**.)

Correct allocation!

Good job on the first try! This will count as **5 questions** for your Understanding Bonus.

[Proceed](#)

### Prize Priorities:

|   |   |   |   |
|---|---|---|---|
| A | B | C | D |
| S | S | T | T |
| Y | T | Y | R |
| R | Y | R | Y |
| T | R | S | S |

### Participant Rankings:

[reset](#) ↻

|   |   |   |   |
|---|---|---|---|
| R | S | T | Y |
| D | B | B | D |
| A | A | C | C |
| B | C | D | B |
| C | D | A | A |

---

**Pick participants to pair** →

|   |   |
|---|---|
| A | Y |
| B | S |
| C | T |
| D | R |

R = Ruth

S = Shirley

T = Theresa

Y = You

Allocation Dashboard

### D.11.2.6 Correct answer on second attempt: rounds 2 and 3

## How the Allocation Process Works: Training Round 2/3

Click for a reminder on the technical details of the allocation process

Find the **allocation** of prizes to participants using the Allocation Dashboard below. Use the multi-step process you learned.

**Note:** In this round, you should only submit once you find the **final allocation**. Do **not** separately submit steps of the process like in Training Round 1.

In case you are still not sure how to find the allocation by yourself, click on the button below to watch a helpful video explaining all the steps. Clicking on the video will pause/unpause it, and if you close and re-open the video, it will continue from the same point.

Click here for a video with step-by-step explanations

(To restart the video, please refresh the page)

Click Submit when you are done.

(Get it right on first try to increase your bonus; it will count as **5 questions**.)

If you only get it right on the second try it will still count for your bonus; it will count as **2 questions**.)

Correct allocation!

Good job on the second try! This will count as **2 questions** for your Understanding Bonus.

Proceed

| Prize Priorities: |   |   |   | Participant Rankings: |   |   |   | reset ↻ |
|-------------------|---|---|---|-----------------------|---|---|---|---------|
| A                 | B | C | D | R                     | S | T | Y |         |
| S                 | S | T | T | D                     | B | B | D |         |
| Y                 | T | Y | R | A                     | A | C | C |         |
| R                 | Y | R | Y | B                     | C | D | B |         |
| T                 | R | S | S | C                     | D | A | A |         |

**Pick participants to pair →**

|   |                                |                                                   |
|---|--------------------------------|---------------------------------------------------|
| A | <input type="text" value="Y"/> | R = Ruth<br>S = Shirley<br>T = Theresa<br>Y = You |
| B | <input type="text" value="S"/> |                                                   |
| C | <input type="text" value="T"/> |                                                   |
| D | <input type="text" value="R"/> |                                                   |

Allocation Dashboard

### D.11.2.7 Correct answer on third attempt: rounds 2 and 3

## How the Allocation Process Works: Training Round 2/3

Click for a reminder on the technical details of the allocation process

Find the **allocation** of prizes to participants using the Allocation Dashboard below. Use the multi-step process you learned.

**Note:** In this round, you should only submit once you find the **final allocation**. Do **not** separately submit steps of the process like in Training Round 1.

In case you are still not sure how to find the allocation by yourself, click on the button below to watch a helpful video explaining all the steps. Clicking on the video will pause/unpause it, and if you close and re-open the video, it will continue from the same point.

Click here for a video with step-by-step explanations

(To restart the video, please refresh the page)

Click Submit when you are done.

(Get it right on first try to increase your bonus; it will count as **5 questions**.)

If you only get it right on the second try it will still count for your bonus; it will count as **2 questions**.)

Correct allocation!

Proceed

| Prize Priorities: |   |   |   | Participant Rankings: |   |   |   | reset ↻ |
|-------------------|---|---|---|-----------------------|---|---|---|---------|
| A                 | B | C | D | R                     | S | T | Y |         |
| S                 | S | T | T | D                     | B | B | D |         |
| Y                 | T | Y | R | A                     | A | C | C |         |
| R                 | Y | R | Y | B                     | C | D | B |         |
| T                 | R | S | S | C                     | D | A | A |         |

**Pick participants to pair →**

|   |                                |                                                   |
|---|--------------------------------|---------------------------------------------------|
| A | <input type="text" value="Y"/> | R = Ruth<br>S = Shirley<br>T = Theresa<br>Y = You |
| B | <input type="text" value="S"/> |                                                   |
| C | <input type="text" value="T"/> |                                                   |
| D | <input type="text" value="R"/> |                                                   |

Allocation Dashboard

### D.11.2.8 Incorrect answer on first and second attempts: rounds 2 and 3

## How the Allocation Process Works: Training Round 2/3

Click for a reminder on the technical details of the allocation process

Find the **allocation** of prizes to participants using the Allocation Dashboard below. Use the multi-step process you learned.

**Note:** In this round, you should only submit once you find the **final allocation**. Do **not** separately submit steps of the process like in Training Round 1.

In case you are still not sure how to find the allocation by yourself, click on the button below to watch a helpful video explaining all the steps. Clicking on the video will pause/unpause it, and if you close and re-open the video, it will continue from the same point.

Click here for a video with step-by-step explanations

(To restart the video, please refresh the page)

Click Submit when you are done.

(Get it right on first try to increase your bonus; it will count as **5 questions**.)

If you only get it right on the second try it will still count for your bonus; it will count as **2 questions**.)

Submit

Incorrect allocation. Please try again.

| Prize Priorities: |   |   |   | Participant Rankings: |   |   |   | reset ↻ |
|-------------------|---|---|---|-----------------------|---|---|---|---------|
| A                 | B | C | D | R                     | S | T | Y |         |
| S                 | S | T | T | D                     | B | B | D |         |
| Y                 | T | Y | R | A                     | A | C | C |         |
| R                 | Y | R | Y | B                     | C | D | B |         |
| T                 | R | S | S | C                     | D | A | A |         |

**Pick participants to pair →**

|   |                                |                                                   |
|---|--------------------------------|---------------------------------------------------|
| A | <input type="text" value="R"/> | R = Ruth<br>S = Shirley<br>T = Theresa<br>Y = You |
| B | <input type="text" value="S"/> |                                                   |
| C | <input type="text" value="T"/> |                                                   |
| D | <input type="text" value="Y"/> |                                                   |

Allocation Dashboard

### D.11.2.9 Incorrect answer on third attempt: rounds 2 and 3

## How the Allocation Process Works: Training Round 2/3

Click for a reminder on the technical details of the allocation process

Find the **allocation** of prizes to participants using the Allocation Dashboard below. Use the multi-step process you learned.

Note: In this round, you should only submit once you find the **final allocation**. Do **not** separately submit steps of the process like in Training Round 1.

In case you are still not sure how to find the allocation by yourself, click on the button below to watch a helpful video explaining all the steps. Clicking on the video will pause/unpause it, and if you close and re-open the video, it will continue from the same point.

Click here for a video with step-by-step explanations

(To restart the video, please refresh the page)

Click Submit when you are done.

(Get it right on first try to increase your bonus; it will count as **5 questions**.)

If you only get it right on the second try it will still count for your bonus; it will count as **2 questions**.)

Incorrect allocation.

We set the dashboard correctly for you this time. Please make sure you understand your mistake.

Proceed

| Prize Priorities: |   |   |   | Participant Rankings: |   |   |   | reset ↻ |
|-------------------|---|---|---|-----------------------|---|---|---|---------|
| A                 | B | C | D | R                     | S | T | Y |         |
| S                 | S | T | T | D                     | B | B | D |         |
| Y                 | T | Y | R | A                     | A | C | C |         |
| R                 | Y | R | Y | B                     | C | D | B |         |
| T                 | R | S | S | C                     | D | A | A |         |

**Pick participants to pair →**

|   |                                |                                                   |
|---|--------------------------------|---------------------------------------------------|
| A | <input type="text" value="Y"/> | R = Ruth<br>S = Shirley<br>T = Theresa<br>Y = You |
| B | <input type="text" value="S"/> |                                                   |
| C | <input type="text" value="T"/> |                                                   |
| D | <input type="text" value="R"/> |                                                   |

Allocation Dashboard
